# Supplementary material for: A corresponding-state framework for the structural transition of supercritical fluids across the Widom delta
Source: arXiv:1812.09453 source file (2019-04-23)
Supplement: Supplementary file 1 [file Supplementary_material_for__A_corresponding_state_framework.pdf]

# Supplementary material for "A corresponding-state framework for the structural transition of supercritical fluids across the Widom delta"

Tae Jun Yoon,[1] Min Young Ha,[1] Won Bo Lee,[1, a)] and Youn-Woo Lee[1, b)]
*School of Chemical and Biological Engineering, Institute of Chemical Processes, Seoul National University, Seoul 08826, Republic of Korea*

In this supplementary material, we provide the numerical data that can help understand and reproduce the results in the main article. It includes the algorithm validation result; pressure data of near-critical fluids used for the estimation of the critical point; the fractions of gas-like molecules; the probabilities of finding an infinite droplet (bubble); the percolation transition densities (pressures); the number of independent gas-like bubbles and liquid-like droplets in $N = 1,000$ systems; and the finite-size scaling data.

## ALGORITHM VALIDATION

To validate the algorithm, we perform the NVT simulations of the Lennard-Jones (LJ) fluid ($\sigma = 1.0$ and $\epsilon = 1.0$). For the NVT simulations of the LJ fluid, the number of particles is 2,000. The interatomic potential is truncated at $r_{cut} = 3.0\sigma$ and the tail correction term is added. Table s1 shows the $\rho$-T-p relation of the LJ fluid. All simulation data for the LJ fluid are dimensionless, and the pressure data is collected every step during the production run (1,000,000 steps). A cubic equation is used to fit the pressure data at constant temperature.

$$p = a\rho^3 + b\rho^2 + c\rho + d \tag{1}$$

where $a$, $b$, $c$, and $d$ are fitting parameters. The inflection density is thus defined as $\rho_{inflection} = -b/3a$. By fitting a linear equation to the inflection densities at different temperatures, we obtain the critical point. The critical point of the LJ fluid is obtained as $T_c* = 1.3425$, $p_c* = 0.1411$, and $\rho_c* = 0.3054$.

TABLE s1. ρ-T-p relation for near-critical LJ fluid

| $\rho\sigma^3$ | T*=1.330 | T*=1.335 | T*=1.340 | T*=1.345 |
|---|---|---|---|---|
| 0.24 | 0.1348 | 0.1369 | 0.1387 | 0.1405 |
| 0.26 | 0.1353 | 0.1376 | 0.1398 | 0.1421 |
| 0.28 | 0.1355 | 0.1377 | 0.1401 | 0.1425 |
| 0.30 | 0.1351 | 0.1376 | 0.1402 | 0.1432 |
| 0.32 | 0.1346 | 0.1369 | 0.1402 | 0.1430 |
| 0.34 | 0.1339 | 0.1367 | 0.1400 | 0.1433 |
| 0.36 | 0.1333 | 0.1366 | 0.1406 | 0.1444 |
| 0.38 | 0.1342 | 0.1374 | 0.1421 | 0.1455 |

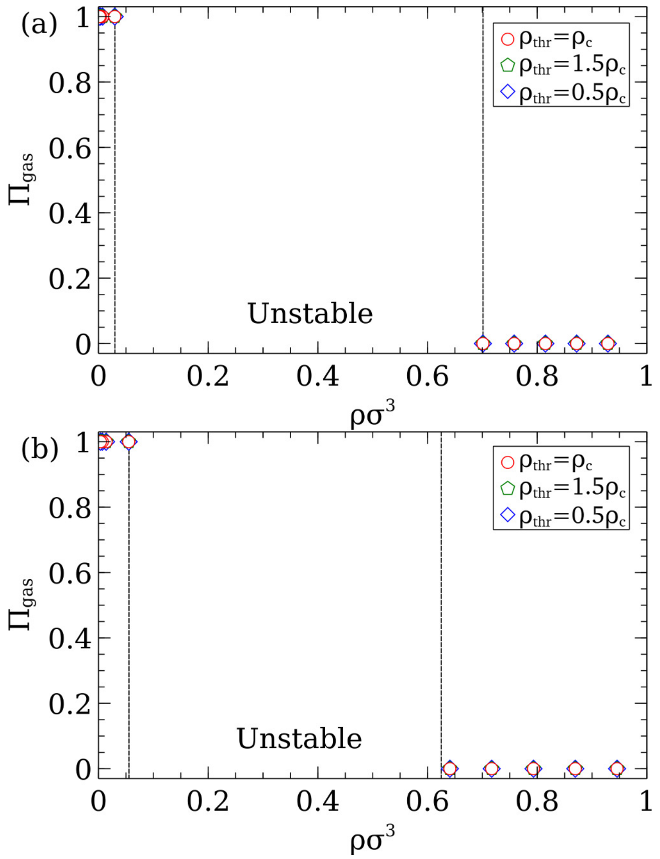


FIG. s1. Classification results at $T* = 1.00$ and $T* = 1.10$. Regardless of the choice of the density criterion, the classification results agree with each other. For subcritical vapor, the fraction of gas-like molecules ($\Pi_{gas}$) is always one. For subcritical liquid, $\Pi_{gas}$ is zero. The dotted lines denote the saturation densities.

After the estimation of the critical point, we perform the NVT simulations of subcritical LJ fluids ($T* = 1.00 - 1.30$). The systems are equilibrated for 100,000 steps and three hundred snapshots are collected every 10,000 steps during the production run. The simulation densities of vapor and liquid phases are determined based on the NIST reference simulation data[1] generated from the empirical fitting equation proposed by Johnson and his coworkers[2]. We apply the weighted mean-field classification strategy to the obtained data. In this procedure, we use different densities ($\rho_{thr} = 0.5\rho_c*, 1.0\rho_c*$ and $1.5\rho_c*$) to validate that the critical density should be used to classify a molecule into gas-like or liquid-like in the critical region. Figs. s1 and s2 compare the classi-

a) Electronic mail: wblee@snu.ac.kr
b) Electronic mail: ywlee@snu.ac.kr

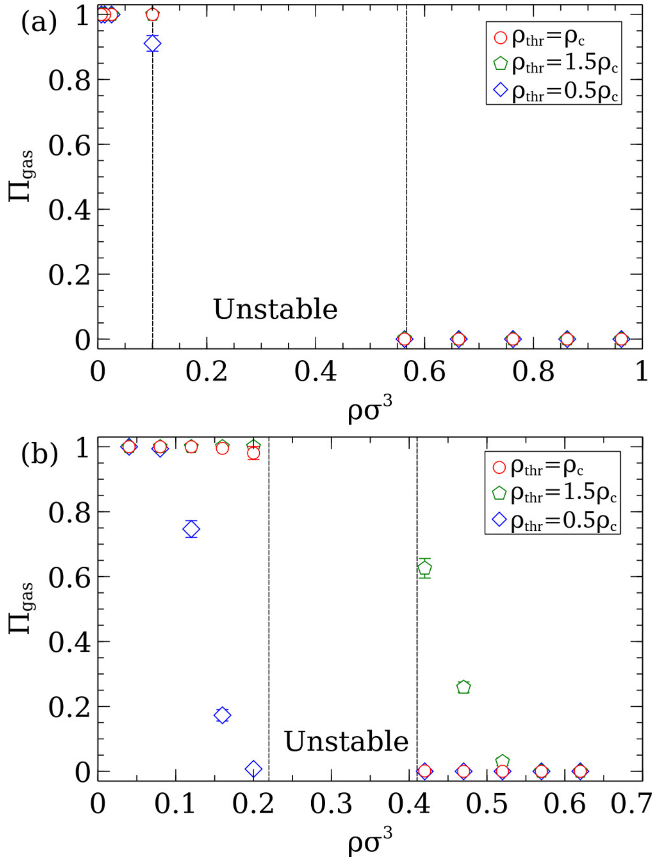


FIG. s2. Classification results at $T* = 1.20$ and $T* = 1.30$. As the simulation temperature approaches the critical temperature, the classification results start to disagree with each other. At $T* = 1.20$, the gas-like fraction of saturated vapor deviates from one when $\rho_{thr} = 0.5\rho_c$ is used. At $T* = 1.30$, both $\rho_{thr} = 0.5\rho_c$ and $\rho_{thr} = 1.5\rho_c$ criteria yield unacceptable classification results taking into account that the subcritical saturated vapor ($\Pi_{gas} = 1.0$) and liquid ($\Pi_{gas} = 0.0$) systems should be clearly distinct from each other. The dotted lines denote the saturation densities.

fication results obtained when different density criterion is used. Far from the critical temperature (s1a and b), the classification results among different criteria are not significantly different from each other. For subcritical vapor, the fraction of gas-like molecules ($\Pi_{gas}$) is always unity. It becomes zero for subcritical liquid. However, as seen in Fig. s2a and b, the classification results become different from each other near the critical temperature. When $\rho_{thr} = 1.5\rho_c*$ is used, subcritical liquids near the saturation densities at $T* = 1.20$ and 1.30 have a considerable amount of gas-like molecules. On the other hand, when a lower density criterion ($\rho_{thr} = 0.5\rho_c$) is used, the fractions of gas-like molecules in the subcritical vapor systems are far below unity near the critical temperature. Taking into account that the subcritical vapor ($\Pi_{gas} = 1.0$) and liquid ($\Pi_{gas} = 0.0$) should be clearly distinct from each other, the classification result based on the density criterion of $\rho_{thr} = \rho_c$ is adequate. Hence, this result justifies our use of the critical density for the classification of molecules in the supercritical state.

## ESTIMATION OF THE CRITICAL POINT

We use the same procedure to obtain the critical points of various substances. Tables s2-s11 contain the ρ-T-p

TABLE s2. ρ-T-p relation for near-critical argon

| ρ [kg/m$^3$] | 150 K | 155 K | 160 K | 165 K | 170 K |
|---|---|---|---|---|---|
| 150 | 33.048 | 35.029 | 37.003 | 38.910 | 40.894 |
| 250 | 42.195 | 45.865 | 49.690 | 53.274 | 57.026 |
| 350 | 44.041 | 49.958 | 55.825 | 61.687 | 67.077 |
| 450 | 42.009 | 49.949 | 58.375 | 65.611 | 73.714 |
| 550 | 38.203 | 48.255 | 58.438 | 68.845 | 79.407 |
| 650 | 32.147 | 46.027 | 59.504 | 73.214 | 87.099 |
| 750 | 30.814 | 47.704 | 65.889 | 83.557 | 101.730 |
| 850 | 38.656 | 61.310 | 83.677 | 108.356 | 132.295 |
| 950 | 69.584 | 100.289 | 132.381 | 162.976 | 193.574 |

TABLE s3. ρ-T-p relation for near-critical methane

| ρ [kg/m$^3$] | 185 K | 190 K | 195 K | 200 K | 205 K |
|---|---|---|---|---|---|
| 50 | 32.609 | 34.270 | 35.989 | 37.630 | 39.337 |
| 90 | 40.958 | 44.472 | 48.090 | 51.676 | 55.033 |
| 130 | 40.221 | 45.763 | 51.495 | 56.873 | 62.499 |
| 150 | 37.840 | 44.434 | 51.215 | 57.718 | 64.533 |
| 160 | 36.544 | 43.532 | 51.116 | 58.406 | 65.750 |
| 170 | 34.764 | 42.507 | 50.753 | 58.519 | 66.475 |
| 190 | 31.794 | 41.073 | 50.258 | 60.164 | 69.595 |
| 230 | 27.751 | 41.691 | 54.725 | 68.563 | 82.266 |
| 270 | 41.142 | 60.595 | 80.383 | 100.086 | 120.298 |

TABLE s4. ρ-T-p relation for near-critical ethylene oxide

| ρ [kg/m$^3$] | 460 K | 470 K | 475 K | 480 K | 490 K |
|---|---|---|---|---|---|
| 50 | 35.796 | 36.956 | 37.614 | 38.138 | 39.352 |
| 150 | 72.673 | 77.522 | 79.904 | 81.739 | 86.345 |
| 250 | 84.555 | 92.585 | 96.962 | 100.518 | 108.583 |
| 300 | 86.103 | 96.339 | 101.332 | 106.074 | 116.357 |
| 350 | 85.325 | 97.113 | 103.311 | 108.631 | 120.857 |
| 400 | 83.038 | 98.487 | 101.295 | 112.315 | 127.229 |
| 450 | 82.483 | 98.440 | 107.048 | 116.266 | 133.392 |
| 550 | 83.394 | 106.720 | 119.267 | 132.651 | 154.104 |
| 650 | 111.817 | 146.721 | 164.718 | 181.362 | 218.343 |

TABLE s5. ρ-T-p relation for near-critical ammonia

| ρ [kg/m$^3$] | 395 K | 405 K | 415 K | 425 K | 435 K |
|---|---|---|---|---|---|
| 50 | 67.889 | 71.445 | 74.785 | 78.179 | 81.466 |
| 100 | 96.490 | 104.589 | 112.458 | 120.307 | 128.065 |
| 150 | 102.942 | 115.890 | 128.891 | 141.898 | 154.494 |
| 200 | 99.602 | 117.843 | 135.811 | 153.697 | 172.057 |
| 250 | 91.013 | 114.011 | 138.857 | 162.079 | 186.506 |
| 300 | 82.269 | 112.411 | 144.528 | 175.685 | 208.452 |
| 350 | 81.809 | 122.594 | 165.712 | 208.243 | 251.260 |
| 400 | 113.415 | 168.366 | 224.740 | 284.680 | 340.110 |

TABLE s6. ρ-T-p relation for near-critical oxygen

| ρ [kg/m$^3$] | 145 K | 150 K | 155 K | 160 K | 165 K |
|---|---|---|---|---|---|
| 150 | 35.423 | 38.005 | 40.654 | 43.335 | 45.946 |
| 200 | 39.124 | 43.132 | 47.213 | 50.905 | 54.620 |
| 250 | 40.198 | 45.520 | 51.221 | 55.917 | 61.052 |
| 300 | 39.772 | 46.333 | 52.865 | 59.190 | 65.715 |
| 350 | 38.000 | 45.457 | 53.575 | 61.247 | 69.335 |
| 400 | 35.093 | 44.138 | 53.403 | 62.680 | 71.713 |
| 450 | 32.111 | 42.280 | 52.748 | 63.680 | 74.614 |
| 500 | 27.871 | 39.873 | 52.269 | 65.749 | 78.050 |
| 550 | 23.386 | 37.712 | 52.709 | 68.248 | 83.429 |
| 600 | 20.122 | 37.082 | 54.292 | 73.007 | 91.459 |
| 650 | 18.213 | 39.977 | 61.775 | 83.058 | 104.825 |
| 700 | 23.225 | 48.170 | 72.229 | 99.984 | 126.311 |

TABLE s7. ρ-T-p relation for near-critical ethane

| ρ [kg/m$^3$] | 295 K | 300 K | 305 K | 310 K | 315 K |
|---|---|---|---|---|---|
| 90 | 42.707 | 44.455 | 46.299 | 47.999 | 49.985 |
| 120 | 46.058 | 48.640 | 51.478 | 54.227 | 56.702 |
| 150 | 46.739 | 50.473 | 53.796 | 56.905 | 60.622 |
| 180 | 45.491 | 49.728 | 54.119 | 58.203 | 62.844 |
| 210 | 42.473 | 48.126 | 53.037 | 58.813 | 64.104 |
| 240 | 39.220 | 45.617 | 52.130 | 58.902 | 64.807 |
| 270 | 36.221 | 44.415 | 52.343 | 60.513 | 68.945 |
| 300 | 36.147 | 46.011 | 55.747 | 65.789 | 76.156 |
| 330 | 42.187 | 54.755 | 68.202 | 79.777 | 91.483 |

TABLE s8. ρ-T-p relation for near-critical methanol

| ρ [kg/m$^3$] | 505 K | 515 K | 525 K | 535 K | 545 K | 555 K |
|---|---|---|---|---|---|---|
| 50 | 42.612 | 45.114 | 47.533 | 50.058 | 52.047 | 54.287 |
| 100 | 56.628 | 62.087 | 67.498 | 72.649 | 77.848 | 82.714 |
| 150 | 59.036 | 67.162 | 74.628 | 82.346 | 90.602 | 98.049 |
| 200 | 56.117 | 66.066 | 76.852 | 86.358 | 96.783 | 106.412 |
| 250 | 50.893 | 63.997 | 75.354 | 87.938 | 100.569 | 113.490 |
| 300 | 43.954 | 58.848 | 73.577 | 88.376 | 103.999 | 121.075 |
| 350 | 37.144 | 54.690 | 72.027 | 91.298 | 109.952 | 130.427 |
| 400 | 32.791 | 56.475 | 77.555 | 100.681 | 125.947 | 149.676 |
| 450 | 41.155 | 67.745 | 100.722 | 130.368 | 160.277 | 189.171 |

TABLE s9. ρ-T-p relation for near-critical water

| ρ [kg/m$^3$] | 635 K | 640 K | 645 K | 650 K | 655 K |
|---|---|---|---|---|---|
| 150 | 141.300 | 147.334 | 154.861 | 160.595 | 167.222 |
| 200 | 142.015 | 150.342 | 159.280 | 168.267 | 175.888 |
| 250 | 139.112 | 149.540 | 159.732 | 169.162 | 179.900 |
| 290 | 135.968 | 147.220 | 158.731 | 169.145 | 180.699 |
| 320 | 130.293 | 144.821 | 156.643 | 169.616 | 182.324 |
| 350 | 127.396 | 141.504 | 155.221 | 168.406 | 183.601 |
| 390 | 123.804 | 139.016 | 154.689 | 170.276 | 190.102 |
| 440 | 123.468 | 138.700 | 161.475 | 180.306 | 200.570 |
| 490 | 132.238 | 157.294 | 182.307 | 205.241 | 229.704 |

TABLE s10. ρ-T-p relation for near-critical carbon dioxide

| ρ [kg/m$^3$] | 300 K | 305 K | 310 K | 315 K | 320 K |
|---|---|---|---|---|---|
| 200 | 64.517 | 67.725 | 70.674 | 73.618 | 76.466 |
| 250 | 68.698 | 72.682 | 77.174 | 81.521 | 85.281 |
| 300 | 70.609 | 76.084 | 80.987 | 85.776 | 91.415 |
| 350 | 69.528 | 76.551 | 83.227 | 89.681 | 95.387 |
| 400 | 68.485 | 76.322 | 83.485 | 91.078 | 98.643 |
| 430 | 67.362 | 75.222 | 83.445 | 91.486 | 100.220 |
| 460 | 64.784 | 74.400 | 83.193 | 92.307 | 101.339 |
| 490 | 63.291 | 72.863 | 82.885 | 92.817 | 102.857 |
| 520 | 61.054 | 71.997 | 82.180 | 93.606 | 103.905 |
| 570 | 58.484 | 69.945 | 83.385 | 94.932 | 109.758 |
| 620 | 54.856 | 71.292 | 85.001 | 99.734 | 113.710 |
| 670 | 57.504 | 73.294 | 89.633 | 106.516 | 122.102 |

TABLE s11. ρ-T-p relation for near-critical nitrogen

| ρ [kg/m$^3$] | 120 K | 125 K | 130 K | 135 K | 140 K |
|---|---|---|---|---|---|
| 120 | 25.435 | 27.918 | 30.467 | 32.787 | 35.249 |
| 160 | 27.488 | 31.146 | 34.954 | 38.410 | 41.943 |
| 200 | 27.960 | 32.648 | 37.609 | 42.158 | 46.824 |
| 240 | 26.607 | 32.901 | 38.994 | 44.857 | 50.916 |
| 280 | 24.923 | 32.148 | 39.352 | 46.834 | 54.318 |
| 320 | 22.230 | 30.739 | 39.535 | 48.537 | 57.327 |
| 360 | 19.149 | 29.246 | 39.959 | 51.111 | 61.898 |
| 400 | 16.943 | 28.855 | 41.368 | 54.455 | 67.124 |
| 440 | 14.784 | 29.196 | 45.031 | 60.185 | 76.924 |
| 480 | 14.927 | 33.700 | 52.573 | 71.405 | 90.635 |

relation of near-critical fluids used to estimate the critical point according to the flat top proposal. Pressure data are given in bar.

## FINITE-SIZE SCALING ANALYSIS

Tables s12-s16 shows the fractions of gas-like molecules and the probabilities of finding an infinite cluster in a configuration. They are obtained from the NVT simulations at $\rho_r = 0.75 - 1.17$ at $T_r = 3.50$. These data are used to conduct the finite-size scaling analysis to determine the probability of finding an infinite cluster in a configuration when the system size is infinitely large.

## THERMODYNAMIC PROPERTIES AND STRUCTURAL CHARACTERISTICS

Tables s17-s26 contain the ρ-T-p relation of supercritical fluids and the structural characteristics. All data are from the simulations of $N = 1,000$ molecules.

[1]V. K. Shen, D. W. Siderius, W. P. Krekelberg, and H. W. Hatch, "Nist standard reference simulation website, nist standard reference database number 173, national institute of standards and technology, gaithersburg md, 20899," (2018).
[2]J. K. Johnson, J. A. Zollweg, and K. E. Gubbins, Molecular Physics **78**, 591 (1993).

TABLE s12. Percolation behavior of $N = 1,000$ systems

| $\rho_r$ | $\Pi_{liq}$ | $p_{inf}^{gas}$ | $p_{inf}^{liq}$ |
|---|---|---|---|
| 0.750 | 0.000 | 1.000 | 0.000 |
| 0.768 | 0.000 | 1.000 | 0.000 |
| 0.787 | 0.001 | 1.000 | 0.000 |
| 0.805 | 0.002 | 1.000 | 0.000 |
| 0.823 | 0.004 | 1.000 | 0.000 |
| 0.841 | 0.009 | 1.000 | 0.000 |
| 0.860 | 0.019 | 1.000 | 0.000 |
| 0.878 | 0.037 | 1.000 | 0.004 |
| 0.896 | 0.064 | 1.000 | 0.034 |
| 0.914 | 0.110 | 1.000 | 0.138 |
| 0.933 | 0.181 | 1.000 | 0.508 |
| 0.951 | 0.282 | 1.000 | 0.930 |
| 0.969 | 0.399 | 1.000 | 0.994 |
| 0.987 | 0.526 | 1.000 | 1.000 |
| 1.006 | 0.658 | 1.000 | 1.000 |
| 1.024 | 0.771 | 0.978 | 1.000 |
| 1.042 | 0.863 | 0.660 | 1.000 |
| 1.060 | 0.928 | 0.200 | 1.000 |
| 1.079 | 0.966 | 0.038 | 1.000 |
| 1.097 | 0.987 | 0.004 | 1.000 |
| 1.115 | 0.995 | 0.000 | 1.000 |
| 1.133 | 0.998 | 0.000 | 1.000 |
| 1.152 | 1.000 | 0.000 | 1.000 |
| 1.170 | 1.000 | 0.000 | 1.000 |

TABLE s13. Percolation behavior of $N = 2,000$ systems

| $\rho_r$ | $\Pi_{liq}$ | $p_{inf}^{gas}$ | $p_{inf}^{liq}$ |
|---|---|---|---|
| 0.750 | 0.000 | 1.000 | 0.000 |
| 0.768 | 0.000 | 1.000 | 0.000 |
| 0.787 | 0.001 | 1.000 | 0.000 |
| 0.805 | 0.002 | 1.000 | 0.000 |
| 0.823 | 0.005 | 1.000 | 0.000 |
| 0.841 | 0.010 | 1.000 | 0.000 |
| 0.860 | 0.019 | 1.000 | 0.000 |
| 0.878 | 0.037 | 1.000 | 0.000 |
| 0.896 | 0.069 | 1.000 | 0.008 |
| 0.914 | 0.118 | 1.000 | 0.154 |
| 0.933 | 0.190 | 1.000 | 0.610 |
| 0.951 | 0.281 | 1.000 | 0.978 |
| 0.969 | 0.400 | 1.000 | 1.000 |
| 0.987 | 0.528 | 1.000 | 1.000 |
| 1.006 | 0.657 | 1.000 | 1.000 |
| 1.024 | 0.772 | 1.000 | 1.000 |
| 1.042 | 0.861 | 0.770 | 1.000 |
| 1.060 | 0.925 | 0.174 | 1.000 |
| 1.079 | 0.964 | 0.012 | 1.000 |
| 1.097 | 0.985 | 0.000 | 1.000 |
| 1.115 | 0.994 | 0.000 | 1.000 |
| 1.133 | 0.998 | 0.000 | 1.000 |
| 1.152 | 1.000 | 0.000 | 1.000 |
| 1.170 | 1.000 | 0.000 | 1.000 |

TABLE s14. Percolation behavior of $N = 4,000$ systems

| $\rho_r$ | $\Pi_{liq}$ | $p_{inf}^{gas}$ | $p_{inf}^{liq}$ |
|---|---|---|---|
| 0.750 | 0.000 | 1.000 | 0.000 |
| 0.768 | 0.000 | 1.000 | 0.000 |
| 0.787 | 0.001 | 1.000 | 0.000 |
| 0.805 | 0.002 | 1.000 | 0.000 |
| 0.823 | 0.005 | 1.000 | 0.000 |
| 0.841 | 0.010 | 1.000 | 0.000 |
| 0.860 | 0.020 | 1.000 | 0.000 |
| 0.878 | 0.039 | 1.000 | 0.000 |
| 0.896 | 0.072 | 1.000 | 0.020 |
| 0.914 | 0.120 | 1.000 | 0.150 |
| 0.933 | 0.190 | 1.000 | 0.644 |
| 0.951 | 0.286 | 1.000 | 0.996 |
| 0.969 | 0.400 | 1.000 | 1.000 |
| 0.987 | 0.528 | 1.000 | 1.000 |
| 1.006 | 0.655 | 1.000 | 1.000 |
| 1.024 | 0.768 | 1.000 | 1.000 |
| 1.042 | 0.859 | 0.846 | 1.000 |
| 1.060 | 0.923 | 0.164 | 1.000 |
| 1.079 | 0.963 | 0.004 | 1.000 |
| 1.097 | 0.984 | 0.002 | 1.000 |
| 1.115 | 0.994 | 0.000 | 1.000 |
| 1.133 | 0.998 | 0.000 | 1.000 |
| 1.152 | 1.000 | 0.000 | 1.000 |
| 1.170 | 1.000 | 0.000 | 1.000 |

TABLE s15. Percolation behavior of $N = 8,000$ systems

| $\rho_r$ | $\Pi_{liq}$ | $p_{inf}^{gas}$ | $p_{inf}^{liq}$ |
|---|---|---|---|
| 0.750 | 0.000 | 1.000 | 0.000 |
| 0.768 | 0.000 | 1.000 | 0.000 |
| 0.787 | 0.001 | 1.000 | 0.000 |
| 0.805 | 0.002 | 1.000 | 0.000 |
| 0.823 | 0.005 | 1.000 | 0.000 |
| 0.841 | 0.010 | 1.000 | 0.000 |
| 0.860 | 0.020 | 1.000 | 0.000 |
| 0.878 | 0.040 | 1.000 | 0.000 |
| 0.896 | 0.070 | 1.000 | 0.008 |
| 0.914 | 0.124 | 1.000 | 0.108 |
| 0.933 | 0.190 | 1.000 | 0.714 |
| 0.951 | 0.288 | 1.000 | 1.000 |
| 0.969 | 0.402 | 1.000 | 1.000 |
| 0.987 | 0.527 | 1.000 | 1.000 |
| 1.006 | 0.656 | 1.000 | 1.000 |
| 1.024 | 0.770 | 1.000 | 1.000 |
| 1.042 | 0.856 | 0.884 | 1.000 |
| 1.060 | 0.920 | 0.182 | 1.000 |
| 1.079 | 0.962 | 0.006 | 1.000 |
| 1.097 | 0.984 | 0.000 | 1.000 |
| 1.115 | 0.994 | 0.000 | 1.000 |
| 1.133 | 0.998 | 0.000 | 1.000 |
| 1.152 | 0.999 | 0.000 | 1.000 |
| 1.170 | 1.000 | 0.000 | 1.000 |

TABLE s16. Percolation behavior of $N = 16,000$ systems

| $\rho_r$ | $\Pi_{liq}$ | $p_{inf}^{gas}$ | $p_{inf}^{liq}$ |
|---|---|---|---|
| 0.750 | 0.000 | 1.000 | 0.000 |
| 0.768 | 0.000 | 1.000 | 0.000 |
| 0.787 | 0.001 | 1.000 | 0.000 |
| 0.805 | 0.002 | 1.000 | 0.000 |
| 0.823 | 0.005 | 1.000 | 0.000 |
| 0.841 | 0.011 | 1.000 | 0.000 |
| 0.860 | 0.021 | 1.000 | 0.000 |
| 0.878 | 0.040 | 1.000 | 0.000 |
| 0.896 | 0.073 | 1.000 | 0.000 |
| 0.914 | 0.121 | 1.000 | 0.066 |
| 0.933 | 0.194 | 1.000 | 0.850 |
| 0.951 | 0.288 | 1.000 | 1.000 |
| 0.969 | 0.402 | 1.000 | 1.000 |
| 0.987 | 0.528 | 1.000 | 1.000 |
| 1.006 | 0.654 | 1.000 | 1.000 |
| 1.024 | 0.767 | 1.000 | 1.000 |
| 1.042 | 0.858 | 0.968 | 1.000 |
| 1.060 | 0.922 | 0.090 | 1.000 |
| 1.079 | 0.962 | 0.000 | 1.000 |
| 1.097 | 0.984 | 0.000 | 1.000 |
| 1.115 | 0.994 | 0.000 | 1.000 |
| 1.133 | 0.998 | 0.000 | 1.000 |
| 1.152 | 0.999 | 0.000 | 1.000 |
| 1.170 | 1.000 | 0.000 | 1.000 |

TABLE s17: Thermodynamic and structural properties of argon

| $T/T_c$ | $\rho/\rho_c$ | $p/p_c$ | $z$ | $\Pi_{gas}$ | $p^{gas}_{inf}$ | $p^{liq}_{inf}$ | $\langle n^{gas}_c \rangle$ | $\langle n^{liq}_c \rangle$ |
|---|---|---|---|---|---|---|---|---|
| 1.000 | 0.500 | 0.804 | 0.638 | 0.997 | 1.000 | 0.000 | 1.000 | 0.436 |
| 1.000 | 0.600 | 0.873 | 0.577 | 0.976 | 1.000 | 0.000 | 1.000 | 2.149 |
| 1.000 | 0.700 | 0.931 | 0.527 | 0.913 | 1.000 | 0.020 | 1.000 | 3.693 |
| 1.000 | 0.800 | 0.973 | 0.482 | 0.749 | 1.000 | 0.604 | 1.000 | 2.178 |
| 1.000 | 0.900 | 1.002 | 0.441 | 0.524 | 1.000 | 1.000 | 1.000 | 1.218 |
| 1.000 | 1.000 | 1.027 | 0.407 | 0.298 | 1.000 | 1.000 | 1.000 | 1.020 |
| 1.000 | 1.100 | 1.043 | 0.376 | 0.132 | 0.881 | 1.000 | 1.069 | 1.000 |
| 1.000 | 1.200 | 1.063 | 0.351 | 0.040 | 0.149 | 1.000 | 1.505 | 1.000 |
| 1.000 | 1.300 | 1.075 | 0.328 | 0.008 | 0.020 | 1.000 | 0.881 | 1.000 |
| 1.000 | 1.400 | 1.121 | 0.317 | 0.001 | 0.000 | 1.000 | 0.277 | 1.000 |
| 1.000 | 1.500 | 1.184 | 0.313 | 0.000 | 0.000 | 1.000 | 0.020 | 1.000 |
| 1.010 | 0.500 | 0.818 | 0.642 | 0.999 | 1.000 | 0.000 | 1.000 | 0.406 |
| 1.010 | 0.600 | 0.818 | 0.535 | 0.980 | 1.000 | 0.000 | 1.000 | 2.337 |
| 1.010 | 0.700 | 0.895 | 0.502 | 0.912 | 1.000 | 0.030 | 1.000 | 3.614 |
| 1.010 | 0.800 | 0.957 | 0.470 | 0.760 | 1.000 | 0.515 | 1.000 | 2.327 |
| 1.010 | 0.900 | 1.007 | 0.439 | 0.533 | 1.000 | 1.000 | 1.000 | 1.198 |
| 1.010 | 1.000 | 1.034 | 0.406 | 0.296 | 1.000 | 1.000 | 1.010 | 1.020 |
| 1.010 | 1.100 | 1.064 | 0.380 | 0.120 | 0.842 | 1.000 | 1.208 | 1.000 |
| 1.010 | 1.200 | 1.094 | 0.358 | 0.035 | 0.109 | 1.000 | 1.475 | 1.000 |
| 1.010 | 1.300 | 1.116 | 0.337 | 0.006 | 0.000 | 1.000 | 0.861 | 1.000 |
| 1.010 | 1.400 | 1.150 | 0.322 | 0.000 | 0.000 | 1.000 | 0.149 | 1.000 |
| 1.010 | 1.500 | 1.201 | 0.314 | 0.000 | 0.000 | 1.000 | 0.000 | 1.000 |
| 1.050 | 0.350 | 0.701 | 0.757 | 1.000 | 1.000 | 0.000 | 1.000 | 0.010 |
| 1.050 | 0.550 | 0.939 | 0.645 | 0.995 | 1.000 | 0.000 | 1.000 | 0.891 |
| 1.050 | 0.750 | 1.097 | 0.552 | 0.869 | 1.000 | 0.079 | 1.000 | 3.842 |
| 1.050 | 0.870 | 1.170 | 0.508 | 0.627 | 1.000 | 0.960 | 1.000 | 1.366 |
| 1.050 | 0.970 | 1.221 | 0.475 | 0.365 | 1.000 | 1.000 | 1.010 | 1.040 |
| 1.050 | 1.070 | 1.280 | 0.452 | 0.163 | 0.941 | 1.000 | 1.050 | 1.000 |
| 1.050 | 1.170 | 1.324 | 0.427 | 0.045 | 0.149 | 1.000 | 1.436 | 1.000 |
| 1.050 | 1.350 | 1.442 | 0.403 | 0.001 | 0.000 | 1.000 | 0.208 | 1.000 |
| 1.050 | 1.550 | 1.676 | 0.408 | 0.000 | 0.000 | 1.000 | 0.000 | 1.000 |
| 1.050 | 1.750 | 2.085 | 0.450 | 0.000 | 0.000 | 1.000 | 0.000 | 1.000 |
| 1.050 | 1.950 | 2.871 | 0.556 | 0.000 | 0.000 | 1.000 | 0.000 | 1.000 |
| 1.100 | 0.350 | 0.757 | 0.780 | 1.000 | 1.000 | 0.000 | 1.000 | 0.000 |
| 1.100 | 0.550 | 1.039 | 0.681 | 0.998 | 1.000 | 0.000 | 1.000 | 0.564 |
| 1.100 | 0.750 | 1.243 | 0.598 | 0.893 | 1.000 | 0.059 | 1.000 | 3.802 |
| 1.100 | 0.870 | 1.356 | 0.562 | 0.646 | 1.000 | 0.950 | 1.000 | 1.505 |
| 1.100 | 0.970 | 1.429 | 0.531 | 0.374 | 1.000 | 1.000 | 1.010 | 1.059 |
| 1.100 | 1.070 | 1.509 | 0.508 | 0.154 | 0.851 | 1.000 | 1.099 | 1.000 |
| 1.100 | 1.170 | 1.591 | 0.490 | 0.038 | 0.139 | 1.000 | 1.653 | 1.000 |
| 1.100 | 1.350 | 1.783 | 0.476 | 0.000 | 0.000 | 1.000 | 0.208 | 1.000 |
| 1.100 | 1.550 | 2.109 | 0.491 | 0.000 | 0.000 | 1.000 | 0.000 | 1.000 |
| 1.100 | 1.750 | 2.664 | 0.549 | 0.000 | 0.000 | 1.000 | 0.000 | 1.000 |
| 1.100 | 1.950 | 3.635 | 0.672 | 0.000 | 0.000 | 1.000 | 0.000 | 1.000 |
| 1.150 | 0.350 | 0.812 | 0.800 | 1.000 | 1.000 | 0.000 | 1.000 | 0.000 |
| 1.150 | 0.550 | 1.133 | 0.710 | 0.998 | 1.000 | 0.000 | 1.000 | 0.356 |
| 1.150 | 0.750 | 1.386 | 0.637 | 0.905 | 1.000 | 0.050 | 1.000 | 3.743 |
| 1.150 | 0.870 | 1.517 | 0.601 | 0.669 | 1.000 | 0.891 | 1.000 | 1.525 |
| 1.150 | 0.970 | 1.631 | 0.580 | 0.379 | 1.000 | 1.000 | 1.010 | 1.050 |
| 1.150 | 1.070 | 1.743 | 0.562 | 0.147 | 0.881 | 1.000 | 1.158 | 1.000 |
| 1.150 | 1.170 | 1.863 | 0.549 | 0.030 | 0.020 | 1.000 | 1.693 | 1.000 |
| 1.150 | 1.350 | 2.136 | 0.546 | 0.000 | 0.000 | 1.000 | 0.119 | 1.000 |
| 1.150 | 1.550 | 2.550 | 0.567 | 0.000 | 0.000 | 1.000 | 0.000 | 1.000 |
| 1.150 | 1.750 | 3.235 | 0.638 | 0.000 | 0.000 | 1.000 | 0.000 | 1.000 |
| 1.150 | 1.950 | 4.346 | 0.769 | 0.000 | 0.000 | 1.000 | 0.000 | 1.000 |
| 1.200 | 0.350 | 0.866 | 0.818 | 1.000 | 1.000 | 0.000 | 1.000 | 0.000 |
| 1.200 | 0.550 | 1.228 | 0.738 | 0.999 | 1.000 | 0.000 | 1.000 | 0.267 |
| 1.200 | 0.750 | 1.528 | 0.673 | 0.925 | 1.000 | 0.000 | 1.000 | 3.970 |
| 1.200 | 0.870 | 1.699 | 0.645 | 0.688 | 1.000 | 0.911 | 1.000 | 1.802 |
| 1.200 | 0.970 | 1.833 | 0.625 | 0.391 | 1.000 | 1.000 | 1.010 | 1.059 |

*Continued on next page*

TABLE s17 – Thermodynamic and structural properties of argon (continued)

| $T/T_c$ | $\rho/\rho_c$ | $p/p_c$ | $z$ | $\Pi_{gas}$ | $p_{inf}^{gas}$ | $p_{inf}^{liq}$ | $\langle n_c^{gas}\rangle$ | $\langle n_c^{liq}\rangle$ |
|---|---|---|---|---|---|---|---|---|
| 1.200 | 1.070 | 1.982 | 0.612 | 0.140 | 0.832 | 1.000 | 1.119 | 1.000 |
| 1.200 | 1.170 | 2.138 | 0.604 | 0.026 | 0.020 | 1.000 | 1.713 | 1.000 |
| 1.200 | 1.350 | 2.462 | 0.603 | 0.000 | 0.000 | 1.000 | 0.089 | 1.000 |
| 1.200 | 1.550 | 2.993 | 0.638 | 0.000 | 0.000 | 1.000 | 0.000 | 1.000 |
| 1.200 | 1.750 | 3.813 | 0.720 | 0.000 | 0.000 | 1.000 | 0.000 | 1.000 |
| 1.200 | 1.950 | 5.074 | 0.860 | 0.000 | 0.000 | 1.000 | 0.000 | 1.000 |
| 1.250 | 0.350 | 0.920 | 0.834 | 1.000 | 1.000 | 0.000 | 1.000 | 0.000 |
| 1.250 | 0.550 | 1.323 | 0.763 | 0.999 | 1.000 | 0.000 | 1.000 | 0.228 |
| 1.250 | 0.750 | 1.672 | 0.707 | 0.925 | 1.000 | 0.030 | 1.000 | 3.851 |
| 1.250 | 0.870 | 1.871 | 0.682 | 0.709 | 1.000 | 0.762 | 1.000 | 1.733 |
| 1.250 | 0.970 | 2.039 | 0.667 | 0.390 | 1.000 | 1.000 | 1.000 | 1.050 |
| 1.250 | 1.070 | 2.217 | 0.657 | 0.138 | 0.812 | 1.000 | 1.129 | 1.000 |
| 1.250 | 1.170 | 2.404 | 0.652 | 0.023 | 0.030 | 1.000 | 1.723 | 1.000 |
| 1.250 | 1.350 | 2.814 | 0.661 | 0.000 | 0.000 | 1.000 | 0.040 | 1.000 |
| 1.250 | 1.550 | 3.444 | 0.705 | 0.000 | 0.000 | 1.000 | 0.000 | 1.000 |
| 1.250 | 1.750 | 4.382 | 0.794 | 0.000 | 0.000 | 1.000 | 0.000 | 1.000 |
| 1.250 | 1.950 | 5.820 | 0.947 | 0.000 | 0.000 | 1.000 | 0.000 | 1.000 |
| 1.300 | 0.350 | 0.976 | 0.851 | 1.000 | 1.000 | 0.000 | 1.000 | 0.000 |
| 1.300 | 0.550 | 1.417 | 0.786 | 0.999 | 1.000 | 0.000 | 1.000 | 0.178 |
| 1.300 | 0.750 | 1.815 | 0.738 | 0.940 | 1.000 | 0.000 | 1.000 | 4.069 |
| 1.300 | 0.870 | 2.046 | 0.717 | 0.713 | 1.000 | 0.842 | 1.000 | 1.802 |
| 1.300 | 0.970 | 2.242 | 0.705 | 0.404 | 1.000 | 1.000 | 1.000 | 1.059 |
| 1.300 | 1.070 | 2.449 | 0.698 | 0.131 | 0.743 | 1.000 | 1.356 | 1.000 |
| 1.300 | 1.170 | 2.676 | 0.698 | 0.020 | 0.020 | 1.000 | 1.683 | 1.000 |
| 1.300 | 1.350 | 3.163 | 0.715 | 0.000 | 0.000 | 1.000 | 0.020 | 1.000 |
| 1.300 | 1.550 | 3.897 | 0.767 | 0.000 | 0.000 | 1.000 | 0.000 | 1.000 |
| 1.300 | 1.750 | 4.955 | 0.864 | 0.000 | 0.000 | 1.000 | 0.000 | 1.000 |
| 1.300 | 1.950 | 6.530 | 1.022 | 0.000 | 0.000 | 1.000 | 0.000 | 1.000 |
| 1.500 | 0.350 | 1.190 | 0.899 | 1.000 | 1.000 | 0.000 | 1.000 | 0.000 |
| 1.500 | 0.550 | 1.788 | 0.860 | 1.000 | 1.000 | 0.000 | 1.000 | 0.149 |
| 1.500 | 0.750 | 2.368 | 0.835 | 0.957 | 1.000 | 0.000 | 1.000 | 3.683 |
| 1.500 | 0.870 | 2.733 | 0.831 | 0.752 | 1.000 | 0.663 | 1.000 | 2.178 |
| 1.500 | 0.970 | 3.054 | 0.832 | 0.408 | 1.000 | 1.000 | 1.010 | 1.059 |
| 1.500 | 1.070 | 3.390 | 0.838 | 0.122 | 0.663 | 1.000 | 1.327 | 1.000 |
| 1.500 | 1.170 | 3.763 | 0.850 | 0.016 | 0.000 | 1.000 | 1.584 | 1.000 |
| 1.500 | 1.350 | 4.538 | 0.889 | 0.000 | 0.000 | 1.000 | 0.020 | 1.000 |
| 1.500 | 1.550 | 5.661 | 0.966 | 0.000 | 0.000 | 1.000 | 0.000 | 1.000 |
| 1.500 | 1.750 | 7.200 | 1.088 | 0.000 | 0.000 | 1.000 | 0.000 | 1.000 |
| 1.500 | 1.950 | 9.368 | 1.270 | 0.000 | 0.000 | 1.000 | 0.000 | 1.000 |
| 1.900 | 0.350 | 1.612 | 0.961 | 1.000 | 1.000 | 0.000 | 1.000 | 0.000 |
| 1.900 | 0.550 | 2.520 | 0.956 | 1.000 | 1.000 | 0.000 | 1.000 | 0.020 |
| 1.900 | 0.750 | 3.481 | 0.969 | 0.973 | 1.000 | 0.000 | 1.000 | 3.188 |
| 1.900 | 0.870 | 4.090 | 0.981 | 0.793 | 1.000 | 0.505 | 1.000 | 2.693 |
| 1.900 | 0.970 | 4.643 | 0.999 | 0.428 | 1.000 | 1.000 | 1.000 | 1.030 |
| 1.900 | 1.070 | 5.247 | 1.024 | 0.107 | 0.564 | 1.000 | 1.554 | 1.000 |
| 1.900 | 1.170 | 5.892 | 1.051 | 0.009 | 0.000 | 1.000 | 1.267 | 1.000 |
| 1.900 | 1.350 | 7.257 | 1.122 | 0.000 | 0.000 | 1.000 | 0.000 | 1.000 |
| 1.900 | 1.550 | 9.141 | 1.231 | 0.000 | 0.000 | 1.000 | 0.000 | 1.000 |
| 1.900 | 1.750 | 11.601 | 1.384 | 0.000 | 0.000 | 1.000 | 0.000 | 1.000 |
| 1.900 | 1.950 | 14.877 | 1.593 | 0.000 | 0.000 | 1.000 | 0.000 | 1.000 |
| 2.100 | 0.350 | 1.821 | 0.983 | 1.000 | 1.000 | 0.000 | 1.000 | 0.000 |
| 2.100 | 0.550 | 2.886 | 0.991 | 1.000 | 1.000 | 0.000 | 1.000 | 0.040 |
| 2.100 | 0.750 | 4.023 | 1.013 | 0.978 | 1.000 | 0.000 | 1.000 | 2.842 |
| 2.100 | 0.870 | 4.765 | 1.034 | 0.808 | 1.000 | 0.455 | 1.000 | 2.911 |
| 2.100 | 0.970 | 5.438 | 1.059 | 0.432 | 1.000 | 1.000 | 1.020 | 1.069 |
| 2.100 | 1.070 | 6.152 | 1.086 | 0.103 | 0.475 | 1.000 | 1.505 | 1.010 |
| 2.100 | 1.170 | 6.936 | 1.120 | 0.008 | 0.000 | 1.000 | 1.356 | 1.000 |
| 2.100 | 1.350 | 8.598 | 1.203 | 0.000 | 0.000 | 1.000 | 0.000 | 1.000 |
| 2.100 | 1.550 | 10.846 | 1.322 | 0.000 | 0.000 | 1.000 | 0.000 | 1.000 |
| 2.100 | 1.750 | 13.734 | 1.482 | 0.000 | 0.000 | 1.000 | 0.000 | 1.000 |
| 2.100 | 1.950 | 17.528 | 1.698 | 0.000 | 0.000 | 1.000 | 0.000 | 1.000 |

*Continued on next page*

TABLE s17 – Thermodynamic and structural properties of argon (continued)

| $T/T_c$ | $\rho/\rho_c$ | $p/p_c$ | $z$ | $\Pi_{gas}$ | $p^{gas}_{inf}$ | $p^{liq}_{inf}$ | $\langle n^{gas}_c \rangle$ | $\langle n^{liq}_c \rangle$ |
|---|---|---|---|---|---|---|---|---|
| 2.300 | 0.350 | 2.032 | 1.001 | 1.000 | 1.000 | 0.000 | 1.000 | 0.000 |
| 2.300 | 0.550 | 3.246 | 1.018 | 1.000 | 1.000 | 0.000 | 1.000 | 0.000 |
| 2.300 | 0.750 | 4.562 | 1.049 | 0.981 | 1.000 | 0.000 | 1.000 | 2.970 |
| 2.300 | 0.870 | 5.423 | 1.075 | 0.807 | 1.000 | 0.455 | 1.000 | 2.505 |
| 2.300 | 0.970 | 6.211 | 1.104 | 0.434 | 1.000 | 1.000 | 1.000 | 1.079 |
| 2.300 | 1.070 | 7.066 | 1.139 | 0.103 | 0.564 | 1.000 | 1.594 | 1.000 |
| 2.300 | 1.170 | 7.977 | 1.176 | 0.008 | 0.000 | 1.000 | 1.198 | 1.000 |
| 2.300 | 1.350 | 9.899 | 1.264 | 0.000 | 0.000 | 1.000 | 0.020 | 1.000 |
| 2.300 | 1.550 | 12.521 | 1.393 | 0.000 | 0.000 | 1.000 | 0.000 | 1.000 |
| 2.300 | 1.750 | 15.852 | 1.562 | 0.000 | 0.000 | 1.000 | 0.000 | 1.000 |
| 2.300 | 1.950 | 20.153 | 1.782 | 0.000 | 0.000 | 1.000 | 0.000 | 1.000 |
| 2.900 | 0.350 | 2.654 | 1.037 | 1.000 | 1.000 | 0.000 | 1.000 | 0.000 |
| 2.900 | 0.550 | 4.321 | 1.074 | 1.000 | 1.000 | 0.000 | 1.000 | 0.000 |
| 2.900 | 0.750 | 6.173 | 1.126 | 0.984 | 1.000 | 0.000 | 1.000 | 2.525 |
| 2.900 | 0.870 | 7.408 | 1.165 | 0.825 | 1.000 | 0.297 | 1.000 | 3.010 |
| 2.900 | 0.970 | 8.526 | 1.202 | 0.444 | 1.000 | 1.000 | 1.000 | 1.050 |
| 2.900 | 1.070 | 9.736 | 1.244 | 0.092 | 0.396 | 1.000 | 1.614 | 1.000 |
| 2.900 | 1.170 | 11.062 | 1.293 | 0.006 | 0.000 | 1.000 | 1.050 | 1.000 |
| 2.900 | 1.350 | 13.790 | 1.397 | 0.000 | 0.000 | 1.000 | 0.000 | 1.000 |
| 2.900 | 1.550 | 17.484 | 1.543 | 0.000 | 0.000 | 1.000 | 0.000 | 1.000 |
| 2.900 | 1.750 | 22.037 | 1.722 | 0.000 | 0.000 | 1.000 | 0.000 | 1.000 |
| 2.900 | 1.950 | 27.807 | 1.950 | 0.000 | 0.000 | 1.000 | 0.000 | 1.000 |
| 3.500 | 0.350 | 3.272 | 1.059 | 1.000 | 1.000 | 0.000 | 1.000 | 0.000 |
| 3.500 | 0.550 | 5.380 | 1.108 | 1.000 | 1.000 | 0.000 | 1.000 | 0.020 |
| 3.500 | 0.750 | 7.758 | 1.172 | 0.988 | 1.000 | 0.000 | 1.000 | 2.337 |
| 3.500 | 0.870 | 9.362 | 1.219 | 0.833 | 1.000 | 0.277 | 1.000 | 3.030 |
| 3.500 | 0.970 | 10.803 | 1.262 | 0.441 | 1.000 | 1.000 | 1.010 | 1.099 |
| 3.500 | 1.070 | 12.371 | 1.310 | 0.096 | 0.475 | 1.000 | 1.772 | 1.000 |
| 3.500 | 1.170 | 14.084 | 1.364 | 0.006 | 0.000 | 1.000 | 1.069 | 1.000 |
| 3.500 | 1.350 | 17.560 | 1.474 | 0.000 | 0.000 | 1.000 | 0.000 | 1.000 |
| 3.500 | 1.550 | 22.248 | 1.626 | 0.000 | 0.000 | 1.000 | 0.000 | 1.000 |
| 3.500 | 1.750 | 28.012 | 1.814 | 0.000 | 0.000 | 1.000 | 0.000 | 1.000 |
| 3.500 | 1.950 | 35.082 | 2.039 | 0.000 | 0.000 | 1.000 | 0.000 | 1.000 |

TABLE s18: Thermodynamic and structural properties of methane

| $T/T_c$ | $\rho/\rho_c$ | $p/p_c$ | $z$ | $\Pi_{gas}$ | $p^{gas}_{inf}$ | $p^{liq}_{inf}$ | $\langle n^{gas}_c \rangle$ | $\langle n^{liq}_c \rangle$ |
|---|---|---|---|---|---|---|---|---|
| 1.000 | 0.500 | 0.829 | 0.616 | 0.997 | 1.000 | 0.000 | 1.000 | 0.653 |
| 1.000 | 0.600 | 0.900 | 0.557 | 0.977 | 1.000 | 0.000 | 1.000 | 2.475 |
| 1.000 | 0.700 | 0.948 | 0.503 | 0.897 | 1.000 | 0.000 | 1.000 | 3.218 |
| 1.000 | 0.800 | 0.984 | 0.457 | 0.742 | 1.000 | 0.188 | 1.000 | 2.020 |
| 1.000 | 0.900 | 1.001 | 0.413 | 0.526 | 1.000 | 0.891 | 1.000 | 1.178 |
| 1.000 | 1.000 | 1.010 | 0.375 | 0.296 | 1.000 | 1.000 | 1.010 | 1.040 |
| 1.000 | 1.100 | 1.021 | 0.345 | 0.131 | 0.792 | 1.000 | 1.079 | 1.000 |
| 1.000 | 1.200 | 1.031 | 0.319 | 0.043 | 0.198 | 1.000 | 1.356 | 1.000 |
| 1.000 | 1.300 | 1.047 | 0.299 | 0.008 | 0.000 | 1.000 | 0.970 | 1.000 |
| 1.000 | 1.400 | 1.074 | 0.285 | 0.001 | 0.000 | 1.000 | 0.218 | 1.000 |
| 1.000 | 1.500 | 1.131 | 0.280 | 0.000 | 0.000 | 1.000 | 0.000 | 1.000 |
| 1.010 | 0.500 | 0.848 | 0.624 | 0.997 | 1.000 | 0.000 | 1.000 | 0.614 |
| 1.010 | 0.600 | 0.920 | 0.564 | 0.974 | 1.000 | 0.000 | 1.000 | 2.139 |
| 1.010 | 0.700 | 0.976 | 0.513 | 0.907 | 1.000 | 0.000 | 1.000 | 3.614 |
| 1.010 | 0.800 | 1.010 | 0.464 | 0.746 | 1.000 | 0.277 | 1.000 | 1.792 |
| 1.010 | 0.900 | 1.040 | 0.425 | 0.519 | 1.000 | 0.891 | 1.000 | 1.109 |
| 1.010 | 1.000 | 1.056 | 0.388 | 0.294 | 1.000 | 1.000 | 1.000 | 1.030 |
| 1.010 | 1.100 | 1.071 | 0.358 | 0.130 | 0.822 | 1.000 | 1.089 | 1.000 |
| 1.010 | 1.200 | 1.086 | 0.333 | 0.039 | 0.168 | 1.000 | 1.535 | 1.000 |
| 1.010 | 1.300 | 1.113 | 0.315 | 0.005 | 0.000 | 1.000 | 0.891 | 1.000 |
| 1.010 | 1.400 | 1.142 | 0.300 | 0.000 | 0.000 | 1.000 | 0.168 | 1.000 |
| 1.010 | 1.500 | 1.215 | 0.298 | 0.000 | 0.000 | 1.000 | 0.000 | 1.000 |

*Continued on next page*

TABLE s18 – Thermodynamic and structural properties of methane (continued)

| $T/T_c$ | $\rho/\rho_c$ | $p/p_c$ | $z$ | $\Pi_{gas}$ | $p^{gas}_{inf}$ | $p^{liq}_{inf}$ | $\langle n^{gas}_c \rangle$ | $\langle n^{liq}_c \rangle$ |
|---|---|---|---|---|---|---|---|---|
| 1.050 | 0.300 | 0.658 | 0.776 | 1.000 | 1.000 | 0.000 | 1.000 | 0.000 |
| 1.050 | 0.500 | 0.924 | 0.654 | 0.998 | 1.000 | 0.000 | 1.000 | 0.426 |
| 1.050 | 0.700 | 1.090 | 0.551 | 0.926 | 1.000 | 0.020 | 1.000 | 3.673 |
| 1.050 | 0.850 | 1.173 | 0.488 | 0.660 | 1.000 | 0.911 | 1.000 | 1.475 |
| 1.050 | 0.950 | 1.221 | 0.455 | 0.420 | 1.000 | 1.000 | 1.000 | 1.069 |
| 1.050 | 1.050 | 1.264 | 0.426 | 0.198 | 0.990 | 1.000 | 1.079 | 1.000 |
| 1.050 | 1.150 | 1.309 | 0.403 | 0.062 | 0.277 | 1.000 | 1.485 | 1.000 |
| 1.050 | 1.300 | 1.390 | 0.378 | 0.003 | 0.000 | 1.000 | 0.634 | 1.000 |
| 1.050 | 1.500 | 1.575 | 0.371 | 0.000 | 0.000 | 1.000 | 0.000 | 1.000 |
| 1.050 | 1.700 | 1.986 | 0.413 | 0.000 | 0.000 | 1.000 | 0.000 | 1.000 |
| 1.100 | 0.300 | 0.708 | 0.797 | 1.000 | 1.000 | 0.000 | 1.000 | 0.000 |
| 1.100 | 0.500 | 1.016 | 0.686 | 0.999 | 1.000 | 0.000 | 1.000 | 0.228 |
| 1.100 | 0.700 | 1.235 | 0.596 | 0.939 | 1.000 | 0.010 | 1.000 | 3.901 |
| 1.100 | 0.850 | 1.360 | 0.540 | 0.700 | 1.000 | 0.772 | 1.000 | 1.723 |
| 1.100 | 0.950 | 1.436 | 0.510 | 0.430 | 1.000 | 1.000 | 1.000 | 1.139 |
| 1.100 | 1.050 | 1.513 | 0.487 | 0.187 | 0.980 | 1.000 | 1.109 | 1.000 |
| 1.100 | 1.150 | 1.588 | 0.466 | 0.056 | 0.267 | 1.000 | 1.495 | 1.000 |
| 1.100 | 1.300 | 1.734 | 0.450 | 0.002 | 0.000 | 1.000 | 0.446 | 1.000 |
| 1.100 | 1.500 | 2.035 | 0.458 | 0.000 | 0.000 | 1.000 | 0.000 | 1.000 |
| 1.100 | 1.700 | 2.570 | 0.510 | 0.000 | 0.000 | 1.000 | 0.000 | 1.000 |
| 1.150 | 0.300 | 0.758 | 0.816 | 1.000 | 1.000 | 0.000 | 1.000 | 0.000 |
| 1.150 | 0.500 | 1.109 | 0.716 | 0.999 | 1.000 | 0.000 | 1.000 | 0.168 |
| 1.150 | 0.700 | 1.376 | 0.635 | 0.956 | 1.000 | 0.020 | 1.000 | 3.446 |
| 1.150 | 0.850 | 1.545 | 0.587 | 0.726 | 1.000 | 0.693 | 1.000 | 1.891 |
| 1.150 | 0.950 | 1.649 | 0.561 | 0.432 | 1.000 | 1.000 | 1.000 | 1.089 |
| 1.150 | 1.050 | 1.758 | 0.541 | 0.182 | 0.950 | 1.000 | 1.059 | 1.000 |
| 1.150 | 1.150 | 1.876 | 0.527 | 0.042 | 0.089 | 1.000 | 1.762 | 1.000 |
| 1.150 | 1.300 | 2.092 | 0.520 | 0.002 | 0.000 | 1.000 | 0.436 | 1.000 |
| 1.150 | 1.500 | 2.489 | 0.536 | 0.000 | 0.000 | 1.000 | 0.000 | 1.000 |
| 1.150 | 1.700 | 3.154 | 0.599 | 0.000 | 0.000 | 1.000 | 0.000 | 1.000 |
| 1.200 | 0.300 | 0.807 | 0.833 | 1.000 | 1.000 | 0.000 | 1.000 | 0.000 |
| 1.200 | 0.500 | 1.199 | 0.742 | 1.000 | 1.000 | 0.000 | 1.000 | 0.119 |
| 1.200 | 0.700 | 1.515 | 0.670 | 0.965 | 1.000 | 0.000 | 1.000 | 3.129 |
| 1.200 | 0.850 | 1.724 | 0.628 | 0.733 | 1.000 | 0.703 | 1.000 | 1.871 |
| 1.200 | 0.950 | 1.865 | 0.608 | 0.448 | 1.000 | 1.000 | 1.000 | 1.099 |
| 1.200 | 1.050 | 2.008 | 0.592 | 0.180 | 0.950 | 1.000 | 1.079 | 1.000 |
| 1.200 | 1.150 | 2.156 | 0.580 | 0.044 | 0.109 | 1.000 | 1.802 | 1.000 |
| 1.200 | 1.300 | 2.435 | 0.580 | 0.001 | 0.000 | 1.000 | 0.228 | 1.000 |
| 1.200 | 1.500 | 2.941 | 0.607 | 0.000 | 0.000 | 1.000 | 0.000 | 1.000 |
| 1.200 | 1.700 | 3.746 | 0.682 | 0.000 | 0.000 | 1.000 | 0.000 | 1.000 |
| 1.250 | 0.300 | 0.855 | 0.847 | 1.000 | 1.000 | 0.000 | 1.000 | 0.000 |
| 1.250 | 0.500 | 1.287 | 0.765 | 1.000 | 1.000 | 0.000 | 1.000 | 0.109 |
| 1.250 | 0.700 | 1.657 | 0.703 | 0.967 | 1.000 | 0.000 | 1.000 | 3.139 |
| 1.250 | 0.850 | 1.909 | 0.667 | 0.752 | 1.000 | 0.624 | 1.000 | 2.198 |
| 1.250 | 0.950 | 2.079 | 0.650 | 0.451 | 1.000 | 1.000 | 1.000 | 1.089 |
| 1.250 | 1.050 | 2.257 | 0.639 | 0.178 | 0.941 | 1.000 | 1.149 | 1.000 |
| 1.250 | 1.150 | 2.447 | 0.632 | 0.034 | 0.069 | 1.000 | 1.871 | 1.000 |
| 1.250 | 1.300 | 2.787 | 0.637 | 0.001 | 0.000 | 1.000 | 0.198 | 1.000 |
| 1.250 | 1.500 | 3.399 | 0.673 | 0.000 | 0.000 | 1.000 | 0.000 | 1.000 |
| 1.250 | 1.700 | 4.326 | 0.756 | 0.000 | 0.000 | 1.000 | 0.000 | 1.000 |
| 1.300 | 0.300 | 0.903 | 0.860 | 1.000 | 1.000 | 0.000 | 1.000 | 0.000 |
| 1.300 | 0.500 | 1.379 | 0.788 | 1.000 | 1.000 | 0.000 | 1.000 | 0.059 |
| 1.300 | 0.700 | 1.792 | 0.731 | 0.974 | 1.000 | 0.000 | 1.000 | 2.832 |
| 1.300 | 0.850 | 2.089 | 0.702 | 0.758 | 1.000 | 0.644 | 1.000 | 2.129 |
| 1.300 | 0.950 | 2.288 | 0.688 | 0.461 | 1.000 | 1.000 | 1.010 | 1.119 |
| 1.300 | 1.050 | 2.502 | 0.681 | 0.178 | 0.950 | 1.000 | 1.139 | 1.000 |
| 1.300 | 1.150 | 2.736 | 0.680 | 0.032 | 0.089 | 1.000 | 1.693 | 1.000 |
| 1.300 | 1.300 | 3.139 | 0.690 | 0.001 | 0.000 | 1.000 | 0.178 | 1.000 |
| 1.300 | 1.500 | 3.863 | 0.736 | 0.000 | 0.000 | 1.000 | 0.000 | 1.000 |
| 1.300 | 1.700 | 4.918 | 0.826 | 0.000 | 0.000 | 1.000 | 0.000 | 1.000 |
| 1.500 | 0.300 | 1.097 | 0.905 | 1.000 | 1.000 | 0.000 | 1.000 | 0.000 |

*Continued on next page*

TABLE s18 – Thermodynamic and structural properties of methane (continued)

| $T/T_c$ | $\rho/\rho_c$ | $p/p_c$ | $z$ | $\Pi_{gas}$ | $p_{inf}^{gas}$ | $p_{inf}^{liq}$ | $\langle n_c^{gas}\rangle$ | $\langle n_c^{liq}\rangle$ |
|---|---|---|---|---|---|---|---|---|
| 1.500 | 0.500 | 1.733 | 0.858 | 1.000 | 1.000 | 0.000 | 1.000 | 0.000 |
| 1.500 | 0.700 | 2.341 | 0.828 | 0.986 | 1.000 | 0.000 | 1.000 | 2.287 |
| 1.500 | 0.850 | 2.806 | 0.817 | 0.808 | 1.000 | 0.327 | 1.000 | 2.644 |
| 1.500 | 0.950 | 3.135 | 0.817 | 0.487 | 1.000 | 1.000 | 1.000 | 1.129 |
| 1.500 | 1.050 | 3.492 | 0.823 | 0.170 | 0.891 | 1.000 | 1.208 | 1.000 |
| 1.500 | 1.150 | 3.867 | 0.833 | 0.025 | 0.040 | 1.000 | 1.792 | 1.000 |
| 1.500 | 1.300 | 4.540 | 0.865 | 0.000 | 0.000 | 1.000 | 0.059 | 1.000 |
| 1.500 | 1.500 | 5.668 | 0.936 | 0.000 | 0.000 | 1.000 | 0.000 | 1.000 |
| 1.500 | 1.700 | 7.243 | 1.055 | 0.000 | 0.000 | 1.000 | 0.000 | 1.000 |
| 1.700 | 0.300 | 1.287 | 0.937 | 1.000 | 1.000 | 0.000 | 1.000 | 0.000 |
| 1.700 | 0.500 | 2.086 | 0.911 | 1.000 | 1.000 | 0.000 | 1.000 | 0.010 |
| 1.700 | 0.700 | 2.889 | 0.902 | 0.990 | 1.000 | 0.000 | 1.000 | 1.861 |
| 1.700 | 0.850 | 3.517 | 0.904 | 0.822 | 1.000 | 0.297 | 1.000 | 3.089 |
| 1.700 | 0.950 | 3.972 | 0.913 | 0.501 | 1.000 | 1.000 | 1.000 | 1.198 |
| 1.700 | 1.050 | 4.465 | 0.929 | 0.157 | 0.851 | 1.000 | 1.188 | 1.020 |
| 1.700 | 1.150 | 4.997 | 0.949 | 0.020 | 0.020 | 1.000 | 1.752 | 1.000 |
| 1.700 | 1.300 | 5.926 | 0.996 | 0.000 | 0.000 | 1.000 | 0.079 | 1.000 |
| 1.700 | 1.500 | 7.475 | 1.089 | 0.000 | 0.000 | 1.000 | 0.000 | 1.000 |
| 1.700 | 1.700 | 9.533 | 1.225 | 0.000 | 0.000 | 1.000 | 0.000 | 1.000 |
| 2.000 | 0.300 | 1.569 | 0.971 | 1.000 | 1.000 | 0.000 | 1.000 | 0.000 |
| 2.000 | 0.500 | 2.609 | 0.969 | 1.000 | 1.000 | 0.000 | 1.000 | 0.000 |
| 2.000 | 0.700 | 3.695 | 0.980 | 0.994 | 1.000 | 0.000 | 1.000 | 1.386 |
| 2.000 | 0.850 | 4.577 | 1.000 | 0.853 | 1.000 | 0.178 | 1.000 | 3.554 |
| 2.000 | 0.950 | 5.221 | 1.021 | 0.514 | 1.000 | 1.000 | 1.010 | 1.119 |
| 2.000 | 1.050 | 5.909 | 1.045 | 0.152 | 0.911 | 1.000 | 1.337 | 1.000 |
| 2.000 | 1.150 | 6.682 | 1.079 | 0.015 | 0.000 | 1.000 | 1.772 | 1.000 |
| 2.000 | 1.300 | 7.978 | 1.140 | 0.000 | 0.000 | 1.000 | 0.000 | 1.000 |
| 2.000 | 1.500 | 10.124 | 1.253 | 0.000 | 0.000 | 1.000 | 0.000 | 1.000 |
| 2.000 | 1.700 | 12.917 | 1.411 | 0.000 | 0.000 | 1.000 | 0.000 | 1.000 |
| 2.500 | 0.300 | 2.037 | 1.009 | 1.000 | 1.000 | 0.000 | 1.000 | 0.000 |
| 2.500 | 0.500 | 3.465 | 1.030 | 1.000 | 1.000 | 0.000 | 1.000 | 0.000 |
| 2.500 | 0.700 | 5.022 | 1.066 | 0.996 | 1.000 | 0.000 | 1.000 | 0.941 |
| 2.500 | 0.850 | 6.316 | 1.104 | 0.872 | 1.000 | 0.119 | 1.000 | 3.743 |
| 2.500 | 0.950 | 7.262 | 1.136 | 0.529 | 1.000 | 1.000 | 1.000 | 1.178 |
| 2.500 | 1.050 | 8.292 | 1.173 | 0.145 | 0.832 | 1.000 | 1.327 | 1.000 |
| 2.500 | 1.150 | 9.414 | 1.216 | 0.013 | 0.010 | 1.000 | 1.644 | 1.000 |
| 2.500 | 1.300 | 11.329 | 1.295 | 0.000 | 0.000 | 1.000 | 0.010 | 1.000 |
| 2.500 | 1.500 | 14.460 | 1.432 | 0.000 | 0.000 | 1.000 | 0.000 | 1.000 |
| 2.500 | 1.700 | 18.325 | 1.601 | 0.000 | 0.000 | 1.000 | 0.000 | 1.000 |
| 3.000 | 0.300 | 2.502 | 1.032 | 1.000 | 1.000 | 0.000 | 1.000 | 0.000 |
| 3.000 | 0.500 | 4.319 | 1.069 | 1.000 | 1.000 | 0.000 | 1.000 | 0.010 |
| 3.000 | 0.700 | 6.341 | 1.121 | 0.997 | 1.000 | 0.000 | 1.000 | 0.822 |
| 3.000 | 0.850 | 8.034 | 1.170 | 0.881 | 1.000 | 0.099 | 1.000 | 3.980 |
| 3.000 | 0.950 | 9.274 | 1.209 | 0.537 | 1.000 | 1.000 | 1.010 | 1.228 |
| 3.000 | 1.050 | 10.612 | 1.251 | 0.142 | 0.762 | 1.000 | 1.307 | 1.000 |
| 3.000 | 1.150 | 12.116 | 1.304 | 0.010 | 0.000 | 1.000 | 1.446 | 1.000 |
| 3.000 | 1.300 | 14.609 | 1.391 | 0.000 | 0.000 | 1.000 | 0.010 | 1.000 |
| 3.000 | 1.500 | 18.615 | 1.536 | 0.000 | 0.000 | 1.000 | 0.000 | 1.000 |
| 3.000 | 1.700 | 23.619 | 1.720 | 0.000 | 0.000 | 1.000 | 0.000 | 1.000 |
| 3.500 | 0.300 | 2.965 | 1.049 | 1.000 | 1.000 | 0.000 | 1.000 | 0.000 |
| 3.500 | 0.500 | 5.166 | 1.096 | 1.000 | 1.000 | 0.000 | 1.000 | 0.010 |
| 3.500 | 0.700 | 7.632 | 1.157 | 0.997 | 1.000 | 0.000 | 1.000 | 0.871 |
| 3.500 | 0.850 | 9.715 | 1.213 | 0.891 | 1.000 | 0.099 | 1.000 | 4.158 |
| 3.500 | 0.950 | 11.260 | 1.258 | 0.539 | 1.000 | 1.000 | 1.000 | 1.188 |
| 3.500 | 1.050 | 12.929 | 1.307 | 0.137 | 0.792 | 1.000 | 1.396 | 1.000 |
| 3.500 | 1.150 | 14.747 | 1.361 | 0.010 | 0.000 | 1.000 | 1.356 | 1.000 |
| 3.500 | 1.300 | 17.837 | 1.456 | 0.000 | 0.000 | 1.000 | 0.000 | 1.000 |
| 3.500 | 1.500 | 22.716 | 1.607 | 0.000 | 0.000 | 1.000 | 0.000 | 1.000 |
| 3.500 | 1.700 | 28.748 | 1.794 | 0.000 | 0.000 | 1.000 | 0.000 | 1.000 |

TABLE s19: Thermodynamic and structural properties of oxygen

| $T/T_c$ | $\rho/\rho_c$ | $p/p_c$ | $z$ | $\Pi_{gas}$ | $p^{gas}_{inf}$ | $p^{liq}_{inf}$ | $\langle n_c^{gas}\rangle$ | $\langle n_c^{liq}\rangle$ |
|---|---|---|---|---|---|---|---|---|
| 1.000 | 0.500 | 0.846 | 0.603 | 0.996 | 1.000 | 0.000 | 1.000 | 0.743 |
| 1.000 | 0.600 | 0.911 | 0.542 | 0.969 | 1.000 | 0.000 | 1.000 | 2.683 |
| 1.000 | 0.700 | 0.957 | 0.488 | 0.881 | 1.000 | 0.000 | 1.000 | 3.149 |
| 1.000 | 0.800 | 0.985 | 0.439 | 0.705 | 1.000 | 0.416 | 1.000 | 1.693 |
| 1.000 | 0.900 | 1.001 | 0.397 | 0.501 | 1.000 | 0.990 | 1.000 | 1.168 |
| 1.000 | 1.000 | 1.009 | 0.360 | 0.294 | 1.000 | 1.000 | 1.020 | 1.020 |
| 1.000 | 1.100 | 1.012 | 0.328 | 0.126 | 0.851 | 1.000 | 1.079 | 1.000 |
| 1.000 | 1.200 | 1.022 | 0.304 | 0.043 | 0.218 | 1.000 | 1.406 | 1.000 |
| 1.000 | 1.300 | 1.041 | 0.286 | 0.008 | 0.010 | 1.000 | 0.891 | 1.000 |
| 1.000 | 1.400 | 1.058 | 0.270 | 0.001 | 0.000 | 1.000 | 0.228 | 1.000 |
| 1.000 | 1.500 | 1.121 | 0.266 | 0.000 | 0.000 | 1.000 | 0.010 | 1.000 |
| 1.010 | 0.500 | 0.864 | 0.610 | 0.996 | 1.000 | 0.000 | 1.000 | 0.782 |
| 1.010 | 0.600 | 0.938 | 0.552 | 0.972 | 1.000 | 0.000 | 1.000 | 2.525 |
| 1.010 | 0.700 | 0.986 | 0.497 | 0.884 | 1.000 | 0.010 | 1.000 | 3.158 |
| 1.010 | 0.800 | 1.022 | 0.451 | 0.722 | 1.000 | 0.416 | 1.000 | 1.842 |
| 1.010 | 0.900 | 1.044 | 0.410 | 0.510 | 1.000 | 0.951 | 1.000 | 1.129 |
| 1.010 | 1.000 | 1.066 | 0.376 | 0.293 | 1.000 | 1.000 | 1.000 | 1.000 |
| 1.010 | 1.100 | 1.073 | 0.345 | 0.131 | 0.871 | 1.000 | 1.178 | 1.000 |
| 1.010 | 1.200 | 1.101 | 0.324 | 0.041 | 0.158 | 1.000 | 1.426 | 1.000 |
| 1.010 | 1.300 | 1.111 | 0.302 | 0.006 | 0.010 | 1.000 | 0.931 | 1.000 |
| 1.010 | 1.400 | 1.155 | 0.291 | 0.001 | 0.000 | 1.000 | 0.198 | 1.000 |
| 1.010 | 1.500 | 1.231 | 0.290 | 0.000 | 0.000 | 1.000 | 0.000 | 1.000 |
| 1.050 | 0.250 | 0.592 | 0.804 | 1.000 | 1.000 | 0.000 | 1.000 | 0.000 |
| 1.050 | 0.450 | 0.890 | 0.672 | 0.999 | 1.000 | 0.000 | 1.000 | 0.178 |
| 1.050 | 0.650 | 1.077 | 0.563 | 0.962 | 1.000 | 0.000 | 1.000 | 3.119 |
| 1.050 | 0.830 | 1.182 | 0.484 | 0.700 | 1.000 | 0.782 | 1.000 | 1.545 |
| 1.050 | 0.930 | 1.232 | 0.450 | 0.459 | 1.000 | 1.000 | 1.010 | 1.129 |
| 1.050 | 1.030 | 1.276 | 0.421 | 0.234 | 1.000 | 1.000 | 1.079 | 1.010 |
| 1.050 | 1.130 | 1.314 | 0.395 | 0.087 | 0.525 | 1.000 | 1.396 | 1.000 |
| 1.050 | 1.250 | 1.373 | 0.373 | 0.012 | 0.040 | 1.000 | 1.149 | 1.000 |
| 1.050 | 1.450 | 1.546 | 0.362 | 0.000 | 0.000 | 1.000 | 0.030 | 1.000 |
| 1.050 | 1.650 | 1.913 | 0.394 | 0.000 | 0.000 | 1.000 | 0.000 | 1.000 |
| 1.100 | 0.250 | 0.635 | 0.823 | 1.000 | 1.000 | 0.000 | 1.000 | 0.000 |
| 1.100 | 0.450 | 0.980 | 0.706 | 1.000 | 1.000 | 0.000 | 1.000 | 0.040 |
| 1.100 | 0.650 | 1.217 | 0.607 | 0.972 | 1.000 | 0.000 | 1.000 | 2.802 |
| 1.100 | 0.830 | 1.381 | 0.539 | 0.735 | 1.000 | 0.683 | 1.000 | 1.881 |
| 1.100 | 0.930 | 1.458 | 0.508 | 0.479 | 1.000 | 1.000 | 1.000 | 1.069 |
| 1.100 | 1.030 | 1.538 | 0.484 | 0.229 | 1.000 | 1.000 | 1.059 | 1.010 |
| 1.100 | 1.130 | 1.623 | 0.466 | 0.075 | 0.396 | 1.000 | 1.485 | 1.000 |
| 1.100 | 1.250 | 1.740 | 0.451 | 0.010 | 0.000 | 1.000 | 0.931 | 1.000 |
| 1.100 | 1.450 | 2.023 | 0.452 | 0.000 | 0.000 | 1.000 | 0.000 | 1.000 |
| 1.100 | 1.650 | 2.529 | 0.497 | 0.000 | 0.000 | 1.000 | 0.000 | 1.000 |
| 1.150 | 0.250 | 0.677 | 0.840 | 1.000 | 1.000 | 0.000 | 1.000 | 0.000 |
| 1.150 | 0.450 | 1.065 | 0.734 | 1.000 | 1.000 | 0.000 | 1.000 | 0.020 |
| 1.150 | 0.650 | 1.358 | 0.648 | 0.978 | 1.000 | 0.000 | 1.000 | 2.455 |
| 1.150 | 0.830 | 1.576 | 0.589 | 0.757 | 1.000 | 0.713 | 1.000 | 2.119 |
| 1.150 | 0.930 | 1.688 | 0.563 | 0.497 | 1.000 | 1.000 | 1.000 | 1.198 |
| 1.150 | 1.030 | 1.802 | 0.543 | 0.228 | 0.990 | 1.000 | 1.139 | 1.010 |
| 1.150 | 1.130 | 1.920 | 0.527 | 0.068 | 0.277 | 1.000 | 1.723 | 1.000 |
| 1.150 | 1.250 | 2.110 | 0.523 | 0.007 | 0.000 | 1.000 | 0.733 | 1.000 |
| 1.150 | 1.450 | 2.491 | 0.533 | 0.000 | 0.000 | 1.000 | 0.000 | 1.000 |
| 1.150 | 1.650 | 3.136 | 0.589 | 0.000 | 0.000 | 1.000 | 0.000 | 1.000 |
| 1.200 | 0.250 | 0.718 | 0.853 | 1.000 | 1.000 | 0.000 | 1.000 | 0.000 |
| 1.200 | 0.450 | 1.148 | 0.758 | 1.000 | 1.000 | 0.000 | 1.000 | 0.020 |
| 1.200 | 0.650 | 1.492 | 0.682 | 0.982 | 1.000 | 0.000 | 1.000 | 2.129 |
| 1.200 | 0.830 | 1.760 | 0.630 | 0.783 | 1.000 | 0.515 | 1.000 | 2.475 |
| 1.200 | 0.930 | 1.905 | 0.609 | 0.509 | 1.000 | 1.000 | 1.000 | 1.248 |
| 1.200 | 1.030 | 2.063 | 0.595 | 0.229 | 1.000 | 1.000 | 1.109 | 1.010 |
| 1.200 | 1.130 | 2.227 | 0.586 | 0.061 | 0.248 | 1.000 | 1.752 | 1.000 |
| 1.200 | 1.250 | 2.457 | 0.584 | 0.004 | 0.000 | 1.000 | 0.624 | 1.000 |

*Continued on next page*

TABLE s19 – Thermodynamic and structural properties of oxygen (continued)

| $T/T_c$ | $\rho/\rho_c$ | $p/p_c$ | $z$ | $\Pi_{gas}$ | $p_{inf}^{gas}$ | $p_{inf}^{liq}$ | $\langle n_c^{gas}\rangle$ | $\langle n_c^{liq}\rangle$ |
|---|---|---|---|---|---|---|---|---|
| 1.200 | 1.450 | 2.973 | 0.609 | 0.000 | 0.000 | 1.000 | 0.000 | 1.000 |
| 1.200 | 1.650 | 3.759 | 0.677 | 0.000 | 0.000 | 1.000 | 0.000 | 1.000 |
| 1.250 | 0.250 | 0.761 | 0.868 | 1.000 | 1.000 | 0.000 | 1.000 | 0.000 |
| 1.250 | 0.450 | 1.233 | 0.782 | 1.000 | 1.000 | 0.000 | 1.000 | 0.010 |
| 1.250 | 0.650 | 1.627 | 0.714 | 0.990 | 1.000 | 0.000 | 1.000 | 1.673 |
| 1.250 | 0.830 | 1.954 | 0.672 | 0.792 | 1.000 | 0.436 | 1.000 | 2.604 |
| 1.250 | 0.930 | 2.136 | 0.655 | 0.520 | 1.000 | 1.000 | 1.000 | 1.129 |
| 1.250 | 1.030 | 2.323 | 0.643 | 0.222 | 1.000 | 1.000 | 1.119 | 1.000 |
| 1.250 | 1.130 | 2.539 | 0.641 | 0.052 | 0.208 | 1.000 | 1.842 | 1.000 |
| 1.250 | 1.250 | 2.807 | 0.641 | 0.003 | 0.000 | 1.000 | 0.535 | 1.000 |
| 1.250 | 1.450 | 3.420 | 0.673 | 0.000 | 0.000 | 1.000 | 0.000 | 1.000 |
| 1.250 | 1.650 | 4.378 | 0.757 | 0.000 | 0.000 | 1.000 | 0.000 | 1.000 |
| 1.300 | 0.250 | 0.802 | 0.880 | 1.000 | 1.000 | 0.000 | 1.000 | 0.000 |
| 1.300 | 0.450 | 1.319 | 0.804 | 1.000 | 1.000 | 0.000 | 1.000 | 0.000 |
| 1.300 | 0.650 | 1.764 | 0.744 | 0.991 | 1.000 | 0.000 | 1.000 | 1.455 |
| 1.300 | 0.830 | 2.146 | 0.709 | 0.808 | 1.000 | 0.347 | 1.000 | 2.782 |
| 1.300 | 0.930 | 2.359 | 0.696 | 0.532 | 1.000 | 1.000 | 1.000 | 1.158 |
| 1.300 | 1.030 | 2.584 | 0.688 | 0.225 | 1.000 | 1.000 | 1.158 | 1.010 |
| 1.300 | 1.130 | 2.837 | 0.689 | 0.051 | 0.208 | 1.000 | 1.822 | 1.000 |
| 1.300 | 1.250 | 3.162 | 0.694 | 0.003 | 0.000 | 1.000 | 0.446 | 1.000 |
| 1.300 | 1.450 | 3.909 | 0.740 | 0.000 | 0.000 | 1.000 | 0.000 | 1.000 |
| 1.300 | 1.650 | 5.002 | 0.832 | 0.000 | 0.000 | 1.000 | 0.000 | 1.000 |
| 2.300 | 0.250 | 1.614 | 1.001 | 1.000 | 1.000 | 0.000 | 1.000 | 0.000 |
| 2.300 | 0.450 | 2.954 | 1.018 | 1.000 | 1.000 | 0.000 | 1.000 | 0.000 |
| 2.300 | 0.650 | 4.401 | 1.050 | 0.999 | 1.000 | 0.000 | 1.000 | 0.297 |
| 2.300 | 0.830 | 5.847 | 1.092 | 0.915 | 1.000 | 0.020 | 1.000 | 4.297 |
| 2.300 | 0.930 | 6.741 | 1.124 | 0.616 | 1.000 | 1.000 | 1.010 | 1.307 |
| 2.300 | 1.030 | 7.708 | 1.160 | 0.202 | 0.980 | 1.000 | 1.129 | 1.020 |
| 2.300 | 1.130 | 8.794 | 1.207 | 0.022 | 0.020 | 1.000 | 1.683 | 1.000 |
| 2.300 | 1.250 | 10.243 | 1.271 | 0.000 | 0.000 | 1.000 | 0.337 | 1.000 |
| 2.300 | 1.450 | 13.170 | 1.408 | 0.000 | 0.000 | 1.000 | 0.000 | 1.000 |
| 2.300 | 1.650 | 16.946 | 1.592 | 0.000 | 0.000 | 1.000 | 0.000 | 1.000 |
| 2.600 | 0.250 | 1.855 | 1.018 | 1.000 | 1.000 | 0.000 | 1.000 | 0.000 |
| 2.600 | 0.450 | 3.433 | 1.046 | 1.000 | 1.000 | 0.000 | 1.000 | 0.000 |
| 2.600 | 0.650 | 5.163 | 1.089 | 1.000 | 1.000 | 0.000 | 1.000 | 0.208 |
| 2.600 | 0.830 | 6.930 | 1.145 | 0.915 | 1.000 | 0.059 | 1.000 | 4.238 |
| 2.600 | 0.930 | 8.023 | 1.183 | 0.623 | 1.000 | 0.990 | 1.000 | 1.356 |
| 2.600 | 1.030 | 9.216 | 1.227 | 0.199 | 0.980 | 1.000 | 1.426 | 1.000 |
| 2.600 | 1.130 | 10.552 | 1.281 | 0.019 | 0.010 | 1.000 | 1.337 | 1.000 |
| 2.600 | 1.250 | 12.330 | 1.353 | 0.000 | 0.000 | 1.000 | 0.089 | 1.000 |
| 2.600 | 1.450 | 15.893 | 1.503 | 0.000 | 0.000 | 1.000 | 0.000 | 1.000 |
| 2.600 | 1.650 | 20.389 | 1.695 | 0.000 | 0.000 | 1.000 | 0.000 | 1.000 |
| 3.300 | 0.250 | 2.414 | 1.043 | 1.000 | 1.000 | 0.000 | 1.000 | 0.000 |
| 3.300 | 0.450 | 4.545 | 1.091 | 1.000 | 1.000 | 0.000 | 1.000 | 0.000 |
| 3.300 | 0.650 | 6.952 | 1.156 | 1.000 | 1.000 | 0.000 | 1.000 | 0.139 |
| 3.300 | 0.830 | 9.437 | 1.229 | 0.932 | 1.000 | 0.000 | 1.000 | 4.257 |
| 3.300 | 0.930 | 10.975 | 1.275 | 0.637 | 1.000 | 0.990 | 1.000 | 1.515 |
| 3.300 | 1.030 | 12.677 | 1.330 | 0.200 | 0.990 | 1.000 | 1.495 | 1.000 |
| 3.300 | 1.130 | 14.556 | 1.392 | 0.016 | 0.010 | 1.000 | 1.198 | 1.000 |
| 3.300 | 1.250 | 17.048 | 1.474 | 0.000 | 0.000 | 1.000 | 0.050 | 1.000 |
| 3.300 | 1.450 | 22.007 | 1.640 | 0.000 | 0.000 | 1.000 | 0.000 | 1.000 |
| 3.300 | 1.650 | 28.211 | 1.848 | 0.000 | 0.000 | 1.000 | 0.000 | 1.000 |
| 3.400 | 0.250 | 2.493 | 1.046 | 1.000 | 1.000 | 0.000 | 1.000 | 0.000 |
| 3.400 | 0.450 | 4.707 | 1.097 | 1.000 | 1.000 | 0.000 | 1.000 | 0.000 |
| 3.400 | 0.650 | 7.204 | 1.162 | 0.999 | 1.000 | 0.000 | 1.000 | 0.188 |
| 3.400 | 0.830 | 9.783 | 1.236 | 0.931 | 1.000 | 0.020 | 1.000 | 4.218 |
| 3.400 | 0.930 | 11.403 | 1.286 | 0.643 | 1.000 | 0.990 | 1.000 | 1.396 |
| 3.400 | 1.030 | 13.168 | 1.341 | 0.199 | 0.980 | 1.000 | 1.485 | 1.000 |
| 3.400 | 1.130 | 15.107 | 1.402 | 0.016 | 0.000 | 1.000 | 1.050 | 1.000 |
| 3.400 | 1.250 | 17.704 | 1.486 | 0.000 | 0.000 | 1.000 | 0.010 | 1.000 |
| 3.400 | 1.450 | 22.865 | 1.654 | 0.000 | 0.000 | 1.000 | 0.000 | 1.000 |

*Continued on next page*

TABLE s19 – Thermodynamic and structural properties of oxygen (continued)

| $T/T_c$ | $\rho/\rho_c$ | $p/p_c$ | $z$ | $\Pi_{gas}$ | $p_{inf}^{gas}$ | $p_{inf}^{liq}$ | $\langle n_c^{gas}\rangle$ | $\langle n_c^{liq}\rangle$ |
|---|---|---|---|---|---|---|---|---|
| 3.400 | 1.650 | 29.328 | 1.864 | 0.000 | 0.000 | 1.000 | 0.000 | 1.000 |

TABLE s20: Thermodynamic and structural properties of carbon dioxide

| $T/T_c$ | $\rho/\rho_c$ | $p/p_c$ | $z$ | $\Pi_{gas}$ | $p_{inf}^{gas}$ | $p_{inf}^{liq}$ | $\langle n_c^{gas}\rangle$ | $\langle n_c^{liq}\rangle$ |
|---|---|---|---|---|---|---|---|---|
| 1.000 | 0.500 | 0.877 | 0.569 | 0.997 | 1.000 | 0.000 | 1.000 | 0.594 |
| 1.000 | 0.600 | 0.938 | 0.507 | 0.968 | 1.000 | 0.000 | 1.000 | 2.881 |
| 1.000 | 0.700 | 0.968 | 0.448 | 0.839 | 1.000 | 0.050 | 1.000 | 2.772 |
| 1.000 | 0.800 | 0.988 | 0.401 | 0.708 | 1.000 | 0.436 | 1.000 | 1.842 |
| 1.000 | 0.900 | 0.999 | 0.360 | 0.496 | 1.000 | 0.970 | 1.000 | 1.168 |
| 1.000 | 1.000 | 1.004 | 0.326 | 0.280 | 1.000 | 1.000 | 1.000 | 1.010 |
| 1.000 | 1.100 | 0.998 | 0.294 | 0.128 | 0.931 | 1.000 | 1.099 | 1.000 |
| 1.000 | 1.200 | 1.005 | 0.272 | 0.038 | 0.168 | 1.000 | 1.426 | 1.000 |
| 1.000 | 1.300 | 1.033 | 0.258 | 0.007 | 0.030 | 1.000 | 0.921 | 1.000 |
| 1.000 | 1.400 | 1.058 | 0.245 | 0.001 | 0.000 | 1.000 | 0.277 | 1.000 |
| 1.000 | 1.500 | 1.152 | 0.249 | 0.000 | 0.000 | 1.000 | 0.010 | 1.000 |
| 1.010 | 0.500 | 0.903 | 0.580 | 0.993 | 1.000 | 0.000 | 1.000 | 0.980 |
| 1.010 | 0.600 | 0.969 | 0.519 | 0.973 | 1.000 | 0.000 | 1.000 | 2.525 |
| 1.010 | 0.700 | 1.012 | 0.464 | 0.879 | 1.000 | 0.010 | 1.000 | 3.178 |
| 1.010 | 0.800 | 1.037 | 0.416 | 0.696 | 1.000 | 0.525 | 1.000 | 1.455 |
| 1.010 | 0.900 | 1.061 | 0.378 | 0.487 | 1.000 | 1.000 | 1.010 | 1.119 |
| 1.010 | 1.000 | 1.067 | 0.343 | 0.289 | 1.000 | 1.000 | 1.010 | 1.020 |
| 1.010 | 1.100 | 1.075 | 0.314 | 0.115 | 0.851 | 1.000 | 1.129 | 1.000 |
| 1.010 | 1.200 | 1.092 | 0.292 | 0.030 | 0.050 | 1.000 | 1.644 | 1.000 |
| 1.010 | 1.300 | 1.114 | 0.275 | 0.010 | 0.000 | 1.000 | 1.287 | 1.000 |
| 1.010 | 1.400 | 1.173 | 0.269 | 0.000 | 0.000 | 1.000 | 0.168 | 1.000 |
| 1.010 | 1.500 | 1.276 | 0.273 | 0.000 | 0.000 | 1.000 | 0.000 | 1.000 |
| 1.050 | 0.200 | 0.538 | 0.831 | 1.000 | 1.000 | 0.000 | 1.000 | 0.000 |
| 1.050 | 0.400 | 0.883 | 0.682 | 1.000 | 1.000 | 0.000 | 1.000 | 0.000 |
| 1.050 | 0.600 | 1.099 | 0.566 | 0.984 | 1.000 | 0.000 | 1.000 | 2.109 |
| 1.050 | 0.800 | 1.232 | 0.476 | 0.738 | 1.000 | 0.525 | 1.000 | 1.950 |
| 1.050 | 0.900 | 1.284 | 0.441 | 0.531 | 1.000 | 1.000 | 1.000 | 1.109 |
| 1.050 | 1.000 | 1.332 | 0.411 | 0.303 | 1.000 | 1.000 | 1.000 | 1.000 |
| 1.050 | 1.100 | 1.383 | 0.388 | 0.120 | 0.871 | 1.000 | 1.139 | 1.000 |
| 1.050 | 1.200 | 1.432 | 0.369 | 0.026 | 0.010 | 1.000 | 1.416 | 1.000 |
| 1.050 | 1.400 | 1.644 | 0.363 | 0.000 | 0.000 | 1.000 | 0.020 | 1.000 |
| 1.050 | 1.600 | 2.059 | 0.398 | 0.000 | 0.000 | 1.000 | 0.000 | 1.000 |
| 1.050 | 1.800 | 3.025 | 0.519 | 0.000 | 0.000 | 1.000 | 0.000 | 1.000 |
| 1.050 | 2.000 | 4.868 | 0.752 | 0.000 | 0.000 | 1.000 | 0.000 | 1.000 |
| 1.100 | 0.200 | 0.574 | 0.846 | 1.000 | 1.000 | 0.000 | 1.000 | 0.000 |
| 1.100 | 0.400 | 0.978 | 0.721 | 1.000 | 1.000 | 0.000 | 1.000 | 0.010 |
| 1.100 | 0.600 | 1.244 | 0.611 | 0.993 | 1.000 | 0.000 | 1.000 | 1.327 |
| 1.100 | 0.800 | 1.456 | 0.537 | 0.804 | 1.000 | 0.347 | 1.000 | 2.663 |
| 1.100 | 0.900 | 1.565 | 0.513 | 0.589 | 1.000 | 1.000 | 1.000 | 1.198 |
| 1.100 | 1.000 | 1.633 | 0.481 | 0.297 | 1.000 | 1.000 | 1.000 | 1.010 |
| 1.100 | 1.100 | 1.722 | 0.462 | 0.096 | 0.574 | 1.000 | 1.257 | 1.000 |
| 1.100 | 1.200 | 1.853 | 0.455 | 0.027 | 0.059 | 1.000 | 1.535 | 1.000 |
| 1.100 | 1.400 | 2.192 | 0.462 | 0.000 | 0.000 | 1.000 | 0.079 | 1.000 |
| 1.100 | 1.600 | 2.891 | 0.533 | 0.000 | 0.000 | 1.000 | 0.000 | 1.000 |
| 1.100 | 1.800 | 4.089 | 0.670 | 0.000 | 0.000 | 1.000 | 0.000 | 1.000 |
| 1.100 | 2.000 | 6.319 | 0.932 | 0.000 | 0.000 | 1.000 | 0.000 | 1.000 |
| 1.150 | 0.200 | 0.610 | 0.860 | 1.000 | 1.000 | 0.000 | 1.000 | 0.000 |
| 1.150 | 0.400 | 1.060 | 0.747 | 1.000 | 1.000 | 0.000 | 1.000 | 0.000 |
| 1.150 | 0.600 | 1.408 | 0.662 | 0.996 | 1.000 | 0.000 | 1.000 | 0.980 |
| 1.150 | 0.800 | 1.690 | 0.596 | 0.822 | 1.000 | 0.366 | 1.000 | 2.525 |
| 1.150 | 0.900 | 1.827 | 0.573 | 0.594 | 1.000 | 1.000 | 1.000 | 1.277 |
| 1.150 | 1.000 | 1.969 | 0.555 | 0.302 | 1.000 | 1.000 | 1.030 | 1.020 |
| 1.150 | 1.100 | 2.095 | 0.537 | 0.100 | 0.614 | 1.000 | 1.406 | 1.000 |
| 1.150 | 1.200 | 2.292 | 0.539 | 0.014 | 0.020 | 1.000 | 1.545 | 1.000 |

*Continued on next page*

TABLE s20 – Thermodynamic and structural properties of carbon dioxide (continued)

| $T/T_c$ | $\rho/\rho_c$ | $p/p_c$ | $z$ | $\Pi_{gas}$ | $p_{inf}^{gas}$ | $p_{inf}^{liq}$ | $\langle n_c^{gas}\rangle$ | $\langle n_c^{liq}\rangle$ |
|---|---|---|---|---|---|---|---|---|
| 1.150 | 1.400 | 2.804 | 0.565 | 0.000 | 0.000 | 1.000 | 0.050 | 1.000 |
| 1.150 | 1.600 | 3.612 | 0.637 | 0.000 | 0.000 | 1.000 | 0.000 | 1.000 |
| 1.150 | 1.800 | 5.117 | 0.802 | 0.000 | 0.000 | 1.000 | 0.000 | 1.000 |
| 1.150 | 2.000 | 7.689 | 1.084 | 0.000 | 0.000 | 1.000 | 0.000 | 1.000 |
| 1.200 | 0.200 | 0.649 | 0.877 | 1.000 | 1.000 | 0.000 | 1.000 | 0.000 |
| 1.200 | 0.400 | 1.159 | 0.783 | 1.000 | 1.000 | 0.000 | 1.000 | 0.000 |
| 1.200 | 0.600 | 1.557 | 0.701 | 0.997 | 1.000 | 0.000 | 1.000 | 0.782 |
| 1.200 | 0.800 | 1.919 | 0.648 | 0.852 | 1.000 | 0.099 | 1.000 | 3.069 |
| 1.200 | 0.900 | 2.101 | 0.631 | 0.613 | 1.000 | 1.000 | 1.000 | 1.238 |
| 1.200 | 1.000 | 2.272 | 0.614 | 0.302 | 1.000 | 1.000 | 1.000 | 1.010 |
| 1.200 | 1.100 | 2.472 | 0.607 | 0.092 | 0.475 | 1.000 | 1.317 | 1.010 |
| 1.200 | 1.200 | 2.755 | 0.621 | 0.014 | 0.030 | 1.000 | 1.455 | 1.000 |
| 1.200 | 1.400 | 3.384 | 0.653 | 0.000 | 0.000 | 1.000 | 0.010 | 1.000 |
| 1.200 | 1.600 | 4.465 | 0.754 | 0.000 | 0.000 | 1.000 | 0.000 | 1.000 |
| 1.200 | 1.800 | 6.143 | 0.922 | 0.000 | 0.000 | 1.000 | 0.000 | 1.000 |
| 1.200 | 2.000 | 9.050 | 1.223 | 0.000 | 0.000 | 1.000 | 0.000 | 1.000 |
| 1.250 | 0.200 | 0.689 | 0.894 | 1.000 | 1.000 | 0.000 | 1.000 | 0.000 |
| 1.250 | 0.400 | 1.244 | 0.807 | 1.000 | 1.000 | 0.000 | 1.000 | 0.000 |
| 1.250 | 0.600 | 1.695 | 0.733 | 0.997 | 1.000 | 0.000 | 1.000 | 0.614 |
| 1.250 | 0.800 | 2.139 | 0.694 | 0.863 | 1.000 | 0.139 | 1.000 | 3.307 |
| 1.250 | 0.900 | 2.350 | 0.678 | 0.629 | 1.000 | 0.980 | 1.000 | 1.218 |
| 1.250 | 1.000 | 2.593 | 0.673 | 0.305 | 1.000 | 1.000 | 1.059 | 1.030 |
| 1.250 | 1.100 | 2.848 | 0.672 | 0.074 | 0.347 | 1.000 | 1.673 | 1.000 |
| 1.250 | 1.200 | 3.168 | 0.685 | 0.010 | 0.000 | 1.000 | 1.347 | 1.000 |
| 1.250 | 1.400 | 3.957 | 0.733 | 0.000 | 0.000 | 1.000 | 0.020 | 1.000 |
| 1.250 | 1.600 | 5.164 | 0.837 | 0.000 | 0.000 | 1.000 | 0.000 | 1.000 |
| 1.250 | 1.800 | 7.195 | 1.037 | 0.000 | 0.000 | 1.000 | 0.000 | 1.000 |
| 1.250 | 2.000 | 10.377 | 1.346 | 0.000 | 0.000 | 1.000 | 0.000 | 1.000 |
| 1.300 | 0.200 | 0.725 | 0.904 | 1.000 | 1.000 | 0.000 | 1.000 | 0.000 |
| 1.300 | 0.400 | 1.328 | 0.828 | 1.000 | 1.000 | 0.000 | 1.000 | 0.000 |
| 1.300 | 0.600 | 1.851 | 0.770 | 0.999 | 1.000 | 0.000 | 1.000 | 0.238 |
| 1.300 | 0.800 | 2.368 | 0.738 | 0.895 | 1.000 | 0.010 | 1.000 | 3.554 |
| 1.300 | 0.900 | 2.621 | 0.727 | 0.649 | 1.000 | 0.921 | 1.000 | 1.426 |
| 1.300 | 1.000 | 2.911 | 0.726 | 0.313 | 1.000 | 1.000 | 1.020 | 1.010 |
| 1.300 | 1.100 | 3.245 | 0.736 | 0.071 | 0.376 | 1.000 | 1.703 | 1.000 |
| 1.300 | 1.200 | 3.618 | 0.752 | 0.004 | 0.000 | 1.000 | 1.020 | 1.000 |
| 1.300 | 1.400 | 4.559 | 0.812 | 0.000 | 0.000 | 1.000 | 0.000 | 1.000 |
| 1.300 | 1.600 | 5.970 | 0.931 | 0.000 | 0.000 | 1.000 | 0.000 | 1.000 |
| 1.300 | 1.800 | 8.160 | 1.131 | 0.000 | 0.000 | 1.000 | 0.000 | 1.000 |
| 1.300 | 2.000 | 11.711 | 1.461 | 0.000 | 0.000 | 1.000 | 0.000 | 1.000 |
| 1.900 | 0.200 | 1.157 | 0.988 | 1.000 | 1.000 | 0.000 | 1.000 | 0.000 |
| 1.900 | 0.400 | 2.315 | 0.988 | 1.000 | 1.000 | 0.000 | 1.000 | 0.000 |
| 1.900 | 0.600 | 3.555 | 1.011 | 1.000 | 1.000 | 0.000 | 1.000 | 0.030 |
| 1.900 | 0.800 | 4.970 | 1.061 | 0.954 | 1.000 | 0.000 | 1.000 | 3.535 |
| 1.900 | 0.900 | 5.742 | 1.089 | 0.735 | 1.000 | 0.842 | 1.000 | 1.950 |
| 1.900 | 1.000 | 6.588 | 1.125 | 0.321 | 1.000 | 1.000 | 1.030 | 1.010 |
| 1.900 | 1.100 | 7.548 | 1.171 | 0.045 | 0.079 | 1.000 | 2.000 | 1.000 |
| 1.900 | 1.200 | 8.655 | 1.231 | 0.001 | 0.000 | 1.000 | 0.416 | 1.000 |
| 1.900 | 1.400 | 11.431 | 1.394 | 0.000 | 0.000 | 1.000 | 0.000 | 1.000 |
| 1.900 | 1.600 | 15.103 | 1.611 | 0.000 | 0.000 | 1.000 | 0.000 | 1.000 |
| 1.900 | 1.800 | 20.116 | 1.908 | 0.000 | 0.000 | 1.000 | 0.000 | 1.000 |
| 1.900 | 2.000 | 27.043 | 2.308 | 0.000 | 0.000 | 1.000 | 0.000 | 1.000 |
| 2.200 | 0.200 | 1.372 | 1.011 | 1.000 | 1.000 | 0.000 | 1.000 | 0.000 |
| 2.200 | 0.400 | 2.805 | 1.034 | 1.000 | 1.000 | 0.000 | 1.000 | 0.000 |
| 2.200 | 0.600 | 4.397 | 1.080 | 1.000 | 1.000 | 0.000 | 1.000 | 0.040 |
| 2.200 | 0.800 | 6.220 | 1.146 | 0.968 | 1.000 | 0.000 | 1.000 | 3.277 |
| 2.200 | 0.900 | 7.246 | 1.187 | 0.759 | 1.000 | 0.713 | 1.000 | 1.990 |
| 2.200 | 1.000 | 8.365 | 1.233 | 0.327 | 1.000 | 1.000 | 1.059 | 1.030 |
| 2.200 | 1.100 | 9.674 | 1.297 | 0.043 | 0.040 | 1.000 | 2.040 | 1.000 |
| 2.200 | 1.200 | 11.148 | 1.370 | 0.001 | 0.000 | 1.000 | 0.386 | 1.000 |
| 2.200 | 1.400 | 14.599 | 1.537 | 0.000 | 0.000 | 1.000 | 0.000 | 1.000 |

*Continued on next page*

TABLE s20 – Thermodynamic and structural properties of carbon dioxide (continued)

| $T/T_c$ | $\rho/\rho_c$ | $p/p_c$ | $z$ | $\Pi_{gas}$ | $p^{gas}_{inf}$ | $p^{liq}_{inf}$ | $\langle n^{gas}_c \rangle$ | $\langle n^{liq}_c \rangle$ |
|---|---|---|---|---|---|---|---|---|
| 2.200 | 1.600 | 19.377 | 1.785 | 0.000 | 0.000 | 1.000 | 0.000 | 1.000 |
| 2.200 | 1.800 | 25.605 | 2.097 | 0.000 | 0.000 | 1.000 | 0.000 | 1.000 |
| 2.200 | 2.000 | 34.246 | 2.524 | 0.000 | 0.000 | 1.000 | 0.000 | 1.000 |
| 2.700 | 0.200 | 1.721 | 1.034 | 1.000 | 1.000 | 0.000 | 1.000 | 0.000 |
| 2.700 | 0.400 | 3.596 | 1.080 | 1.000 | 1.000 | 0.000 | 1.000 | 0.000 |
| 2.700 | 0.600 | 5.771 | 1.155 | 1.000 | 1.000 | 0.000 | 1.000 | 0.010 |
| 2.700 | 0.800 | 8.261 | 1.240 | 0.966 | 1.000 | 0.000 | 1.000 | 3.099 |
| 2.700 | 0.900 | 9.699 | 1.295 | 0.778 | 1.000 | 0.525 | 1.000 | 2.139 |
| 2.700 | 1.000 | 11.342 | 1.362 | 0.321 | 1.000 | 1.000 | 1.020 | 1.010 |
| 2.700 | 1.100 | 13.134 | 1.434 | 0.037 | 0.069 | 1.000 | 2.050 | 1.000 |
| 2.700 | 1.200 | 15.161 | 1.518 | 0.001 | 0.000 | 1.000 | 0.277 | 1.000 |
| 2.700 | 1.400 | 20.035 | 1.719 | 0.000 | 0.000 | 1.000 | 0.000 | 1.000 |
| 2.700 | 1.600 | 26.449 | 1.986 | 0.000 | 0.000 | 1.000 | 0.000 | 1.000 |
| 2.700 | 1.800 | 34.806 | 2.323 | 0.000 | 0.000 | 1.000 | 0.000 | 1.000 |
| 2.700 | 2.000 | 45.702 | 2.745 | 0.000 | 0.000 | 1.000 | 0.000 | 1.000 |
| 3.200 | 0.200 | 2.072 | 1.050 | 1.000 | 1.000 | 0.000 | 1.000 | 0.000 |
| 3.200 | 0.400 | 4.392 | 1.113 | 1.000 | 1.000 | 0.000 | 1.000 | 0.000 |
| 3.200 | 0.600 | 7.079 | 1.196 | 1.000 | 1.000 | 0.000 | 1.000 | 0.000 |
| 3.200 | 0.800 | 10.309 | 1.306 | 0.980 | 1.000 | 0.000 | 1.000 | 2.861 |
| 3.200 | 0.900 | 12.118 | 1.365 | 0.780 | 1.000 | 0.663 | 1.000 | 2.188 |
| 3.200 | 1.000 | 14.182 | 1.437 | 0.327 | 1.000 | 1.000 | 1.010 | 1.020 |
| 3.200 | 1.100 | 16.482 | 1.519 | 0.031 | 0.040 | 1.000 | 2.149 | 1.000 |
| 3.200 | 1.200 | 19.084 | 1.612 | 0.001 | 0.000 | 1.000 | 0.238 | 1.000 |
| 3.200 | 1.400 | 25.244 | 1.828 | 0.000 | 0.000 | 1.000 | 0.000 | 1.000 |
| 3.200 | 1.600 | 33.261 | 2.107 | 0.000 | 0.000 | 1.000 | 0.000 | 1.000 |
| 3.200 | 1.800 | 43.451 | 2.447 | 0.000 | 0.000 | 1.000 | 0.000 | 1.000 |
| 3.200 | 2.000 | 56.810 | 2.879 | 0.000 | 0.000 | 1.000 | 0.000 | 1.000 |
| 3.400 | 0.200 | 2.211 | 1.055 | 1.000 | 1.000 | 0.000 | 1.000 | 0.000 |
| 3.400 | 0.400 | 4.714 | 1.124 | 1.000 | 1.000 | 0.000 | 1.000 | 0.000 |
| 3.400 | 0.600 | 7.617 | 1.211 | 1.000 | 1.000 | 0.000 | 1.000 | 0.000 |
| 3.400 | 0.800 | 11.106 | 1.324 | 0.977 | 1.000 | 0.000 | 1.000 | 3.010 |
| 3.400 | 0.900 | 13.104 | 1.389 | 0.786 | 1.000 | 0.693 | 1.000 | 2.455 |
| 3.400 | 1.000 | 15.310 | 1.460 | 0.333 | 1.000 | 1.000 | 1.020 | 1.040 |
| 3.400 | 1.100 | 17.859 | 1.549 | 0.033 | 0.069 | 1.000 | 2.188 | 1.000 |
| 3.400 | 1.200 | 20.635 | 1.640 | 0.001 | 0.000 | 1.000 | 0.198 | 1.000 |
| 3.400 | 1.400 | 27.305 | 1.861 | 0.000 | 0.000 | 1.000 | 0.000 | 1.000 |
| 3.400 | 1.600 | 35.844 | 2.137 | 0.000 | 0.000 | 1.000 | 0.000 | 1.000 |
| 3.400 | 1.800 | 46.970 | 2.489 | 0.000 | 0.000 | 1.000 | 0.000 | 1.000 |
| 3.400 | 2.000 | 60.908 | 2.905 | 0.000 | 0.000 | 1.000 | 0.000 | 1.000 |
| 3.500 | 0.200 | 2.277 | 1.055 | 1.000 | 1.000 | 0.000 | 1.000 | 0.000 |
| 3.500 | 0.400 | 4.869 | 1.128 | 1.000 | 1.000 | 0.000 | 1.000 | 0.000 |
| 3.500 | 0.600 | 7.874 | 1.216 | 1.000 | 1.000 | 0.000 | 1.000 | 0.000 |
| 3.500 | 0.800 | 11.487 | 1.331 | 0.978 | 1.000 | 0.000 | 1.000 | 3.119 |
| 3.500 | 0.900 | 13.577 | 1.398 | 0.794 | 1.000 | 0.545 | 1.000 | 2.327 |
| 3.500 | 1.000 | 15.892 | 1.473 | 0.323 | 1.000 | 1.000 | 1.040 | 1.010 |
| 3.500 | 1.100 | 18.518 | 1.560 | 0.034 | 0.020 | 1.000 | 2.228 | 1.000 |
| 3.500 | 1.200 | 21.397 | 1.652 | 0.000 | 0.000 | 1.000 | 0.139 | 1.000 |
| 3.500 | 1.400 | 28.303 | 1.873 | 0.000 | 0.000 | 1.000 | 0.000 | 1.000 |
| 3.500 | 1.600 | 37.141 | 2.151 | 0.000 | 0.000 | 1.000 | 0.000 | 1.000 |
| 3.500 | 1.800 | 48.445 | 2.494 | 0.000 | 0.000 | 1.000 | 0.000 | 1.000 |
| 3.500 | 2.000 | 63.078 | 2.923 | 0.000 | 0.000 | 1.000 | 0.000 | 1.000 |

TABLE s21: Thermodynamic and structural properties of ethylene oxide

| $T/T_c$ | $\rho/\rho_c$ | $p/p_c$ | $z$ | $\Pi_{gas}$ | $p^{gas}_{inf}$ | $p^{liq}_{inf}$ | $\langle n^{gas}_c \rangle$ | $\langle n^{liq}_c \rangle$ |
|---|---|---|---|---|---|---|---|---|
| 1.000 | 0.500 | 0.863 | 0.527 | 0.988 | 1.000 | 0.000 | 1.000 | 1.535 |
| 1.000 | 0.600 | 0.922 | 0.469 | 0.936 | 1.000 | 0.000 | 1.000 | 3.109 |
| 1.000 | 0.700 | 0.962 | 0.419 | 0.839 | 1.000 | 0.020 | 1.000 | 3.168 |
| 1.000 | 0.800 | 0.997 | 0.380 | 0.661 | 1.000 | 0.337 | 1.000 | 1.584 |
| 1.000 | 0.900 | 1.001 | 0.339 | 0.450 | 1.000 | 0.990 | 1.000 | 1.119 |

*Continued on next page*

TABLE s21 – Thermodynamic and structural properties of ethylene oxide (continued)

| $T/T_c$ | $\rho/\rho_c$ | $p/p_c$ | $z$ | $\Pi_{gas}$ | $p_{inf}^{gas}$ | $p_{inf}^{liq}$ | $\langle n_c^{gas}\rangle$ | $\langle n_c^{liq}\rangle$ |
|---|---|---|---|---|---|---|---|---|
| 1.000 | 1.000 | 1.006 | 0.307 | 0.268 | 1.000 | 1.000 | 1.010 | 1.020 |
| 1.000 | 1.100 | 1.013 | 0.281 | 0.130 | 0.861 | 1.000 | 1.050 | 1.000 |
| 1.000 | 1.200 | 1.024 | 0.260 | 0.049 | 0.248 | 1.000 | 1.396 | 1.000 |
| 1.000 | 1.300 | 1.023 | 0.240 | 0.011 | 0.010 | 1.000 | 1.149 | 1.000 |
| 1.000 | 1.400 | 1.065 | 0.232 | 0.001 | 0.000 | 1.000 | 0.347 | 1.000 |
| 1.000 | 1.500 | 1.097 | 0.223 | 0.000 | 0.000 | 1.000 | 0.030 | 1.000 |
| 1.010 | 0.500 | 0.893 | 0.539 | 0.989 | 1.000 | 0.000 | 1.000 | 1.366 |
| 1.010 | 0.600 | 0.951 | 0.479 | 0.940 | 1.000 | 0.000 | 1.000 | 3.139 |
| 1.010 | 0.700 | 1.001 | 0.432 | 0.842 | 1.000 | 0.030 | 1.000 | 3.327 |
| 1.010 | 0.800 | 1.036 | 0.391 | 0.660 | 1.000 | 0.386 | 1.000 | 1.653 |
| 1.010 | 0.900 | 1.062 | 0.357 | 0.464 | 1.000 | 0.941 | 1.000 | 1.119 |
| 1.010 | 1.000 | 1.078 | 0.326 | 0.273 | 1.000 | 1.000 | 1.020 | 1.000 |
| 1.010 | 1.100 | 1.087 | 0.298 | 0.129 | 0.911 | 1.000 | 1.069 | 1.000 |
| 1.010 | 1.200 | 1.101 | 0.277 | 0.042 | 0.188 | 1.000 | 1.455 | 1.000 |
| 1.010 | 1.300 | 1.120 | 0.260 | 0.010 | 0.010 | 1.000 | 1.079 | 1.000 |
| 1.010 | 1.400 | 1.158 | 0.250 | 0.002 | 0.000 | 1.000 | 0.465 | 1.000 |
| 1.010 | 1.500 | 1.206 | 0.243 | 0.000 | 0.000 | 1.000 | 0.050 | 1.000 |
| 1.050 | 0.300 | 0.735 | 0.712 | 1.000 | 1.000 | 0.000 | 1.000 | 0.010 |
| 1.050 | 0.500 | 0.993 | 0.577 | 0.996 | 1.000 | 0.000 | 1.000 | 0.861 |
| 1.050 | 0.700 | 1.157 | 0.480 | 0.887 | 1.000 | 0.030 | 1.000 | 3.941 |
| 1.050 | 0.800 | 1.221 | 0.443 | 0.702 | 1.000 | 0.743 | 1.000 | 1.812 |
| 1.050 | 0.900 | 1.276 | 0.412 | 0.490 | 1.000 | 1.000 | 1.010 | 1.188 |
| 1.050 | 1.000 | 1.319 | 0.383 | 0.273 | 1.000 | 1.000 | 1.020 | 1.030 |
| 1.050 | 1.100 | 1.364 | 0.360 | 0.118 | 0.822 | 1.000 | 1.158 | 1.010 |
| 1.050 | 1.300 | 1.482 | 0.331 | 0.006 | 0.000 | 1.000 | 0.970 | 1.000 |
| 1.050 | 1.500 | 1.662 | 0.322 | 0.000 | 0.000 | 1.000 | 0.010 | 1.000 |
| 1.050 | 1.700 | 2.032 | 0.347 | 0.000 | 0.000 | 1.000 | 0.000 | 1.000 |
| 1.150 | 0.300 | 0.873 | 0.772 | 1.000 | 1.000 | 0.000 | 1.000 | 0.000 |
| 1.150 | 0.500 | 1.246 | 0.661 | 0.998 | 1.000 | 0.000 | 1.000 | 0.465 |
| 1.150 | 0.700 | 1.541 | 0.584 | 0.932 | 1.000 | 0.010 | 1.000 | 3.931 |
| 1.150 | 0.800 | 1.674 | 0.555 | 0.790 | 1.000 | 0.426 | 1.000 | 2.604 |
| 1.150 | 0.900 | 1.799 | 0.530 | 0.545 | 1.000 | 1.000 | 1.000 | 1.228 |
| 1.150 | 1.000 | 1.918 | 0.509 | 0.286 | 1.000 | 1.000 | 1.000 | 1.030 |
| 1.150 | 1.100 | 2.058 | 0.496 | 0.099 | 0.644 | 1.000 | 1.347 | 1.000 |
| 1.150 | 1.300 | 2.378 | 0.485 | 0.002 | 0.000 | 1.000 | 0.545 | 1.000 |
| 1.150 | 1.500 | 2.813 | 0.497 | 0.000 | 0.000 | 1.000 | 0.000 | 1.000 |
| 1.150 | 1.700 | 3.534 | 0.551 | 0.000 | 0.000 | 1.000 | 0.000 | 1.000 |
| 1.250 | 0.300 | 1.005 | 0.818 | 1.000 | 1.000 | 0.000 | 1.000 | 0.000 |
| 1.250 | 0.500 | 1.494 | 0.729 | 1.000 | 1.000 | 0.000 | 1.000 | 0.139 |
| 1.250 | 0.700 | 1.915 | 0.668 | 0.959 | 1.000 | 0.000 | 1.000 | 3.495 |
| 1.250 | 0.800 | 2.125 | 0.648 | 0.826 | 1.000 | 0.277 | 1.000 | 3.010 |
| 1.250 | 0.900 | 2.328 | 0.631 | 0.582 | 1.000 | 0.990 | 1.000 | 1.347 |
| 1.250 | 1.000 | 2.536 | 0.619 | 0.284 | 1.000 | 1.000 | 1.069 | 1.030 |
| 1.250 | 1.100 | 2.755 | 0.611 | 0.087 | 0.505 | 1.000 | 1.485 | 1.000 |
| 1.250 | 1.300 | 3.283 | 0.616 | 0.001 | 0.000 | 1.000 | 0.317 | 1.000 |
| 1.250 | 1.500 | 4.008 | 0.652 | 0.000 | 0.000 | 1.000 | 0.000 | 1.000 |
| 1.250 | 1.700 | 5.054 | 0.726 | 0.000 | 0.000 | 1.000 | 0.000 | 1.000 |
| 1.300 | 0.300 | 1.067 | 0.835 | 1.000 | 1.000 | 0.000 | 1.000 | 0.000 |
| 1.300 | 0.500 | 1.614 | 0.757 | 1.000 | 1.000 | 0.000 | 1.000 | 0.109 |
| 1.300 | 0.700 | 2.097 | 0.703 | 0.966 | 1.000 | 0.000 | 1.000 | 3.624 |
| 1.300 | 0.800 | 2.348 | 0.689 | 0.846 | 1.000 | 0.109 | 1.000 | 3.525 |
| 1.300 | 0.900 | 2.587 | 0.675 | 0.597 | 1.000 | 1.000 | 1.000 | 1.277 |
| 1.300 | 1.000 | 2.836 | 0.665 | 0.284 | 1.000 | 1.000 | 1.050 | 1.020 |
| 1.300 | 1.100 | 3.108 | 0.663 | 0.081 | 0.446 | 1.000 | 1.554 | 1.000 |
| 1.300 | 1.300 | 3.751 | 0.677 | 0.000 | 0.000 | 1.000 | 0.188 | 1.000 |
| 1.300 | 1.500 | 4.587 | 0.718 | 0.000 | 0.000 | 1.000 | 0.000 | 1.000 |
| 1.300 | 1.700 | 3.141 | 0.434 | 0.000 | 0.000 | 1.000 | 0.000 | 1.000 |
| 1.550 | 0.300 | 1.385 | 0.909 | 1.000 | 1.000 | 0.000 | 1.000 | 0.000 |
| 1.550 | 0.500 | 2.203 | 0.867 | 1.000 | 1.000 | 0.000 | 1.000 | 0.000 |
| 1.550 | 0.700 | 3.014 | 0.847 | 0.984 | 1.000 | 0.000 | 1.000 | 2.337 |
| 1.550 | 0.800 | 3.444 | 0.847 | 0.893 | 1.000 | 0.079 | 1.000 | 3.812 |

*Continued on next page*

TABLE s21 – Thermodynamic and structural properties of ethylene oxide (continued)

| $T/T_c$ | $\rho/\rho_c$ | $p/p_c$ | $z$ | $\Pi_{gas}$ | $p^{gas}_{inf}$ | $p^{liq}_{inf}$ | $\langle n^{gas}_c \rangle$ | $\langle n^{liq}_c \rangle$ |
|---|---|---|---|---|---|---|---|---|
| 1.550 | 0.900 | 3.885 | 0.850 | 0.653 | 1.000 | 0.980 | 1.000 | 1.554 |
| 1.550 | 1.000 | 4.350 | 0.856 | 0.299 | 1.000 | 1.000 | 1.010 | 1.059 |
| 1.550 | 1.100 | 4.859 | 0.869 | 0.070 | 0.267 | 1.000 | 1.644 | 1.000 |
| 1.550 | 1.300 | 6.039 | 0.914 | 0.000 | 0.000 | 1.000 | 0.079 | 1.000 |
| 1.550 | 1.500 | 7.541 | 0.989 | 0.000 | 0.000 | 1.000 | 0.000 | 1.000 |
| 1.550 | 1.700 | 9.556 | 1.106 | 0.000 | 0.000 | 1.000 | 0.000 | 1.000 |
| 2.450 | 0.300 | 2.462 | 1.022 | 1.000 | 1.000 | 0.000 | 1.000 | 0.000 |
| 2.450 | 0.500 | 4.219 | 1.051 | 1.000 | 1.000 | 0.000 | 1.000 | 0.000 |
| 2.450 | 0.700 | 6.147 | 1.093 | 0.996 | 1.000 | 0.000 | 1.000 | 1.020 |
| 2.450 | 0.800 | 7.208 | 1.122 | 0.950 | 1.000 | 0.000 | 1.000 | 4.158 |
| 2.450 | 0.900 | 8.354 | 1.156 | 0.734 | 1.000 | 0.752 | 1.000 | 2.040 |
| 2.450 | 1.000 | 9.585 | 1.193 | 0.309 | 1.000 | 1.000 | 1.030 | 1.030 |
| 2.450 | 1.100 | 10.921 | 1.236 | 0.047 | 0.079 | 1.000 | 2.109 | 1.000 |
| 2.450 | 1.300 | 14.010 | 1.342 | 0.000 | 0.000 | 1.000 | 0.000 | 1.000 |
| 2.450 | 1.500 | 17.819 | 1.479 | 0.000 | 0.000 | 1.000 | 0.000 | 1.000 |
| 2.450 | 1.700 | 22.555 | 1.652 | 0.000 | 0.000 | 1.000 | 0.000 | 1.000 |
| 2.950 | 0.300 | 3.045 | 1.050 | 1.000 | 1.000 | 0.000 | 1.000 | 0.000 |
| 2.950 | 0.500 | 5.296 | 1.095 | 1.000 | 1.000 | 0.000 | 1.000 | 0.000 |
| 2.950 | 0.700 | 7.824 | 1.156 | 0.997 | 1.000 | 0.000 | 1.000 | 0.812 |
| 2.950 | 0.800 | 9.234 | 1.194 | 0.959 | 1.000 | 0.000 | 1.000 | 3.822 |
| 2.950 | 0.900 | 10.747 | 1.235 | 0.740 | 1.000 | 0.762 | 1.000 | 1.911 |
| 2.950 | 1.000 | 12.383 | 1.281 | 0.307 | 1.000 | 1.000 | 1.050 | 1.030 |
| 2.950 | 1.100 | 14.164 | 1.332 | 0.044 | 0.079 | 1.000 | 2.139 | 1.000 |
| 2.950 | 1.300 | 18.289 | 1.455 | 0.000 | 0.000 | 1.000 | 0.000 | 1.000 |
| 2.950 | 1.500 | 23.295 | 1.606 | 0.000 | 0.000 | 1.000 | 0.000 | 1.000 |
| 2.950 | 1.700 | 29.486 | 1.794 | 0.000 | 0.000 | 1.000 | 0.000 | 1.000 |
| 3.450 | 0.300 | 3.621 | 1.067 | 1.000 | 1.000 | 0.000 | 1.000 | 0.000 |
| 3.450 | 0.500 | 6.359 | 1.125 | 1.000 | 1.000 | 0.000 | 1.000 | 0.000 |
| 3.450 | 0.700 | 9.475 | 1.197 | 0.998 | 1.000 | 0.000 | 1.000 | 0.762 |
| 3.450 | 0.800 | 11.214 | 1.239 | 0.964 | 1.000 | 0.000 | 1.000 | 3.653 |
| 3.450 | 0.900 | 13.090 | 1.286 | 0.749 | 1.000 | 0.723 | 1.000 | 2.059 |
| 3.450 | 1.000 | 15.129 | 1.338 | 0.311 | 1.000 | 1.000 | 1.040 | 1.020 |
| 3.450 | 1.100 | 17.353 | 1.395 | 0.044 | 0.069 | 1.000 | 2.158 | 1.000 |
| 3.450 | 1.300 | 22.454 | 1.527 | 0.000 | 0.000 | 1.000 | 0.040 | 1.000 |
| 3.450 | 1.500 | 28.621 | 1.687 | 0.000 | 0.000 | 1.000 | 0.000 | 1.000 |
| 3.450 | 1.700 | 36.220 | 1.884 | 0.000 | 0.000 | 1.000 | 0.000 | 1.000 |

TABLE s22: Thermodynamic and structural properties of ethane

| $T/T_c$ | $\rho/\rho_c$ | $p/p_c$ | $z$ | $\Pi_{gas}$ | $p^{gas}_{inf}$ | $p^{liq}_{inf}$ | $\langle n^{gas}_c \rangle$ | $\langle n^{liq}_c \rangle$ |
|---|---|---|---|---|---|---|---|---|
| 1.000 | 0.500 | 0.842 | 0.599 | 0.996 | 1.000 | 0.000 | 1.000 | 0.772 |
| 1.000 | 0.600 | 0.911 | 0.539 | 0.973 | 1.000 | 0.000 | 1.000 | 2.495 |
| 1.000 | 0.700 | 0.957 | 0.486 | 0.894 | 1.000 | 0.000 | 1.000 | 3.307 |
| 1.000 | 0.800 | 0.984 | 0.437 | 0.731 | 1.000 | 0.178 | 1.000 | 1.861 |
| 1.000 | 0.900 | 0.998 | 0.394 | 0.507 | 1.000 | 0.832 | 1.000 | 1.129 |
| 1.000 | 1.000 | 1.009 | 0.359 | 0.289 | 1.000 | 1.000 | 1.010 | 1.030 |
| 1.000 | 1.100 | 1.009 | 0.326 | 0.131 | 0.881 | 1.000 | 1.168 | 1.000 |
| 1.000 | 1.200 | 1.017 | 0.301 | 0.036 | 0.109 | 1.000 | 1.436 | 1.000 |
| 1.000 | 1.300 | 1.027 | 0.281 | 0.007 | 0.010 | 1.000 | 0.881 | 1.000 |
| 1.000 | 1.400 | 1.069 | 0.271 | 0.001 | 0.000 | 1.000 | 0.238 | 1.000 |
| 1.000 | 1.500 | 1.134 | 0.269 | 0.000 | 0.000 | 1.000 | 0.000 | 1.000 |
| 1.010 | 0.500 | 0.865 | 0.609 | 0.998 | 1.000 | 0.000 | 1.000 | 0.515 |
| 1.010 | 0.600 | 0.938 | 0.550 | 0.979 | 1.000 | 0.000 | 1.000 | 2.386 |
| 1.010 | 0.700 | 0.986 | 0.495 | 0.903 | 1.000 | 0.010 | 1.000 | 3.594 |
| 1.010 | 0.800 | 1.022 | 0.450 | 0.742 | 1.000 | 0.119 | 1.000 | 1.931 |
| 1.010 | 0.900 | 1.044 | 0.408 | 0.520 | 1.000 | 0.663 | 1.000 | 1.218 |
| 1.010 | 1.000 | 1.059 | 0.373 | 0.295 | 1.000 | 1.000 | 1.000 | 1.020 |
| 1.010 | 1.100 | 1.071 | 0.343 | 0.126 | 0.842 | 1.000 | 1.129 | 1.000 |
| 1.010 | 1.200 | 1.083 | 0.318 | 0.038 | 0.129 | 1.000 | 1.545 | 1.000 |
| 1.010 | 1.300 | 1.110 | 0.300 | 0.007 | 0.000 | 1.000 | 0.851 | 1.000 |

*Continued on next page*

TABLE s22 – Thermodynamic and structural properties of ethane (continued)

| $T/T_c$ | $\rho/\rho_c$ | $p/p_c$ | $z$ | $\Pi_{gas}$ | $p_{inf}^{gas}$ | $p_{inf}^{liq}$ | $\langle n_c^{gas}\rangle$ | $\langle n_c^{liq}\rangle$ |
|---|---|---|---|---|---|---|---|---|
| 1.010 | 1.400 | 1.154 | 0.290 | 0.001 | 0.000 | 1.000 | 0.129 | 1.000 |
| 1.010 | 1.500 | 1.225 | 0.287 | 0.000 | 0.000 | 1.000 | 0.010 | 1.000 |
| 1.050 | 0.200 | 0.497 | 0.841 | 1.000 | 1.000 | 0.000 | 1.000 | 0.000 |
| 1.050 | 0.400 | 0.829 | 0.701 | 1.000 | 1.000 | 0.000 | 1.000 | 0.020 |
| 1.050 | 0.600 | 1.041 | 0.587 | 0.987 | 1.000 | 0.000 | 1.000 | 1.772 |
| 1.050 | 0.800 | 1.169 | 0.495 | 0.769 | 1.000 | 0.515 | 1.000 | 2.158 |
| 1.050 | 0.900 | 1.219 | 0.458 | 0.540 | 1.000 | 1.000 | 1.000 | 1.267 |
| 1.050 | 1.000 | 1.260 | 0.426 | 0.296 | 1.000 | 1.000 | 1.000 | 1.020 |
| 1.050 | 1.100 | 1.299 | 0.400 | 0.115 | 0.752 | 1.000 | 1.198 | 1.000 |
| 1.050 | 1.200 | 1.357 | 0.383 | 0.026 | 0.050 | 1.000 | 1.465 | 1.000 |
| 1.050 | 1.400 | 1.491 | 0.360 | 0.000 | 0.000 | 1.000 | 0.069 | 1.000 |
| 1.050 | 1.600 | 1.829 | 0.387 | 0.000 | 0.000 | 1.000 | 0.000 | 1.000 |
| 1.100 | 0.200 | 0.529 | 0.854 | 1.000 | 1.000 | 0.000 | 1.000 | 0.000 |
| 1.100 | 0.400 | 0.904 | 0.730 | 1.000 | 1.000 | 0.000 | 1.000 | 0.020 |
| 1.100 | 0.600 | 1.169 | 0.629 | 0.990 | 1.000 | 0.000 | 1.000 | 1.535 |
| 1.100 | 0.800 | 1.353 | 0.546 | 0.812 | 1.000 | 0.267 | 1.000 | 2.713 |
| 1.100 | 0.900 | 1.439 | 0.516 | 0.564 | 1.000 | 1.000 | 1.000 | 1.208 |
| 1.100 | 1.000 | 1.513 | 0.489 | 0.297 | 1.000 | 1.000 | 1.010 | 1.020 |
| 1.100 | 1.100 | 1.592 | 0.468 | 0.106 | 0.663 | 1.000 | 1.208 | 1.000 |
| 1.100 | 1.200 | 1.693 | 0.456 | 0.022 | 0.030 | 1.000 | 1.465 | 1.000 |
| 1.100 | 1.400 | 1.941 | 0.448 | 0.000 | 0.000 | 1.000 | 0.030 | 1.000 |
| 1.100 | 1.600 | 2.404 | 0.485 | 0.000 | 0.000 | 1.000 | 0.000 | 1.000 |
| 1.150 | 0.200 | 0.562 | 0.868 | 1.000 | 1.000 | 0.000 | 1.000 | 0.000 |
| 1.150 | 0.400 | 0.981 | 0.758 | 1.000 | 1.000 | 0.000 | 1.000 | 0.000 |
| 1.150 | 0.600 | 1.292 | 0.665 | 0.994 | 1.000 | 0.000 | 1.000 | 1.188 |
| 1.150 | 0.800 | 1.541 | 0.595 | 0.833 | 1.000 | 0.238 | 1.000 | 2.931 |
| 1.150 | 0.900 | 1.653 | 0.568 | 0.586 | 1.000 | 0.990 | 1.000 | 1.228 |
| 1.150 | 1.000 | 1.771 | 0.547 | 0.302 | 1.000 | 1.000 | 1.000 | 1.000 |
| 1.150 | 1.100 | 1.897 | 0.533 | 0.094 | 0.515 | 1.000 | 1.426 | 1.000 |
| 1.150 | 1.200 | 2.022 | 0.521 | 0.016 | 0.010 | 1.000 | 1.584 | 1.000 |
| 1.150 | 1.400 | 2.397 | 0.529 | 0.000 | 0.000 | 1.000 | 0.030 | 1.000 |
| 1.150 | 1.600 | 2.979 | 0.575 | 0.000 | 0.000 | 1.000 | 0.000 | 1.000 |
| 1.200 | 0.200 | 0.595 | 0.881 | 1.000 | 1.000 | 0.000 | 1.000 | 0.000 |
| 1.200 | 0.400 | 1.054 | 0.780 | 1.000 | 1.000 | 0.000 | 1.000 | 0.000 |
| 1.200 | 0.600 | 1.414 | 0.698 | 0.996 | 1.000 | 0.000 | 1.000 | 0.990 |
| 1.200 | 0.800 | 1.723 | 0.638 | 0.849 | 1.000 | 0.168 | 1.000 | 3.485 |
| 1.200 | 0.900 | 1.869 | 0.615 | 0.602 | 1.000 | 1.000 | 1.000 | 1.228 |
| 1.200 | 1.000 | 2.023 | 0.599 | 0.302 | 1.000 | 1.000 | 1.010 | 1.030 |
| 1.200 | 1.100 | 2.181 | 0.587 | 0.092 | 0.515 | 1.000 | 1.337 | 1.010 |
| 1.200 | 1.200 | 2.377 | 0.587 | 0.016 | 0.010 | 1.000 | 1.307 | 1.000 |
| 1.200 | 1.400 | 2.855 | 0.604 | 0.000 | 0.000 | 1.000 | 0.010 | 1.000 |
| 1.200 | 1.600 | 3.588 | 0.664 | 0.000 | 0.000 | 1.000 | 0.000 | 1.000 |
| 1.250 | 0.200 | 0.628 | 0.893 | 1.000 | 1.000 | 0.000 | 1.000 | 0.000 |
| 1.250 | 0.400 | 1.127 | 0.801 | 1.000 | 1.000 | 0.000 | 1.000 | 0.000 |
| 1.250 | 0.600 | 1.537 | 0.728 | 0.997 | 1.000 | 0.000 | 1.000 | 0.832 |
| 1.250 | 0.800 | 1.903 | 0.676 | 0.868 | 1.000 | 0.139 | 1.000 | 3.376 |
| 1.250 | 0.900 | 2.089 | 0.660 | 0.622 | 1.000 | 0.980 | 1.000 | 1.396 |
| 1.250 | 1.000 | 2.274 | 0.646 | 0.306 | 1.000 | 1.000 | 1.030 | 1.010 |
| 1.250 | 1.100 | 2.476 | 0.640 | 0.089 | 0.475 | 1.000 | 1.396 | 1.000 |
| 1.250 | 1.200 | 2.699 | 0.639 | 0.012 | 0.010 | 1.000 | 1.337 | 1.000 |
| 1.250 | 1.400 | 3.297 | 0.669 | 0.000 | 0.000 | 1.000 | 0.000 | 1.000 |
| 1.250 | 1.600 | 4.181 | 0.743 | 0.000 | 0.000 | 1.000 | 0.000 | 1.000 |
| 1.300 | 0.200 | 0.660 | 0.902 | 1.000 | 1.000 | 0.000 | 1.000 | 0.000 |
| 1.300 | 0.400 | 1.200 | 0.820 | 1.000 | 1.000 | 0.000 | 1.000 | 0.000 |
| 1.300 | 0.600 | 1.664 | 0.758 | 0.998 | 1.000 | 0.000 | 1.000 | 0.485 |
| 1.300 | 0.800 | 2.087 | 0.713 | 0.876 | 1.000 | 0.119 | 1.000 | 3.871 |
| 1.300 | 0.900 | 2.304 | 0.700 | 0.638 | 1.000 | 0.960 | 1.000 | 1.505 |
| 1.300 | 1.000 | 2.525 | 0.690 | 0.306 | 1.000 | 1.000 | 1.030 | 1.010 |
| 1.300 | 1.100 | 2.770 | 0.688 | 0.083 | 0.475 | 1.000 | 1.386 | 1.000 |
| 1.300 | 1.200 | 3.045 | 0.694 | 0.010 | 0.000 | 1.000 | 1.208 | 1.000 |
| 1.300 | 1.400 | 3.749 | 0.732 | 0.000 | 0.000 | 1.000 | 0.020 | 1.000 |

*Continued on next page*

TABLE s22 – Thermodynamic and structural properties of ethane (continued)

| $T/T_c$ | $\rho/\rho_c$ | $p/p_c$ | $z$ | $\Pi_{gas}$ | $p^{gas}_{inf}$ | $p^{liq}_{inf}$ | $\langle n^{gas}_c\rangle$ | $\langle n^{liq}_c\rangle$ |
|---|---|---|---|---|---|---|---|---|
| 1.300 | 1.600 | 4.754 | 0.812 | 0.000 | 0.000 | 1.000 | 0.000 | 1.000 |
| 1.600 | 0.200 | 0.852 | 0.946 | 1.000 | 1.000 | 0.000 | 1.000 | 0.000 |
| 1.600 | 0.400 | 1.633 | 0.907 | 1.000 | 1.000 | 0.000 | 1.000 | 0.000 |
| 1.600 | 0.600 | 2.388 | 0.884 | 1.000 | 1.000 | 0.000 | 1.000 | 0.109 |
| 1.600 | 0.800 | 3.170 | 0.880 | 0.922 | 1.000 | 0.030 | 1.000 | 4.149 |
| 1.600 | 0.900 | 3.583 | 0.884 | 0.681 | 1.000 | 0.911 | 1.000 | 1.772 |
| 1.600 | 1.000 | 4.029 | 0.895 | 0.311 | 1.000 | 1.000 | 1.030 | 1.030 |
| 1.600 | 1.100 | 4.520 | 0.913 | 0.069 | 0.356 | 1.000 | 1.663 | 1.000 |
| 1.600 | 1.200 | 5.081 | 0.940 | 0.004 | 0.000 | 1.000 | 0.931 | 1.000 |
| 1.600 | 1.400 | 6.438 | 1.021 | 0.000 | 0.000 | 1.000 | 0.000 | 1.000 |
| 1.600 | 1.600 | 8.279 | 1.149 | 0.000 | 0.000 | 1.000 | 0.000 | 1.000 |
| 1.800 | 0.200 | 0.979 | 0.966 | 1.000 | 1.000 | 0.000 | 1.000 | 0.000 |
| 1.800 | 0.400 | 1.920 | 0.948 | 1.000 | 1.000 | 0.000 | 1.000 | 0.000 |
| 1.800 | 0.600 | 2.866 | 0.943 | 1.000 | 1.000 | 0.000 | 1.000 | 0.119 |
| 1.800 | 0.800 | 3.877 | 0.957 | 0.934 | 1.000 | 0.030 | 1.000 | 3.921 |
| 1.800 | 0.900 | 4.430 | 0.972 | 0.710 | 1.000 | 0.842 | 1.000 | 1.693 |
| 1.800 | 1.000 | 5.026 | 0.992 | 0.318 | 1.000 | 1.000 | 1.010 | 1.010 |
| 1.800 | 1.100 | 5.685 | 1.020 | 0.059 | 0.198 | 1.000 | 2.000 | 1.000 |
| 1.800 | 1.200 | 6.428 | 1.057 | 0.003 | 0.000 | 1.000 | 0.594 | 1.000 |
| 1.800 | 1.400 | 8.203 | 1.157 | 0.000 | 0.000 | 1.000 | 0.000 | 1.000 |
| 1.800 | 1.600 | 10.587 | 1.306 | 0.000 | 0.000 | 1.000 | 0.000 | 1.000 |
| 2.400 | 0.200 | 1.358 | 1.005 | 1.000 | 1.000 | 0.000 | 1.000 | 0.000 |
| 2.400 | 0.400 | 2.764 | 1.023 | 1.000 | 1.000 | 0.000 | 1.000 | 0.000 |
| 2.400 | 0.600 | 4.277 | 1.055 | 1.000 | 1.000 | 0.000 | 1.000 | 0.040 |
| 2.400 | 0.800 | 5.979 | 1.107 | 0.954 | 1.000 | 0.010 | 1.000 | 4.040 |
| 2.400 | 0.900 | 6.930 | 1.140 | 0.740 | 1.000 | 0.743 | 1.000 | 2.178 |
| 2.400 | 1.000 | 7.970 | 1.180 | 0.321 | 1.000 | 1.000 | 1.040 | 1.020 |
| 2.400 | 1.100 | 9.113 | 1.227 | 0.046 | 0.099 | 1.000 | 2.099 | 1.000 |
| 2.400 | 1.200 | 10.400 | 1.283 | 0.002 | 0.000 | 1.000 | 0.426 | 1.000 |
| 2.400 | 1.400 | 13.423 | 1.420 | 0.000 | 0.000 | 1.000 | 0.000 | 1.000 |
| 2.400 | 1.600 | 17.303 | 1.601 | 0.000 | 0.000 | 1.000 | 0.000 | 1.000 |
| 3.100 | 0.200 | 1.794 | 1.028 | 1.000 | 1.000 | 0.000 | 1.000 | 0.000 |
| 3.100 | 0.400 | 3.736 | 1.071 | 1.000 | 1.000 | 0.000 | 1.000 | 0.000 |
| 3.100 | 0.600 | 5.900 | 1.127 | 1.000 | 1.000 | 0.000 | 1.000 | 0.040 |
| 3.100 | 0.800 | 8.382 | 1.201 | 0.964 | 1.000 | 0.000 | 1.000 | 3.752 |
| 3.100 | 0.900 | 9.797 | 1.248 | 0.763 | 1.000 | 0.673 | 1.000 | 2.198 |
| 3.100 | 1.000 | 11.331 | 1.299 | 0.321 | 1.000 | 1.000 | 1.000 | 1.010 |
| 3.100 | 1.100 | 13.011 | 1.356 | 0.040 | 0.050 | 1.000 | 2.040 | 1.000 |
| 3.100 | 1.200 | 14.900 | 1.423 | 0.001 | 0.000 | 1.000 | 0.436 | 1.000 |
| 3.100 | 1.400 | 19.314 | 1.581 | 0.000 | 0.000 | 1.000 | 0.000 | 1.000 |
| 3.100 | 1.600 | 24.862 | 1.781 | 0.000 | 0.000 | 1.000 | 0.000 | 1.000 |
| 3.500 | 0.200 | 2.045 | 1.038 | 1.000 | 1.000 | 0.000 | 1.000 | 0.000 |
| 3.500 | 0.400 | 4.291 | 1.089 | 1.000 | 1.000 | 0.000 | 1.000 | 0.000 |
| 3.500 | 0.600 | 6.815 | 1.153 | 1.000 | 1.000 | 0.000 | 1.000 | 0.020 |
| 3.500 | 0.800 | 9.748 | 1.237 | 0.966 | 1.000 | 0.000 | 1.000 | 3.802 |
| 3.500 | 0.900 | 11.398 | 1.286 | 0.764 | 1.000 | 0.703 | 1.000 | 2.267 |
| 3.500 | 1.000 | 13.216 | 1.342 | 0.317 | 1.000 | 1.000 | 1.040 | 1.020 |
| 3.500 | 1.100 | 15.216 | 1.404 | 0.038 | 0.050 | 1.000 | 2.238 | 1.000 |
| 3.500 | 1.200 | 17.413 | 1.473 | 0.001 | 0.000 | 1.000 | 0.327 | 1.000 |
| 3.500 | 1.400 | 22.616 | 1.640 | 0.000 | 0.000 | 1.000 | 0.000 | 1.000 |
| 3.500 | 1.600 | 29.100 | 1.846 | 0.000 | 0.000 | 1.000 | 0.000 | 1.000 |

TABLE s23: Thermodynamic and structural properties of ammonia

| $T/T_c$ | $\rho/\rho_c$ | $p/p_c$ | $z$ | $\Pi_{gas}$ | $p^{gas}_{inf}$ | $p^{liq}_{inf}$ | $\langle n^{gas}_c\rangle$ | $\langle n^{liq}_c\rangle$ |
|---|---|---|---|---|---|---|---|---|
| 1.000 | 0.500 | 0.874 | 0.531 | 0.990 | 1.000 | 0.000 | 1.000 | 1.525 |
| 1.000 | 0.600 | 0.932 | 0.473 | 0.944 | 1.000 | 0.000 | 1.000 | 3.297 |
| 1.000 | 0.700 | 0.968 | 0.420 | 0.825 | 1.000 | 0.059 | 1.000 | 2.960 |
| 1.000 | 0.800 | 0.997 | 0.379 | 0.659 | 1.000 | 0.535 | 1.000 | 1.624 |
| 1.000 | 0.900 | 1.018 | 0.344 | 0.462 | 1.000 | 0.980 | 1.000 | 1.139 |

*Continued on next page*

TABLE s23 – Thermodynamic and structural properties of ammonia (continued)

| $T/T_c$ | $\rho/\rho_c$ | $p/p_c$ | $z$ | $\Pi_{gas}$ | $p_{inf}^{gas}$ | $p_{inf}^{liq}$ | $\langle n_c^{gas}\rangle$ | $\langle n_c^{liq}\rangle$ |
|---|---|---|---|---|---|---|---|---|
| 1.000 | 1.000 | 1.030 | 0.313 | 0.273 | 1.000 | 1.000 | 1.020 | 1.020 |
| 1.000 | 1.100 | 1.031 | 0.285 | 0.133 | 0.901 | 1.000 | 1.069 | 1.000 |
| 1.000 | 1.200 | 1.040 | 0.264 | 0.051 | 0.347 | 1.000 | 1.386 | 1.000 |
| 1.000 | 1.300 | 1.062 | 0.249 | 0.013 | 0.030 | 1.000 | 1.238 | 1.000 |
| 1.000 | 1.400 | 1.083 | 0.235 | 0.002 | 0.000 | 1.000 | 0.455 | 1.000 |
| 1.000 | 1.500 | 1.121 | 0.227 | 0.000 | 0.000 | 1.000 | 0.059 | 1.000 |
| 1.010 | 0.500 | 0.901 | 0.542 | 0.992 | 1.000 | 0.000 | 1.000 | 1.208 |
| 1.010 | 0.600 | 0.968 | 0.486 | 0.954 | 1.000 | 0.000 | 1.000 | 3.495 |
| 1.010 | 0.700 | 1.013 | 0.436 | 0.850 | 1.000 | 0.030 | 1.000 | 3.356 |
| 1.010 | 0.800 | 1.048 | 0.395 | 0.676 | 1.000 | 0.406 | 1.000 | 1.703 |
| 1.010 | 0.900 | 1.070 | 0.358 | 0.470 | 1.000 | 0.980 | 1.000 | 1.129 |
| 1.010 | 1.000 | 1.085 | 0.327 | 0.278 | 1.000 | 1.000 | 1.010 | 1.020 |
| 1.010 | 1.100 | 1.107 | 0.303 | 0.128 | 0.832 | 1.000 | 1.109 | 1.000 |
| 1.010 | 1.200 | 1.120 | 0.281 | 0.040 | 0.139 | 1.000 | 1.465 | 1.000 |
| 1.010 | 1.300 | 1.144 | 0.265 | 0.011 | 0.010 | 1.000 | 1.099 | 1.000 |
| 1.010 | 1.400 | 1.182 | 0.254 | 0.001 | 0.000 | 1.000 | 0.386 | 1.000 |
| 1.010 | 1.500 | 1.241 | 0.249 | 0.000 | 0.000 | 1.000 | 0.020 | 1.000 |
| 1.050 | 0.230 | 0.612 | 0.771 | 1.000 | 1.000 | 0.000 | 1.000 | 0.000 |
| 1.050 | 0.430 | 0.925 | 0.623 | 0.999 | 1.000 | 0.000 | 1.000 | 0.208 |
| 1.050 | 0.630 | 1.124 | 0.517 | 0.948 | 1.000 | 0.010 | 1.000 | 3.644 |
| 1.050 | 0.830 | 1.248 | 0.436 | 0.654 | 1.000 | 0.851 | 1.000 | 1.634 |
| 1.050 | 1.030 | 1.348 | 0.379 | 0.224 | 1.000 | 1.000 | 1.030 | 1.010 |
| 1.050 | 1.230 | 1.452 | 0.342 | 0.022 | 0.050 | 1.000 | 1.485 | 1.000 |
| 1.050 | 1.430 | 1.626 | 0.329 | 0.000 | 0.000 | 1.000 | 0.059 | 1.000 |
| 1.050 | 1.630 | 1.911 | 0.340 | 0.000 | 0.000 | 1.000 | 0.000 | 1.000 |
| 1.100 | 0.230 | 0.662 | 0.796 | 1.000 | 1.000 | 0.000 | 1.000 | 0.000 |
| 1.100 | 0.430 | 1.033 | 0.664 | 1.000 | 1.000 | 0.000 | 1.000 | 0.119 |
| 1.100 | 0.630 | 1.292 | 0.567 | 0.967 | 1.000 | 0.000 | 1.000 | 2.990 |
| 1.100 | 0.830 | 1.488 | 0.496 | 0.696 | 1.000 | 0.743 | 1.000 | 1.693 |
| 1.100 | 1.030 | 1.667 | 0.448 | 0.216 | 0.990 | 1.000 | 1.099 | 1.010 |
| 1.100 | 1.230 | 1.873 | 0.421 | 0.012 | 0.000 | 1.000 | 1.455 | 1.000 |
| 1.100 | 1.430 | 2.142 | 0.414 | 0.000 | 0.000 | 1.000 | 0.099 | 1.000 |
| 1.100 | 1.630 | 2.604 | 0.442 | 0.000 | 0.000 | 1.000 | 0.000 | 1.000 |
| 1.200 | 0.230 | 0.760 | 0.838 | 1.000 | 1.000 | 0.000 | 1.000 | 0.000 |
| 1.200 | 0.430 | 1.243 | 0.733 | 1.000 | 1.000 | 0.000 | 1.000 | 0.040 |
| 1.200 | 0.630 | 1.628 | 0.655 | 0.983 | 1.000 | 0.000 | 1.000 | 2.376 |
| 1.200 | 0.830 | 1.971 | 0.602 | 0.750 | 1.000 | 0.673 | 1.000 | 2.208 |
| 1.200 | 1.030 | 2.317 | 0.570 | 0.214 | 0.990 | 1.000 | 1.030 | 1.010 |
| 1.200 | 1.230 | 2.715 | 0.559 | 0.010 | 0.000 | 1.000 | 1.178 | 1.000 |
| 1.200 | 1.430 | 3.226 | 0.572 | 0.000 | 0.000 | 1.000 | 0.020 | 1.000 |
| 1.200 | 1.630 | 3.977 | 0.618 | 0.000 | 0.000 | 1.000 | 0.000 | 1.000 |
| 1.300 | 0.230 | 0.855 | 0.870 | 1.000 | 1.000 | 0.000 | 1.000 | 0.000 |
| 1.300 | 0.430 | 1.446 | 0.787 | 1.000 | 1.000 | 0.000 | 1.000 | 0.000 |
| 1.300 | 0.630 | 1.959 | 0.728 | 0.989 | 1.000 | 0.000 | 1.000 | 1.584 |
| 1.300 | 0.830 | 2.442 | 0.688 | 0.787 | 1.000 | 0.406 | 1.000 | 2.584 |
| 1.300 | 1.030 | 2.952 | 0.671 | 0.213 | 1.000 | 1.000 | 1.099 | 1.010 |
| 1.300 | 1.230 | 3.553 | 0.676 | 0.006 | 0.000 | 1.000 | 0.950 | 1.000 |
| 1.300 | 1.430 | 4.316 | 0.706 | 0.000 | 0.000 | 1.000 | 0.000 | 1.000 |
| 1.300 | 1.630 | 5.346 | 0.767 | 0.000 | 0.000 | 1.000 | 0.000 | 1.000 |
| 1.650 | 0.230 | 1.177 | 0.943 | 1.000 | 1.000 | 0.000 | 1.000 | 0.000 |
| 1.650 | 0.430 | 2.125 | 0.911 | 1.000 | 1.000 | 0.000 | 1.000 | 0.000 |
| 1.650 | 0.630 | 3.068 | 0.898 | 0.998 | 1.000 | 0.000 | 1.000 | 0.723 |
| 1.650 | 0.830 | 4.049 | 0.899 | 0.863 | 1.000 | 0.020 | 1.000 | 3.931 |
| 1.650 | 1.030 | 5.142 | 0.920 | 0.204 | 0.980 | 1.000 | 1.050 | 1.000 |
| 1.650 | 1.230 | 6.438 | 0.965 | 0.001 | 0.000 | 1.000 | 0.376 | 1.000 |
| 1.650 | 1.430 | 8.026 | 1.035 | 0.000 | 0.000 | 1.000 | 0.000 | 1.000 |
| 1.650 | 1.630 | 10.080 | 1.140 | 0.000 | 0.000 | 1.000 | 0.000 | 1.000 |
| 2.030 | 0.230 | 1.513 | 0.986 | 1.000 | 1.000 | 0.000 | 1.000 | 0.000 |
| 2.030 | 0.430 | 2.832 | 0.987 | 1.000 | 1.000 | 0.000 | 1.000 | 0.000 |
| 2.030 | 0.630 | 4.211 | 1.002 | 0.999 | 1.000 | 0.000 | 1.000 | 0.248 |
| 2.030 | 0.830 | 5.724 | 1.033 | 0.889 | 1.000 | 0.079 | 1.000 | 3.812 |

*Continued on next page*

TABLE s23 – Thermodynamic and structural properties of ammonia (continued)

| $T/T_c$ | $\rho/\rho_c$ | $p/p_c$ | $z$ | $\Pi_{gas}$ | $p_{inf}^{gas}$ | $p_{inf}^{liq}$ | $\langle n_c^{gas}\rangle$ | $\langle n_c^{liq}\rangle$ |
|---|---|---|---|---|---|---|---|---|
| 2.030 | 1.030 | 7.450 | 1.084 | 0.205 | 0.990 | 1.000 | 1.139 | 1.000 |
| 2.030 | 1.230 | 9.458 | 1.152 | 0.001 | 0.000 | 1.000 | 0.317 | 1.000 |
| 2.030 | 1.430 | 11.929 | 1.250 | 0.000 | 0.000 | 1.000 | 0.000 | 1.000 |
| 2.030 | 1.630 | 15.003 | 1.379 | 0.000 | 0.000 | 1.000 | 0.000 | 1.000 |
| 2.460 | 0.230 | 1.887 | 1.014 | 1.000 | 1.000 | 0.000 | 1.000 | 0.000 |
| 2.460 | 0.430 | 3.608 | 1.037 | 1.000 | 1.000 | 0.000 | 1.000 | 0.000 |
| 2.460 | 0.630 | 5.473 | 1.074 | 1.000 | 1.000 | 0.000 | 1.000 | 0.149 |
| 2.460 | 0.830 | 7.554 | 1.125 | 0.904 | 1.000 | 0.030 | 1.000 | 4.317 |
| 2.460 | 1.030 | 9.957 | 1.195 | 0.197 | 0.970 | 1.000 | 1.178 | 1.000 |
| 2.460 | 1.230 | 12.785 | 1.285 | 0.000 | 0.000 | 1.000 | 0.198 | 1.000 |
| 2.460 | 1.430 | 16.174 | 1.398 | 0.000 | 0.000 | 1.000 | 0.000 | 1.000 |
| 2.460 | 1.630 | 20.336 | 1.543 | 0.000 | 0.000 | 1.000 | 0.000 | 1.000 |
| 2.960 | 0.230 | 2.314 | 1.034 | 1.000 | 1.000 | 0.000 | 1.000 | 0.000 |
| 2.960 | 0.430 | 4.491 | 1.073 | 1.000 | 1.000 | 0.000 | 1.000 | 0.000 |
| 2.960 | 0.630 | 6.910 | 1.127 | 1.000 | 1.000 | 0.000 | 1.000 | 0.099 |
| 2.960 | 0.830 | 9.622 | 1.191 | 0.916 | 1.000 | 0.020 | 1.000 | 4.505 |
| 2.960 | 1.030 | 12.781 | 1.275 | 0.195 | 0.980 | 1.000 | 1.158 | 1.000 |
| 2.960 | 1.230 | 16.491 | 1.378 | 0.001 | 0.000 | 1.000 | 0.248 | 1.000 |
| 2.960 | 1.430 | 20.932 | 1.504 | 0.000 | 0.000 | 1.000 | 0.000 | 1.000 |
| 2.960 | 1.630 | 26.279 | 1.657 | 0.000 | 0.000 | 1.000 | 0.000 | 1.000 |
| 3.500 | 0.230 | 2.772 | 1.047 | 1.000 | 1.000 | 0.000 | 1.000 | 0.000 |
| 3.500 | 0.430 | 5.431 | 1.098 | 1.000 | 1.000 | 0.000 | 1.000 | 0.000 |
| 3.500 | 0.630 | 8.415 | 1.161 | 1.000 | 1.000 | 0.000 | 1.000 | 0.079 |
| 3.500 | 0.830 | 11.812 | 1.237 | 0.917 | 1.000 | 0.030 | 1.000 | 4.297 |
| 3.500 | 1.030 | 15.752 | 1.329 | 0.198 | 0.950 | 1.000 | 1.129 | 1.010 |
| 3.500 | 1.230 | 20.381 | 1.440 | 0.000 | 0.000 | 1.000 | 0.129 | 1.000 |
| 3.500 | 1.430 | 25.893 | 1.574 | 0.000 | 0.000 | 1.000 | 0.000 | 1.000 |
| 3.500 | 1.630 | 32.491 | 1.732 | 0.000 | 0.000 | 1.000 | 0.000 | 1.000 |

TABLE s24: Thermodynamic and structural properties of nitrogen

| $T/T_c$ | $\rho/\rho_c$ | $p/p_c$ | $z$ | $\Pi_{gas}$ | $p_{inf}^{gas}$ | $p_{inf}^{liq}$ | $\langle n_c^{gas}\rangle$ | $\langle n_c^{liq}\rangle$ |
|---|---|---|---|---|---|---|---|---|
| 1.000 | 0.500 | 0.868 | 0.595 | 0.997 | 1.000 | 0.000 | 1.000 | 0.584 |
| 1.000 | 0.600 | 0.931 | 0.532 | 0.974 | 1.000 | 0.000 | 1.000 | 2.644 |
| 1.000 | 0.700 | 0.977 | 0.478 | 0.890 | 1.000 | 0.020 | 1.000 | 3.386 |
| 1.000 | 0.800 | 1.000 | 0.428 | 0.712 | 1.000 | 0.396 | 1.000 | 1.802 |
| 1.000 | 0.900 | 1.016 | 0.387 | 0.504 | 1.000 | 0.951 | 1.000 | 1.129 |
| 1.000 | 1.000 | 1.029 | 0.353 | 0.294 | 1.000 | 1.000 | 1.010 | 1.020 |
| 1.000 | 1.100 | 1.024 | 0.319 | 0.134 | 0.901 | 1.000 | 1.099 | 1.000 |
| 1.000 | 1.200 | 1.033 | 0.295 | 0.040 | 0.158 | 1.000 | 1.455 | 1.000 |
| 1.000 | 1.300 | 1.048 | 0.276 | 0.009 | 0.030 | 1.000 | 1.020 | 1.000 |
| 1.000 | 1.400 | 1.073 | 0.263 | 0.000 | 0.000 | 1.000 | 0.158 | 1.000 |
| 1.000 | 1.500 | 1.164 | 0.266 | 0.000 | 0.000 | 1.000 | 0.010 | 1.000 |
| 1.010 | 0.500 | 0.887 | 0.602 | 0.996 | 1.000 | 0.000 | 1.000 | 0.673 |
| 1.010 | 0.600 | 0.962 | 0.544 | 0.978 | 1.000 | 0.000 | 1.000 | 2.238 |
| 1.010 | 0.700 | 1.013 | 0.491 | 0.897 | 1.000 | 0.000 | 1.000 | 3.139 |
| 1.010 | 0.800 | 1.040 | 0.441 | 0.729 | 1.000 | 0.267 | 1.000 | 1.733 |
| 1.010 | 0.900 | 1.060 | 0.400 | 0.517 | 1.000 | 0.931 | 1.000 | 1.188 |
| 1.010 | 1.000 | 1.080 | 0.366 | 0.302 | 1.000 | 1.000 | 1.010 | 1.040 |
| 1.010 | 1.100 | 1.083 | 0.334 | 0.126 | 0.822 | 1.000 | 1.168 | 1.000 |
| 1.010 | 1.200 | 1.098 | 0.310 | 0.042 | 0.178 | 1.000 | 1.366 | 1.000 |
| 1.010 | 1.300 | 1.127 | 0.294 | 0.005 | 0.000 | 1.000 | 0.842 | 1.000 |
| 1.010 | 1.400 | 1.173 | 0.284 | 0.000 | 0.000 | 1.000 | 0.129 | 1.000 |
| 1.010 | 1.500 | 1.246 | 0.282 | 0.000 | 0.000 | 1.000 | 0.000 | 1.000 |
| 1.050 | 0.260 | 0.633 | 0.795 | 1.000 | 1.000 | 0.000 | 1.000 | 0.000 |
| 1.050 | 0.460 | 0.930 | 0.660 | 1.000 | 1.000 | 0.000 | 1.000 | 0.119 |
| 1.050 | 0.660 | 1.111 | 0.549 | 0.956 | 1.000 | 0.010 | 1.000 | 3.010 |
| 1.050 | 0.860 | 1.221 | 0.463 | 0.640 | 1.000 | 0.960 | 1.000 | 1.337 |
| 1.050 | 0.960 | 1.275 | 0.433 | 0.391 | 1.000 | 1.000 | 1.010 | 1.040 |
| 1.050 | 1.060 | 1.313 | 0.404 | 0.181 | 0.970 | 1.000 | 1.079 | 1.020 |

*Continued on next page*

TABLE s24 – Thermodynamic and structural properties of nitrogen (continued)

| $T/T_c$ | $\rho/\rho_c$ | $p/p_c$ | $z$ | $\Pi_{gas}$ | $p^{gas}_{inf}$ | $p^{liq}_{inf}$ | $\langle n^{gas}_c \rangle$ | $\langle n^{liq}_c \rangle$ |
|---|---|---|---|---|---|---|---|---|
| 1.050 | 1.160 | 1.359 | 0.382 | 0.055 | 0.287 | 1.000 | 1.396 | 1.000 |
| 1.050 | 1.260 | 1.413 | 0.366 | 0.011 | 0.000 | 1.000 | 1.149 | 1.000 |
| 1.050 | 1.460 | 1.610 | 0.360 | 0.000 | 0.000 | 1.000 | 0.030 | 1.000 |
| 1.050 | 1.660 | 2.053 | 0.404 | 0.000 | 0.000 | 1.000 | 0.000 | 1.000 |
| 1.100 | 0.260 | 0.679 | 0.814 | 1.000 | 1.000 | 0.000 | 1.000 | 0.000 |
| 1.100 | 0.460 | 1.024 | 0.694 | 1.000 | 1.000 | 0.000 | 1.000 | 0.050 |
| 1.100 | 0.660 | 1.264 | 0.597 | 0.965 | 1.000 | 0.000 | 1.000 | 2.743 |
| 1.100 | 0.860 | 1.438 | 0.521 | 0.672 | 1.000 | 0.871 | 1.000 | 1.505 |
| 1.100 | 0.960 | 1.515 | 0.492 | 0.396 | 1.000 | 1.000 | 1.000 | 1.020 |
| 1.100 | 1.060 | 1.595 | 0.469 | 0.170 | 0.950 | 1.000 | 1.059 | 1.010 |
| 1.100 | 1.160 | 1.693 | 0.455 | 0.047 | 0.208 | 1.000 | 1.485 | 1.000 |
| 1.100 | 1.260 | 1.791 | 0.443 | 0.007 | 0.000 | 1.000 | 0.931 | 1.000 |
| 1.100 | 1.460 | 2.123 | 0.453 | 0.000 | 0.000 | 1.000 | 0.000 | 1.000 |
| 1.100 | 1.660 | 2.699 | 0.507 | 0.000 | 0.000 | 1.000 | 0.000 | 1.000 |
| 1.150 | 0.260 | 0.724 | 0.830 | 1.000 | 1.000 | 0.000 | 1.000 | 0.000 |
| 1.150 | 0.460 | 1.115 | 0.722 | 1.000 | 1.000 | 0.000 | 1.000 | 0.050 |
| 1.150 | 0.660 | 1.409 | 0.636 | 0.976 | 1.000 | 0.000 | 1.000 | 2.485 |
| 1.150 | 0.860 | 1.650 | 0.572 | 0.697 | 1.000 | 0.842 | 1.000 | 1.772 |
| 1.150 | 0.960 | 1.767 | 0.549 | 0.415 | 1.000 | 1.000 | 1.000 | 1.030 |
| 1.150 | 1.060 | 1.891 | 0.532 | 0.168 | 0.950 | 1.000 | 1.139 | 1.000 |
| 1.150 | 1.160 | 2.020 | 0.519 | 0.039 | 0.119 | 1.000 | 1.723 | 1.000 |
| 1.150 | 1.260 | 2.171 | 0.513 | 0.004 | 0.000 | 1.000 | 0.733 | 1.000 |
| 1.150 | 1.460 | 2.627 | 0.536 | 0.000 | 0.000 | 1.000 | 0.000 | 1.000 |
| 1.150 | 1.660 | 3.376 | 0.606 | 0.000 | 0.000 | 1.000 | 0.000 | 1.000 |
| 1.200 | 0.260 | 0.770 | 0.846 | 1.000 | 1.000 | 0.000 | 1.000 | 0.000 |
| 1.200 | 0.460 | 1.206 | 0.749 | 1.000 | 1.000 | 0.000 | 1.000 | 0.030 |
| 1.200 | 0.660 | 1.551 | 0.671 | 0.982 | 1.000 | 0.000 | 1.000 | 2.297 |
| 1.200 | 0.860 | 1.861 | 0.618 | 0.719 | 1.000 | 0.782 | 1.000 | 1.812 |
| 1.200 | 0.960 | 2.012 | 0.599 | 0.423 | 1.000 | 1.000 | 1.000 | 1.030 |
| 1.200 | 1.060 | 2.174 | 0.586 | 0.165 | 0.921 | 1.000 | 1.109 | 1.000 |
| 1.200 | 1.160 | 2.354 | 0.580 | 0.037 | 0.119 | 1.000 | 1.752 | 1.000 |
| 1.200 | 1.260 | 2.559 | 0.580 | 0.002 | 0.000 | 1.000 | 0.624 | 1.000 |
| 1.200 | 1.460 | 3.130 | 0.612 | 0.000 | 0.000 | 1.000 | 0.000 | 1.000 |
| 1.200 | 1.660 | 4.032 | 0.694 | 0.000 | 0.000 | 1.000 | 0.000 | 1.000 |
| 1.250 | 0.260 | 0.816 | 0.860 | 1.000 | 1.000 | 0.000 | 1.000 | 0.000 |
| 1.250 | 0.460 | 1.298 | 0.774 | 1.000 | 1.000 | 0.000 | 1.000 | 0.010 |
| 1.250 | 0.660 | 1.699 | 0.706 | 0.985 | 1.000 | 0.000 | 1.000 | 2.030 |
| 1.250 | 0.860 | 2.071 | 0.660 | 0.730 | 1.000 | 0.792 | 1.000 | 1.901 |
| 1.250 | 0.960 | 2.253 | 0.643 | 0.428 | 1.000 | 1.000 | 1.000 | 1.050 |
| 1.250 | 1.060 | 2.457 | 0.636 | 0.154 | 0.901 | 1.000 | 1.119 | 1.010 |
| 1.250 | 1.160 | 2.684 | 0.634 | 0.025 | 0.010 | 1.000 | 1.842 | 1.000 |
| 1.250 | 1.260 | 2.948 | 0.641 | 0.002 | 0.000 | 1.000 | 0.535 | 1.000 |
| 1.250 | 1.460 | 3.649 | 0.685 | 0.000 | 0.000 | 1.000 | 0.000 | 1.000 |
| 1.250 | 1.660 | 4.711 | 0.778 | 0.000 | 0.000 | 1.000 | 0.000 | 1.000 |
| 1.300 | 0.260 | 0.860 | 0.872 | 1.000 | 1.000 | 0.000 | 1.000 | 0.000 |
| 1.300 | 0.460 | 1.389 | 0.796 | 1.000 | 1.000 | 0.000 | 1.000 | 0.000 |
| 1.300 | 0.660 | 1.842 | 0.736 | 0.990 | 1.000 | 0.000 | 1.000 | 1.703 |
| 1.300 | 0.860 | 2.283 | 0.700 | 0.755 | 1.000 | 0.673 | 1.000 | 2.099 |
| 1.300 | 0.960 | 2.504 | 0.688 | 0.434 | 1.000 | 1.000 | 1.000 | 1.109 |
| 1.300 | 1.060 | 2.743 | 0.682 | 0.153 | 0.891 | 1.000 | 1.158 | 1.010 |
| 1.300 | 1.160 | 3.018 | 0.686 | 0.027 | 0.069 | 1.000 | 1.822 | 1.000 |
| 1.300 | 1.260 | 3.335 | 0.698 | 0.001 | 0.000 | 1.000 | 0.446 | 1.000 |
| 1.300 | 1.460 | 4.146 | 0.749 | 0.000 | 0.000 | 1.000 | 0.000 | 1.000 |
| 1.300 | 1.660 | 5.368 | 0.852 | 0.000 | 0.000 | 1.000 | 0.000 | 1.000 |
| 1.400 | 0.260 | 0.951 | 0.895 | 1.000 | 1.000 | 0.000 | 1.000 | 0.000 |
| 1.400 | 0.460 | 1.570 | 0.835 | 1.000 | 1.000 | 0.000 | 1.000 | 0.000 |
| 1.400 | 0.660 | 2.136 | 0.792 | 0.993 | 1.000 | 0.000 | 1.000 | 1.337 |
| 1.400 | 0.860 | 2.705 | 0.770 | 0.768 | 1.000 | 0.584 | 1.000 | 2.257 |
| 1.400 | 0.960 | 2.995 | 0.764 | 0.447 | 1.000 | 1.000 | 1.010 | 1.079 |
| 1.400 | 1.060 | 3.327 | 0.768 | 0.149 | 0.921 | 1.000 | 1.129 | 1.000 |
| 1.400 | 1.160 | 3.693 | 0.779 | 0.022 | 0.030 | 1.000 | 1.683 | 1.000 |

*Continued on next page*

TABLE s24 – Thermodynamic and structural properties of nitrogen (continued)

| $T/T_c$ | $\rho/\rho_c$ | $p/p_c$ | $z$ | $\Pi_{gas}$ | $p^{gas}_{inf}$ | $p^{liq}_{inf}$ | $\langle n^{gas}_c \rangle$ | $\langle n^{liq}_c \rangle$ |
|---|---|---|---|---|---|---|---|---|
| 1.400 | 1.260 | 4.103 | 0.797 | 0.001 | 0.000 | 1.000 | 0.337 | 1.000 |
| 1.400 | 1.460 | 5.163 | 0.866 | 0.000 | 0.000 | 1.000 | 0.000 | 1.000 |
| 1.400 | 1.660 | 6.686 | 0.986 | 0.000 | 0.000 | 1.000 | 0.000 | 1.000 |
| 2.100 | 0.260 | 1.571 | 0.986 | 1.000 | 1.000 | 0.000 | 1.000 | 0.000 |
| 2.100 | 0.460 | 2.794 | 0.991 | 1.000 | 1.000 | 0.000 | 1.000 | 0.000 |
| 2.100 | 0.660 | 4.098 | 1.013 | 0.999 | 1.000 | 0.000 | 1.000 | 0.356 |
| 2.100 | 0.860 | 5.556 | 1.054 | 0.846 | 1.000 | 0.238 | 1.000 | 3.287 |
| 2.100 | 0.960 | 6.381 | 1.085 | 0.486 | 1.000 | 1.000 | 1.000 | 1.168 |
| 2.100 | 1.060 | 7.280 | 1.121 | 0.124 | 0.703 | 1.000 | 1.426 | 1.000 |
| 2.100 | 1.160 | 8.268 | 1.163 | 0.009 | 0.000 | 1.000 | 1.337 | 1.000 |
| 2.100 | 1.260 | 9.400 | 1.218 | 0.000 | 0.000 | 1.000 | 0.089 | 1.000 |
| 2.100 | 1.460 | 12.085 | 1.351 | 0.000 | 0.000 | 1.000 | 0.000 | 1.000 |
| 2.100 | 1.660 | 15.694 | 1.543 | 0.000 | 0.000 | 1.000 | 0.000 | 1.000 |
| 2.800 | 0.260 | 2.181 | 1.027 | 1.000 | 1.000 | 0.000 | 1.000 | 0.000 |
| 2.800 | 0.460 | 3.994 | 1.063 | 1.000 | 1.000 | 0.000 | 1.000 | 0.000 |
| 2.800 | 0.660 | 6.019 | 1.116 | 0.999 | 1.000 | 0.000 | 1.000 | 0.277 |
| 2.800 | 0.860 | 8.339 | 1.187 | 0.873 | 1.000 | 0.198 | 1.000 | 3.802 |
| 2.800 | 0.960 | 9.663 | 1.232 | 0.502 | 1.000 | 1.000 | 1.000 | 1.178 |
| 2.800 | 1.060 | 11.103 | 1.282 | 0.118 | 0.644 | 1.000 | 1.495 | 1.000 |
| 2.800 | 1.160 | 12.739 | 1.344 | 0.006 | 0.000 | 1.000 | 1.198 | 1.000 |
| 2.800 | 1.260 | 14.511 | 1.410 | 0.000 | 0.000 | 1.000 | 0.050 | 1.000 |
| 2.800 | 1.460 | 18.766 | 1.573 | 0.000 | 0.000 | 1.000 | 0.000 | 1.000 |
| 2.800 | 1.660 | 24.214 | 1.785 | 0.000 | 0.000 | 1.000 | 0.000 | 1.000 |
| 3.600 | 0.260 | 2.875 | 1.053 | 1.000 | 1.000 | 0.000 | 1.000 | 0.000 |
| 3.600 | 0.460 | 5.355 | 1.108 | 1.000 | 1.000 | 0.000 | 1.000 | 0.000 |
| 3.600 | 0.660 | 8.174 | 1.179 | 1.000 | 1.000 | 0.000 | 1.000 | 0.139 |
| 3.600 | 0.860 | 11.464 | 1.269 | 0.882 | 1.000 | 0.099 | 1.000 | 3.901 |
| 3.600 | 0.960 | 13.345 | 1.323 | 0.507 | 1.000 | 1.000 | 1.000 | 1.158 |
| 3.600 | 1.060 | 15.402 | 1.383 | 0.114 | 0.495 | 1.000 | 1.485 | 1.000 |
| 3.600 | 1.160 | 17.672 | 1.450 | 0.006 | 0.010 | 1.000 | 1.050 | 1.000 |
| 3.600 | 1.260 | 20.201 | 1.526 | 0.000 | 0.000 | 1.000 | 0.010 | 1.000 |
| 3.600 | 1.460 | 26.184 | 1.707 | 0.000 | 0.000 | 1.000 | 0.000 | 1.000 |
| 3.600 | 1.660 | 33.546 | 1.924 | 0.000 | 0.000 | 1.000 | 0.000 | 1.000 |

TABLE s25: Thermodynamic and structural properties of methanol

| $T/T_c$ | $\rho/\rho_c$ | $p/p_c$ | $z$ | $\Pi_{gas}$ | $p^{gas}_{inf}$ | $p^{liq}_{inf}$ | $\langle n^{gas}_c \rangle$ | $\langle n^{liq}_c \rangle$ |
|---|---|---|---|---|---|---|---|---|
| 1.000 | 0.500 | 0.901 | 0.466 | 0.975 | 1.000 | 0.000 | 1.000 | 2.584 |
| 1.000 | 0.600 | 0.943 | 0.407 | 0.893 | 1.000 | 0.000 | 1.000 | 3.653 |
| 1.000 | 0.700 | 0.973 | 0.360 | 0.767 | 1.000 | 0.059 | 1.000 | 2.673 |
| 1.000 | 0.800 | 0.990 | 0.320 | 0.573 | 1.000 | 0.455 | 1.000 | 1.455 |
| 1.000 | 0.900 | 1.009 | 0.290 | 0.411 | 1.000 | 1.000 | 1.000 | 1.099 |
| 1.000 | 1.000 | 1.010 | 0.261 | 0.244 | 1.000 | 1.000 | 1.030 | 1.040 |
| 1.000 | 1.100 | 1.026 | 0.241 | 0.127 | 0.931 | 1.000 | 1.119 | 1.000 |
| 1.000 | 1.200 | 1.024 | 0.221 | 0.047 | 0.277 | 1.000 | 1.406 | 1.000 |
| 1.000 | 1.300 | 1.037 | 0.206 | 0.012 | 0.020 | 1.000 | 1.228 | 1.000 |
| 1.000 | 1.400 | 1.066 | 0.197 | 0.002 | 0.000 | 1.000 | 0.475 | 1.000 |
| 1.000 | 1.500 | 1.102 | 0.190 | 0.000 | 0.000 | 1.000 | 0.069 | 1.000 |
| 1.010 | 0.500 | 0.000 | 0.000 | 0.979 | 1.000 | 0.000 | 1.000 | 2.426 |
| 1.010 | 0.600 | 0.934 | 0.399 | 0.905 | 1.000 | 0.000 | 1.000 | 4.168 |
| 1.010 | 0.700 | 0.987 | 0.361 | 0.777 | 1.000 | 0.010 | 1.000 | 2.881 |
| 1.010 | 0.800 | 1.025 | 0.328 | 0.605 | 1.000 | 0.366 | 1.000 | 1.396 |
| 1.010 | 0.900 | 1.053 | 0.300 | 0.417 | 1.000 | 1.000 | 1.010 | 1.089 |
| 1.010 | 1.000 | 1.074 | 0.275 | 0.250 | 1.000 | 1.000 | 1.010 | 1.030 |
| 1.010 | 1.100 | 1.095 | 0.255 | 0.118 | 0.871 | 1.000 | 1.129 | 1.000 |
| 1.010 | 1.200 | 1.106 | 0.236 | 0.043 | 0.168 | 1.000 | 1.554 | 1.000 |
| 1.010 | 1.300 | 1.117 | 0.220 | 0.012 | 0.020 | 1.000 | 1.317 | 1.000 |
| 1.010 | 1.400 | 1.138 | 0.208 | 0.003 | 0.000 | 1.000 | 0.564 | 1.000 |
| 1.010 | 1.500 | 1.182 | 0.202 | 0.000 | 0.000 | 1.000 | 0.119 | 1.000 |
| 1.050 | 0.200 | 0.621 | 0.765 | 1.000 | 1.000 | 0.000 | 1.000 | 0.000 |

*Continued on next page*

TABLE s25 – Thermodynamic and structural properties of methanol (continued)

| $T/T_c$ | $\rho/\rho_c$ | $p/p_c$ | $z$ | $\Pi_{gas}$ | $p_{inf}^{gas}$ | $p_{inf}^{liq}$ | $\langle n_c^{gas}\rangle$ | $\langle n_c^{liq}\rangle$ |
|---|---|---|---|---|---|---|---|---|
| 1.050 | 0.400 | 0.985 | 0.606 | 0.998 | 1.000 | 0.000 | 1.000 | 0.327 |
| 1.050 | 0.600 | 1.188 | 0.488 | 0.939 | 1.000 | 0.000 | 1.000 | 3.941 |
| 1.050 | 0.800 | 1.315 | 0.405 | 0.649 | 1.000 | 0.812 | 1.000 | 1.644 |
| 1.050 | 0.900 | 1.311 | 0.359 | 0.441 | 1.000 | 1.000 | 1.010 | 1.129 |
| 1.050 | 1.000 | 1.384 | 0.341 | 0.249 | 1.000 | 1.000 | 1.020 | 1.010 |
| 1.050 | 1.100 | 1.490 | 0.334 | 0.108 | 0.713 | 1.000 | 1.218 | 1.000 |
| 1.050 | 1.200 | 1.549 | 0.318 | 0.037 | 0.178 | 1.000 | 1.634 | 1.000 |
| 1.050 | 1.400 | 1.717 | 0.302 | 0.001 | 0.000 | 1.000 | 0.297 | 1.000 |
| 1.050 | 1.600 | 1.735 | 0.267 | 0.000 | 0.000 | 1.000 | 0.000 | 1.000 |
| 1.050 | 1.800 | 2.254 | 0.308 | 0.000 | 0.000 | 1.000 | 0.000 | 1.000 |
| 1.050 | 2.000 | 3.163 | 0.389 | 0.000 | 0.000 | 1.000 | 0.000 | 1.000 |
| 1.100 | 0.200 | 0.683 | 0.803 | 1.000 | 1.000 | 0.000 | 1.000 | 0.000 |
| 1.100 | 0.400 | 1.111 | 0.653 | 1.000 | 1.000 | 0.000 | 1.000 | 0.119 |
| 1.100 | 0.600 | 1.393 | 0.546 | 0.965 | 1.000 | 0.000 | 1.000 | 3.317 |
| 1.100 | 0.800 | 1.595 | 0.469 | 0.706 | 1.000 | 0.723 | 1.000 | 2.069 |
| 1.100 | 0.900 | 1.720 | 0.449 | 0.480 | 1.000 | 1.000 | 1.000 | 1.119 |
| 1.100 | 1.000 | 1.823 | 0.429 | 0.257 | 1.000 | 1.000 | 1.050 | 1.010 |
| 1.100 | 1.100 | 1.919 | 0.410 | 0.104 | 0.743 | 1.000 | 1.149 | 1.000 |
| 1.100 | 1.200 | 1.948 | 0.382 | 0.026 | 0.069 | 1.000 | 1.644 | 1.000 |
| 1.100 | 1.400 | 2.232 | 0.375 | 0.000 | 0.000 | 1.000 | 0.109 | 1.000 |
| 1.100 | 1.600 | 2.711 | 0.398 | 0.000 | 0.000 | 1.000 | 0.000 | 1.000 |
| 1.100 | 1.800 | 3.447 | 0.450 | 0.000 | 0.000 | 1.000 | 0.000 | 1.000 |
| 1.100 | 2.000 | 4.462 | 0.524 | 0.000 | 0.000 | 1.000 | 0.000 | 1.000 |
| 1.200 | 0.200 | 0.801 | 0.863 | 1.000 | 1.000 | 0.000 | 1.000 | 0.000 |
| 1.200 | 0.400 | 1.369 | 0.737 | 1.000 | 1.000 | 0.000 | 1.000 | 0.040 |
| 1.200 | 0.600 | 1.819 | 0.653 | 0.984 | 1.000 | 0.000 | 1.000 | 2.386 |
| 1.200 | 0.800 | 2.214 | 0.596 | 0.781 | 1.000 | 0.386 | 1.000 | 2.752 |
| 1.200 | 0.900 | 2.330 | 0.558 | 0.534 | 1.000 | 1.000 | 1.000 | 1.267 |
| 1.200 | 1.000 | 2.593 | 0.559 | 0.265 | 1.000 | 1.000 | 1.040 | 1.040 |
| 1.200 | 1.100 | 2.843 | 0.557 | 0.089 | 0.436 | 1.000 | 1.416 | 1.000 |
| 1.200 | 1.200 | 3.020 | 0.542 | 0.016 | 0.020 | 1.000 | 1.604 | 1.000 |
| 1.200 | 1.400 | 3.434 | 0.529 | 0.000 | 0.000 | 1.000 | 0.050 | 1.000 |
| 1.200 | 1.600 | 4.452 | 0.600 | 0.000 | 0.000 | 1.000 | 0.000 | 1.000 |
| 1.200 | 1.800 | 5.278 | 0.632 | 0.000 | 0.000 | 1.000 | 0.000 | 1.000 |
| 1.200 | 2.000 | 7.059 | 0.761 | 0.000 | 0.000 | 1.000 | 0.000 | 1.000 |
| 1.300 | 0.200 | 0.895 | 0.890 | 1.000 | 1.000 | 0.000 | 1.000 | 0.000 |
| 1.300 | 0.400 | 1.597 | 0.794 | 1.000 | 1.000 | 0.000 | 1.000 | 0.010 |
| 1.300 | 0.600 | 2.206 | 0.731 | 0.995 | 1.000 | 0.000 | 1.000 | 1.307 |
| 1.300 | 0.800 | 2.804 | 0.697 | 0.827 | 1.000 | 0.248 | 1.000 | 3.287 |
| 1.300 | 0.900 | 3.071 | 0.679 | 0.571 | 1.000 | 1.000 | 1.000 | 1.297 |
| 1.300 | 1.000 | 3.426 | 0.681 | 0.277 | 1.000 | 1.000 | 1.030 | 1.010 |
| 1.300 | 1.100 | 3.636 | 0.657 | 0.079 | 0.446 | 1.000 | 1.703 | 1.000 |
| 1.300 | 1.200 | 4.031 | 0.668 | 0.013 | 0.010 | 1.000 | 1.436 | 1.000 |
| 1.300 | 1.400 | 4.850 | 0.689 | 0.000 | 0.000 | 1.000 | 0.020 | 1.000 |
| 1.300 | 1.600 | 5.754 | 0.715 | 0.000 | 0.000 | 1.000 | 0.000 | 1.000 |
| 1.300 | 1.800 | 7.364 | 0.814 | 0.000 | 0.000 | 1.000 | 0.000 | 1.000 |
| 1.300 | 2.000 | 9.376 | 0.932 | 0.000 | 0.000 | 1.000 | 0.000 | 1.000 |
| 1.400 | 0.200 | 0.989 | 0.913 | 1.000 | 1.000 | 0.000 | 1.000 | 0.000 |
| 1.400 | 0.400 | 1.843 | 0.851 | 1.000 | 1.000 | 0.000 | 1.000 | 0.010 |
| 1.400 | 0.600 | 2.615 | 0.805 | 0.997 | 1.000 | 0.000 | 1.000 | 0.861 |
| 1.400 | 0.800 | 3.341 | 0.771 | 0.863 | 1.000 | 0.079 | 1.000 | 3.970 |
| 1.400 | 0.900 | 3.759 | 0.771 | 0.606 | 1.000 | 0.990 | 1.000 | 1.376 |
| 1.400 | 1.000 | 4.165 | 0.769 | 0.277 | 1.000 | 1.000 | 1.020 | 1.010 |
| 1.400 | 1.100 | 4.560 | 0.766 | 0.073 | 0.356 | 1.000 | 1.723 | 1.000 |
| 1.400 | 1.200 | 4.973 | 0.765 | 0.009 | 0.010 | 1.000 | 1.317 | 1.000 |
| 1.400 | 1.400 | 6.079 | 0.802 | 0.000 | 0.000 | 1.000 | 0.000 | 1.000 |
| 1.400 | 1.600 | 7.494 | 0.865 | 0.000 | 0.000 | 1.000 | 0.000 | 1.000 |
| 1.400 | 1.800 | 9.438 | 0.968 | 0.000 | 0.000 | 1.000 | 0.000 | 1.000 |
| 1.400 | 2.000 | 11.932 | 1.102 | 0.000 | 0.000 | 1.000 | 0.000 | 1.000 |
| 1.600 | 0.200 | 1.179 | 0.953 | 1.000 | 1.000 | 0.000 | 1.000 | 0.000 |
| 1.600 | 0.400 | 2.301 | 0.930 | 1.000 | 1.000 | 0.000 | 1.000 | 0.000 |

*Continued on next page*

TABLE s25 – Thermodynamic and structural properties of methanol (continued)

| $T/T_c$ | $\rho/\rho_c$ | $p/p_c$ | $z$ | $\Pi_{gas}$ | $p_{inf}^{gas}$ | $p_{inf}^{liq}$ | $\langle n_c^{gas}\rangle$ | $\langle n_c^{liq}\rangle$ |
|---|---|---|---|---|---|---|---|---|
| 1.600 | 0.600 | 3.319 | 0.894 | 0.999 | 1.000 | 0.000 | 1.000 | 0.436 |
| 1.600 | 0.800 | 4.430 | 0.895 | 0.896 | 1.000 | 0.059 | 1.000 | 4.475 |
| 1.600 | 0.900 | 4.978 | 0.894 | 0.649 | 1.000 | 0.950 | 1.000 | 1.525 |
| 1.600 | 1.000 | 5.601 | 0.905 | 0.292 | 1.000 | 1.000 | 1.030 | 1.000 |
| 1.600 | 1.100 | 6.360 | 0.934 | 0.067 | 0.317 | 1.000 | 1.752 | 1.000 |
| 1.600 | 1.200 | 6.911 | 0.931 | 0.005 | 0.000 | 1.000 | 0.960 | 1.000 |
| 1.600 | 1.400 | 8.403 | 0.970 | 0.000 | 0.000 | 1.000 | 0.000 | 1.000 |
| 1.600 | 1.600 | 10.485 | 1.059 | 0.000 | 0.000 | 1.000 | 0.000 | 1.000 |
| 1.600 | 1.800 | 13.307 | 1.195 | 0.000 | 0.000 | 1.000 | 0.000 | 1.000 |
| 1.600 | 2.000 | 16.696 | 1.349 | 0.000 | 0.000 | 1.000 | 0.000 | 1.000 |
| 1.900 | 0.200 | 1.449 | 0.986 | 1.000 | 1.000 | 0.000 | 1.000 | 0.000 |
| 1.900 | 0.400 | 2.878 | 0.979 | 1.000 | 1.000 | 0.000 | 1.000 | 0.000 |
| 1.900 | 0.600 | 4.435 | 1.006 | 0.999 | 1.000 | 0.000 | 1.000 | 0.228 |
| 1.900 | 0.800 | 5.926 | 1.008 | 0.923 | 1.000 | 0.020 | 1.000 | 4.059 |
| 1.900 | 0.900 | 6.805 | 1.029 | 0.685 | 1.000 | 0.881 | 1.000 | 1.693 |
| 1.900 | 1.000 | 7.785 | 1.059 | 0.298 | 1.000 | 1.000 | 1.030 | 1.020 |
| 1.900 | 1.100 | 8.710 | 1.078 | 0.054 | 0.168 | 1.000 | 2.168 | 1.000 |
| 1.900 | 1.200 | 9.797 | 1.111 | 0.003 | 0.000 | 1.000 | 0.752 | 1.000 |
| 1.900 | 1.400 | 12.324 | 1.198 | 0.000 | 0.000 | 1.000 | 0.000 | 1.000 |
| 1.900 | 1.600 | 15.477 | 1.316 | 0.000 | 0.000 | 1.000 | 0.000 | 1.000 |
| 1.900 | 1.800 | 18.800 | 1.421 | 0.000 | 0.000 | 1.000 | 0.000 | 1.000 |
| 1.900 | 2.000 | 23.749 | 1.616 | 0.000 | 0.000 | 1.000 | 0.000 | 1.000 |
| 2.300 | 0.200 | 1.799 | 1.011 | 1.000 | 1.000 | 0.000 | 1.000 | 0.000 |
| 2.300 | 0.400 | 3.671 | 1.032 | 1.000 | 1.000 | 0.000 | 1.000 | 0.000 |
| 2.300 | 0.600 | 5.707 | 1.069 | 1.000 | 1.000 | 0.000 | 1.000 | 0.109 |
| 2.300 | 0.800 | 7.893 | 1.109 | 0.945 | 1.000 | 0.010 | 1.000 | 4.248 |
| 2.300 | 0.900 | 9.131 | 1.141 | 0.711 | 1.000 | 0.861 | 1.000 | 1.891 |
| 2.300 | 1.000 | 10.437 | 1.173 | 0.302 | 1.000 | 1.000 | 1.020 | 1.010 |
| 2.300 | 1.100 | 11.956 | 1.222 | 0.046 | 0.089 | 1.000 | 2.248 | 1.000 |
| 2.300 | 1.200 | 13.420 | 1.257 | 0.002 | 0.000 | 1.000 | 0.644 | 1.000 |
| 2.300 | 1.400 | 16.838 | 1.352 | 0.000 | 0.000 | 1.000 | 0.000 | 1.000 |
| 2.300 | 1.600 | 21.078 | 1.481 | 0.000 | 0.000 | 1.000 | 0.000 | 1.000 |
| 2.300 | 1.800 | 26.165 | 1.634 | 0.000 | 0.000 | 1.000 | 0.000 | 1.000 |
| 2.300 | 2.000 | 32.349 | 1.818 | 0.000 | 0.000 | 1.000 | 0.000 | 1.000 |
| 2.700 | 0.200 | 2.147 | 1.028 | 1.000 | 1.000 | 0.000 | 1.000 | 0.000 |
| 2.700 | 0.400 | 4.451 | 1.066 | 1.000 | 1.000 | 0.000 | 1.000 | 0.000 |
| 2.700 | 0.600 | 6.983 | 1.115 | 1.000 | 1.000 | 0.000 | 1.000 | 0.099 |
| 2.700 | 0.800 | 9.889 | 1.184 | 0.952 | 1.000 | 0.000 | 1.000 | 4.297 |
| 2.700 | 0.900 | 11.414 | 1.215 | 0.721 | 1.000 | 0.842 | 1.000 | 2.020 |
| 2.700 | 1.000 | 12.914 | 1.237 | 0.306 | 1.000 | 1.000 | 1.010 | 1.000 |
| 2.700 | 1.100 | 14.966 | 1.303 | 0.045 | 0.069 | 1.000 | 2.188 | 1.000 |
| 2.700 | 1.200 | 16.851 | 1.345 | 0.002 | 0.000 | 1.000 | 0.663 | 1.000 |
| 2.700 | 1.400 | 21.254 | 1.454 | 0.000 | 0.000 | 1.000 | 0.000 | 1.000 |
| 2.700 | 1.600 | 26.631 | 1.594 | 0.000 | 0.000 | 1.000 | 0.000 | 1.000 |
| 2.700 | 1.800 | 33.186 | 1.766 | 0.000 | 0.000 | 1.000 | 0.000 | 1.000 |
| 2.700 | 2.000 | 41.596 | 1.992 | 0.000 | 0.000 | 1.000 | 0.000 | 1.000 |
| 3.000 | 0.200 | 2.419 | 1.042 | 1.000 | 1.000 | 0.000 | 1.000 | 0.000 |
| 3.000 | 0.400 | 5.008 | 1.079 | 1.000 | 1.000 | 0.000 | 1.000 | 0.000 |
| 3.000 | 0.600 | 7.913 | 1.137 | 1.000 | 1.000 | 0.000 | 1.000 | 0.020 |
| 3.000 | 0.800 | 11.184 | 1.205 | 0.956 | 1.000 | 0.000 | 1.000 | 4.079 |
| 3.000 | 0.900 | 13.036 | 1.248 | 0.736 | 1.000 | 0.822 | 1.000 | 2.218 |
| 3.000 | 1.000 | 14.862 | 1.281 | 0.304 | 1.000 | 1.000 | 1.059 | 1.020 |
| 3.000 | 1.100 | 17.052 | 1.336 | 0.040 | 0.040 | 1.000 | 2.248 | 1.000 |
| 3.000 | 1.200 | 19.348 | 1.390 | 0.001 | 0.000 | 1.000 | 0.505 | 1.000 |
| 3.000 | 1.400 | 24.548 | 1.511 | 0.000 | 0.000 | 1.000 | 0.000 | 1.000 |
| 3.000 | 1.600 | 30.723 | 1.655 | 0.000 | 0.000 | 1.000 | 0.000 | 1.000 |
| 3.000 | 1.800 | 38.387 | 1.838 | 0.000 | 0.000 | 1.000 | 0.000 | 1.000 |
| 3.000 | 2.000 | 47.647 | 2.053 | 0.000 | 0.000 | 1.000 | 0.000 | 1.000 |
| 3.500 | 0.200 | 3.479 | 1.285 | 1.000 | 1.000 | 0.000 | 1.000 | 0.000 |
| 3.500 | 0.400 | 7.244 | 1.338 | 1.000 | 1.000 | 0.000 | 1.000 | 0.000 |
| 3.500 | 0.600 | 11.388 | 1.402 | 1.000 | 1.000 | 0.000 | 1.000 | 0.059 |

*Continued on next page*

TABLE s25 – Thermodynamic and structural properties of methanol (continued)

| $T/T_c$ | $\rho/\rho_c$ | $p/p_c$ | $z$ | $\Pi_{gas}$ | $p^{gas}_{inf}$ | $p^{liq}_{inf}$ | $\langle n^{gas}_c \rangle$ | $\langle n^{liq}_c \rangle$ |
|---|---|---|---|---|---|---|---|---|
| 3.500 | 0.800 | 15.998 | 1.477 | 0.953 | 1.000 | 0.000 | 1.000 | 3.515 |
| 3.500 | 0.900 | 18.513 | 1.520 | 0.744 | 1.000 | 0.772 | 1.000 | 1.970 |
| 3.500 | 1.000 | 21.169 | 1.564 | 0.305 | 1.000 | 1.000 | 1.040 | 1.040 |
| 3.500 | 1.100 | 24.015 | 1.613 | 0.042 | 0.069 | 1.000 | 2.396 | 1.000 |
| 3.500 | 1.200 | 27.047 | 1.665 | 0.000 | 0.000 | 1.000 | 0.317 | 1.000 |
| 3.500 | 1.400 | 33.781 | 1.783 | 0.000 | 0.000 | 1.000 | 0.000 | 1.000 |
| 3.500 | 1.600 | 41.510 | 1.917 | 0.000 | 0.000 | 1.000 | 0.000 | 1.000 |
| 3.500 | 1.800 | 50.302 | 2.065 | 0.000 | 0.000 | 1.000 | 0.000 | 1.000 |
| 3.500 | 2.000 | 60.328 | 2.228 | 0.000 | 0.000 | 1.000 | 0.000 | 1.000 |

TABLE s26: Thermodynamic and structural properties of water

| $T/T_c$ | $\rho/\rho_c$ | $p/p_c$ | $z$ | $\Pi_{gas}$ | $p^{gas}_{inf}$ | $p^{liq}_{inf}$ | $\langle n^{gas}_c \rangle$ | $\langle n^{liq}_c \rangle$ |
|---|---|---|---|---|---|---|---|---|
| 1.000 | 0.500 | 0.914 | 0.381 | 0.925 | 1.000 | 0.000 | 1.000 | 3.951 |
| 1.000 | 0.600 | 0.947 | 0.329 | 0.815 | 1.000 | 0.020 | 1.000 | 3.495 |
| 1.000 | 0.700 | 0.969 | 0.288 | 0.659 | 1.000 | 0.416 | 1.000 | 2.089 |
| 1.000 | 0.800 | 0.988 | 0.257 | 0.501 | 1.000 | 0.871 | 1.000 | 1.317 |
| 1.000 | 0.900 | 1.003 | 0.232 | 0.350 | 1.000 | 1.000 | 1.000 | 1.109 |
| 1.000 | 1.000 | 1.000 | 0.208 | 0.217 | 1.000 | 1.000 | 1.020 | 1.040 |
| 1.000 | 1.100 | 0.996 | 0.189 | 0.120 | 0.901 | 1.000 | 1.099 | 1.000 |
| 1.000 | 1.200 | 1.013 | 0.176 | 0.051 | 0.317 | 1.000 | 1.307 | 1.000 |
| 1.000 | 1.300 | 1.012 | 0.162 | 0.018 | 0.069 | 1.000 | 1.287 | 1.000 |
| 1.000 | 1.400 | 1.037 | 0.154 | 0.004 | 0.000 | 1.000 | 0.752 | 1.000 |
| 1.000 | 1.500 | 1.076 | 0.149 | 0.001 | 0.000 | 1.000 | 0.267 | 1.000 |
| 1.010 | 0.500 | 0.000 | 0.000 | 0.938 | 1.000 | 0.000 | 1.000 | 3.931 |
| 1.010 | 0.600 | 0.959 | 0.330 | 0.825 | 1.000 | 0.010 | 1.000 | 3.525 |
| 1.010 | 0.700 | 1.004 | 0.296 | 0.685 | 1.000 | 0.238 | 1.000 | 2.327 |
| 1.010 | 0.800 | 1.031 | 0.266 | 0.515 | 1.000 | 0.851 | 1.000 | 1.426 |
| 1.010 | 0.900 | 1.051 | 0.241 | 0.359 | 1.000 | 1.000 | 1.000 | 1.050 |
| 1.010 | 1.000 | 1.073 | 0.221 | 0.219 | 1.000 | 1.000 | 1.010 | 1.010 |
| 1.010 | 1.100 | 1.081 | 0.203 | 0.115 | 0.891 | 1.000 | 1.099 | 1.000 |
| 1.010 | 1.200 | 1.097 | 0.188 | 0.050 | 0.317 | 1.000 | 1.297 | 1.000 |
| 1.010 | 1.300 | 1.116 | 0.177 | 0.015 | 0.050 | 1.000 | 1.337 | 1.000 |
| 1.010 | 1.400 | 1.123 | 0.165 | 0.004 | 0.000 | 1.000 | 0.802 | 1.000 |
| 1.010 | 1.500 | 1.167 | 0.161 | 0.001 | 0.000 | 1.000 | 0.218 | 1.000 |
| 1.050 | 0.200 | 0.692 | 0.686 | 1.000 | 1.000 | 0.000 | 1.000 | 0.000 |
| 1.050 | 0.400 | 1.028 | 0.510 | 0.993 | 1.000 | 0.000 | 1.000 | 1.040 |
| 1.050 | 0.600 | 1.212 | 0.401 | 0.890 | 1.000 | 0.010 | 1.000 | 4.020 |
| 1.050 | 0.800 | 1.326 | 0.329 | 0.581 | 1.000 | 0.960 | 1.000 | 1.406 |
| 1.050 | 0.900 | 1.382 | 0.305 | 0.394 | 1.000 | 1.000 | 1.010 | 1.079 |
| 1.050 | 1.000 | 1.427 | 0.283 | 0.229 | 1.000 | 1.000 | 1.050 | 1.000 |
| 1.050 | 1.100 | 1.476 | 0.266 | 0.104 | 0.743 | 1.000 | 1.149 | 1.000 |
| 1.050 | 1.200 | 1.529 | 0.253 | 0.040 | 0.158 | 1.000 | 1.406 | 1.000 |
| 1.050 | 1.400 | 1.676 | 0.238 | 0.002 | 0.000 | 1.000 | 0.525 | 1.000 |
| 1.050 | 1.600 | 1.937 | 0.240 | 0.000 | 0.000 | 1.000 | 0.010 | 1.000 |
| 1.100 | 0.200 | 0.767 | 0.726 | 1.000 | 1.000 | 0.000 | 1.000 | 0.000 |
| 1.100 | 0.400 | 1.194 | 0.565 | 0.997 | 1.000 | 0.000 | 1.000 | 0.485 |
| 1.100 | 0.600 | 1.468 | 0.463 | 0.929 | 1.000 | 0.000 | 1.000 | 4.465 |
| 1.100 | 0.800 | 1.676 | 0.397 | 0.637 | 1.000 | 0.832 | 1.000 | 1.733 |
| 1.100 | 0.900 | 1.774 | 0.373 | 0.426 | 1.000 | 1.000 | 1.000 | 1.139 |
| 1.100 | 1.000 | 1.874 | 0.355 | 0.233 | 1.000 | 1.000 | 1.030 | 1.040 |
| 1.100 | 1.100 | 1.970 | 0.339 | 0.099 | 0.713 | 1.000 | 1.366 | 1.000 |
| 1.100 | 1.200 | 2.076 | 0.328 | 0.026 | 0.089 | 1.000 | 1.683 | 1.000 |
| 1.100 | 1.400 | 2.351 | 0.318 | 0.001 | 0.000 | 1.000 | 0.376 | 1.000 |
| 1.100 | 1.600 | 2.752 | 0.326 | 0.000 | 0.000 | 1.000 | 0.000 | 1.000 |
| 1.150 | 0.200 | 0.841 | 0.762 | 1.000 | 1.000 | 0.000 | 1.000 | 0.000 |
| 1.150 | 0.400 | 1.354 | 0.613 | 0.999 | 1.000 | 0.000 | 1.000 | 0.218 |
| 1.150 | 0.600 | 1.720 | 0.519 | 0.953 | 1.000 | 0.000 | 1.000 | 4.020 |
| 1.150 | 0.800 | 2.020 | 0.457 | 0.681 | 1.000 | 0.752 | 1.000 | 2.079 |
| 1.150 | 0.900 | 2.164 | 0.436 | 0.455 | 1.000 | 1.000 | 1.000 | 1.198 |

*Continued on next page*

TABLE s26 – Thermodynamic and structural properties of water (continued)

| $T/T_c$ | $\rho/\rho_c$ | $p/p_c$ | $z$ | $\Pi_{gas}$ | $p^{gas}_{inf}$ | $p^{liq}_{inf}$ | $\langle n^{gas}_c \rangle$ | $\langle n^{liq}_c \rangle$ |
|---|---|---|---|---|---|---|---|---|
| 1.150 | 1.000 | 2.312 | 0.419 | 0.239 | 1.000 | 1.000 | 1.030 | 1.059 |
| 1.150 | 1.100 | 2.468 | 0.406 | 0.088 | 0.554 | 1.000 | 1.436 | 1.000 |
| 1.150 | 1.200 | 2.632 | 0.397 | 0.024 | 0.059 | 1.000 | 1.594 | 1.000 |
| 1.150 | 1.400 | 3.052 | 0.395 | 0.000 | 0.000 | 1.000 | 0.198 | 1.000 |
| 1.150 | 1.600 | 3.599 | 0.407 | 0.000 | 0.000 | 1.000 | 0.000 | 1.000 |
| 1.200 | 0.200 | 0.909 | 0.789 | 1.000 | 1.000 | 0.000 | 1.000 | 0.000 |
| 1.200 | 0.400 | 1.511 | 0.656 | 1.000 | 1.000 | 0.000 | 1.000 | 0.109 |
| 1.200 | 0.600 | 1.966 | 0.569 | 0.967 | 1.000 | 0.000 | 1.000 | 3.515 |
| 1.200 | 0.800 | 2.364 | 0.513 | 0.723 | 1.000 | 0.663 | 1.000 | 2.356 |
| 1.200 | 0.900 | 2.559 | 0.494 | 0.476 | 1.000 | 1.000 | 1.000 | 1.168 |
| 1.200 | 1.000 | 2.761 | 0.479 | 0.245 | 1.000 | 1.000 | 1.059 | 1.010 |
| 1.200 | 1.100 | 2.973 | 0.469 | 0.089 | 0.594 | 1.000 | 1.485 | 1.000 |
| 1.200 | 1.200 | 3.208 | 0.464 | 0.019 | 0.030 | 1.000 | 1.644 | 1.000 |
| 1.200 | 1.400 | 3.749 | 0.465 | 0.000 | 0.000 | 1.000 | 0.109 | 1.000 |
| 1.200 | 1.600 | 4.465 | 0.484 | 0.000 | 0.000 | 1.000 | 0.000 | 1.000 |
| 1.250 | 0.200 | 0.976 | 0.813 | 1.000 | 1.000 | 0.000 | 1.000 | 0.000 |
| 1.250 | 0.400 | 1.663 | 0.693 | 1.000 | 1.000 | 0.000 | 1.000 | 0.099 |
| 1.250 | 0.600 | 2.213 | 0.615 | 0.977 | 1.000 | 0.000 | 1.000 | 2.881 |
| 1.250 | 0.800 | 2.715 | 0.566 | 0.756 | 1.000 | 0.515 | 1.000 | 2.683 |
| 1.250 | 0.900 | 2.955 | 0.547 | 0.506 | 1.000 | 1.000 | 1.000 | 1.267 |
| 1.250 | 1.000 | 3.211 | 0.535 | 0.251 | 1.000 | 1.000 | 1.050 | 1.000 |
| 1.250 | 1.100 | 3.480 | 0.527 | 0.084 | 0.495 | 1.000 | 1.396 | 1.000 |
| 1.250 | 1.200 | 3.772 | 0.524 | 0.018 | 0.050 | 1.000 | 1.554 | 1.000 |
| 1.250 | 1.400 | 4.452 | 0.530 | 0.000 | 0.000 | 1.000 | 0.040 | 1.000 |
| 1.250 | 1.600 | 5.347 | 0.557 | 0.000 | 0.000 | 1.000 | 0.000 | 1.000 |
| 1.300 | 0.200 | 1.038 | 0.832 | 1.000 | 1.000 | 0.000 | 1.000 | 0.000 |
| 1.300 | 0.400 | 1.813 | 0.726 | 1.000 | 1.000 | 0.000 | 1.000 | 0.050 |
| 1.300 | 0.600 | 2.455 | 0.656 | 0.984 | 1.000 | 0.000 | 1.000 | 2.317 |
| 1.300 | 0.800 | 3.052 | 0.611 | 0.772 | 1.000 | 0.426 | 1.000 | 3.050 |
| 1.300 | 0.900 | 3.351 | 0.597 | 0.517 | 1.000 | 1.000 | 1.000 | 1.386 |
| 1.300 | 1.000 | 3.663 | 0.587 | 0.256 | 1.000 | 1.000 | 1.040 | 1.010 |
| 1.300 | 1.100 | 3.992 | 0.582 | 0.075 | 0.366 | 1.000 | 1.594 | 1.000 |
| 1.300 | 1.200 | 4.348 | 0.581 | 0.016 | 0.020 | 1.000 | 1.743 | 1.000 |
| 1.300 | 1.400 | 5.168 | 0.592 | 0.000 | 0.000 | 1.000 | 0.030 | 1.000 |
| 1.300 | 1.600 | 6.213 | 0.622 | 0.000 | 0.000 | 1.000 | 0.000 | 1.000 |
| 1.600 | 0.200 | 1.408 | 0.917 | 1.000 | 1.000 | 0.000 | 1.000 | 0.000 |
| 1.600 | 0.400 | 2.649 | 0.862 | 1.000 | 1.000 | 0.000 | 1.000 | 0.000 |
| 1.600 | 0.600 | 3.832 | 0.832 | 0.999 | 1.000 | 0.000 | 1.000 | 1.030 |
| 1.600 | 0.800 | 5.031 | 0.819 | 0.901 | 1.000 | 0.089 | 1.000 | 4.119 |
| 1.600 | 0.900 | 5.654 | 0.818 | 0.648 | 1.000 | 1.000 | 1.000 | 1.515 |
| 1.600 | 1.000 | 6.308 | 0.821 | 0.280 | 1.000 | 1.000 | 1.089 | 1.040 |
| 1.600 | 1.100 | 7.006 | 0.829 | 0.056 | 0.248 | 1.000 | 1.743 | 1.000 |
| 1.600 | 1.200 | 7.744 | 0.840 | 0.004 | 0.000 | 1.000 | 1.248 | 1.000 |
| 1.600 | 1.400 | 9.441 | 0.878 | 0.000 | 0.000 | 1.000 | 0.000 | 1.000 |
| 1.600 | 1.600 | 11.482 | 0.934 | 0.000 | 0.000 | 1.000 | 0.000 | 1.000 |
| 2.000 | 0.200 | 1.865 | 0.971 | 1.000 | 1.000 | 0.000 | 1.000 | 0.000 |
| 2.000 | 0.400 | 3.692 | 0.961 | 1.000 | 1.000 | 0.000 | 1.000 | 0.000 |
| 2.000 | 0.600 | 5.545 | 0.963 | 1.000 | 1.000 | 0.000 | 1.000 | 0.287 |
| 2.000 | 0.800 | 7.515 | 0.978 | 0.926 | 1.000 | 0.050 | 1.000 | 4.465 |
| 2.000 | 0.900 | 8.571 | 0.992 | 0.681 | 1.000 | 0.990 | 1.000 | 1.574 |
| 2.000 | 1.000 | 9.683 | 1.009 | 0.287 | 1.000 | 1.000 | 1.020 | 1.059 |
| 2.000 | 1.100 | 10.853 | 1.028 | 0.048 | 0.129 | 1.000 | 1.921 | 1.000 |
| 2.000 | 1.200 | 12.112 | 1.051 | 0.003 | 0.000 | 1.000 | 0.990 | 1.000 |
| 2.000 | 1.400 | 14.966 | 1.113 | 0.000 | 0.000 | 1.000 | 0.000 | 1.000 |
| 2.000 | 1.600 | 18.266 | 1.189 | 0.000 | 0.000 | 1.000 | 0.000 | 1.000 |
| 2.500 | 0.200 | 2.408 | 1.003 | 1.000 | 1.000 | 0.000 | 1.000 | 0.000 |
| 2.500 | 0.400 | 4.915 | 1.024 | 1.000 | 1.000 | 0.000 | 1.000 | 0.000 |
| 2.500 | 0.600 | 7.562 | 1.050 | 1.000 | 1.000 | 0.000 | 1.000 | 0.188 |
| 2.500 | 0.800 | 10.464 | 1.090 | 0.932 | 1.000 | 0.020 | 1.000 | 4.446 |
| 2.500 | 0.900 | 12.019 | 1.113 | 0.695 | 1.000 | 0.941 | 1.000 | 1.812 |
| 2.500 | 1.000 | 13.683 | 1.140 | 0.282 | 1.000 | 1.000 | 1.079 | 1.000 |

*Continued on next page*

TABLE s26 – Thermodynamic and structural properties of water (continued)

| $T/T_c$ | $\rho/\rho_c$ | $p/p_c$ | $z$ | $\Pi_{gas}$ | $p^{gas}_{inf}$ | $p^{liq}_{inf}$ | $\langle n^{gas}_c \rangle$ | $\langle n^{liq}_c \rangle$ |
|---|---|---|---|---|---|---|---|---|
| 2.500 | 1.100 | 15.431 | 1.169 | 0.049 | 0.158 | 1.000 | 2.089 | 1.000 |
| 2.500 | 1.200 | 17.309 | 1.202 | 0.002 | 0.000 | 1.000 | 0.762 | 1.000 |
| 2.500 | 1.400 | 21.512 | 1.280 | 0.000 | 0.000 | 1.000 | 0.000 | 1.000 |
| 2.500 | 1.600 | 26.374 | 1.374 | 0.000 | 0.000 | 1.000 | 0.000 | 1.000 |
| 3.000 | 0.200 | 2.957 | 1.027 | 1.000 | 1.000 | 0.000 | 1.000 | 0.000 |
| 3.000 | 0.400 | 6.091 | 1.057 | 1.000 | 1.000 | 0.000 | 1.000 | 0.000 |
| 3.000 | 0.600 | 9.497 | 1.099 | 1.000 | 1.000 | 0.000 | 1.000 | 0.069 |
| 3.000 | 0.800 | 13.251 | 1.150 | 0.938 | 1.000 | 0.020 | 1.000 | 4.693 |
| 3.000 | 0.900 | 15.308 | 1.181 | 0.698 | 1.000 | 0.871 | 1.000 | 1.772 |
| 3.000 | 1.000 | 17.476 | 1.214 | 0.290 | 1.000 | 1.000 | 1.059 | 1.010 |
| 3.000 | 1.100 | 19.826 | 1.252 | 0.044 | 0.089 | 1.000 | 2.109 | 1.000 |
| 3.000 | 1.200 | 22.254 | 1.288 | 0.002 | 0.000 | 1.000 | 0.545 | 1.000 |
| 3.000 | 1.400 | 27.737 | 1.376 | 0.000 | 0.000 | 1.000 | 0.000 | 1.000 |
| 3.000 | 1.600 | 34.097 | 1.480 | 0.000 | 0.000 | 1.000 | 0.000 | 1.000 |
| 3.500 | 0.200 | 3.480 | 1.036 | 1.000 | 1.000 | 0.000 | 1.000 | 0.000 |
| 3.500 | 0.400 | 7.243 | 1.078 | 1.000 | 1.000 | 0.000 | 1.000 | 0.000 |
| 3.500 | 0.600 | 11.388 | 1.130 | 1.000 | 1.000 | 0.000 | 1.000 | 0.099 |
| 3.500 | 0.800 | 15.998 | 1.190 | 0.938 | 1.000 | 0.000 | 1.000 | 4.614 |
| 3.500 | 0.900 | 18.518 | 1.225 | 0.698 | 1.000 | 0.861 | 1.000 | 1.812 |
| 3.500 | 1.000 | 21.170 | 1.260 | 0.290 | 1.000 | 1.000 | 1.050 | 1.010 |
| 3.500 | 1.100 | 24.015 | 1.299 | 0.044 | 0.099 | 1.000 | 2.307 | 1.000 |
| 3.500 | 1.200 | 27.047 | 1.342 | 0.002 | 0.000 | 1.000 | 0.525 | 1.000 |
| 3.500 | 1.400 | 33.781 | 1.436 | 0.000 | 0.000 | 1.000 | 0.000 | 1.000 |
| 3.500 | 1.600 | 41.511 | 1.544 | 0.000 | 0.000 | 1.000 | 0.000 | 1.000 |
